# Supplementary material for: Reconstructing Video from Interferometric Measurements of Time-Varying Sources
Source: arXiv:1711.01357 source file (2018-02-01)
Supplement: Supplementary file 1 [file rotation_example_supp.tex]

\begin{figure*}
			\vspace{-0.9cm}
	\begin{center}
		\setlength{\tabcolsep}{1pt}
		%\hspace*{-1.5cm}
		\begin{tabular}{  c | c | c  c  c  c  c c }

			%\hline
			\multirow{1}{*}[0.85in]{ \rotatebox[origin=t]{90}{\large{\textsf{uv-coverage}} }} &
			\includegraphics[height=0.12\linewidth]{figures/uvcoverage/uv_ehtfuture2_rotation30_small.pdf} 
			&
			\includegraphics[height=0.12\linewidth]{figures/uvcoverage/ehtfuture2_30/uv_ehtfuture2_rotation30_0.pdf} &
			\includegraphics[height=0.12\linewidth]{figures/uvcoverage/ehtfuture2_30/uv_ehtfuture2_rotation30_6.pdf} &
			\includegraphics[height=0.12\linewidth]{figures/uvcoverage/ehtfuture2_30/uv_ehtfuture2_rotation30_12.pdf} &
			\includegraphics[height=0.12\linewidth]{figures/uvcoverage/ehtfuture2_30/uv_ehtfuture2_rotation30_18.pdf} &
			\includegraphics[height=0.12\linewidth]{figures/uvcoverage/ehtfuture2_30/uv_ehtfuture2_rotation30_24.pdf} &
			\includegraphics[height=0.12\linewidth]{figures/uvcoverage/ehtfuture2_30/uv_ehtfuture2_rotation30_29.pdf} 
			\\  \hline
			&\vspace{-.1in} &&&&&&\\

			&\large{\textsf{Mean Frame}}   &\large{\textsf{GST = 17:00}} &\large{\textsf{19:30}}    &\large{\textsf{22:00}} &\large{\textsf{00:30}}  &\large{\textsf{03:00}}  &\large{\textsf{05:30}}     \\ \hline
			
			&\vspace{-.1in} &&&&&&\\
			\multirow{1}{*}[.6in]{ \rotatebox[origin=t]{90}{\large{\textsf{Truth}} }}
			&
			{{\includegraphics[height=0.12\linewidth]{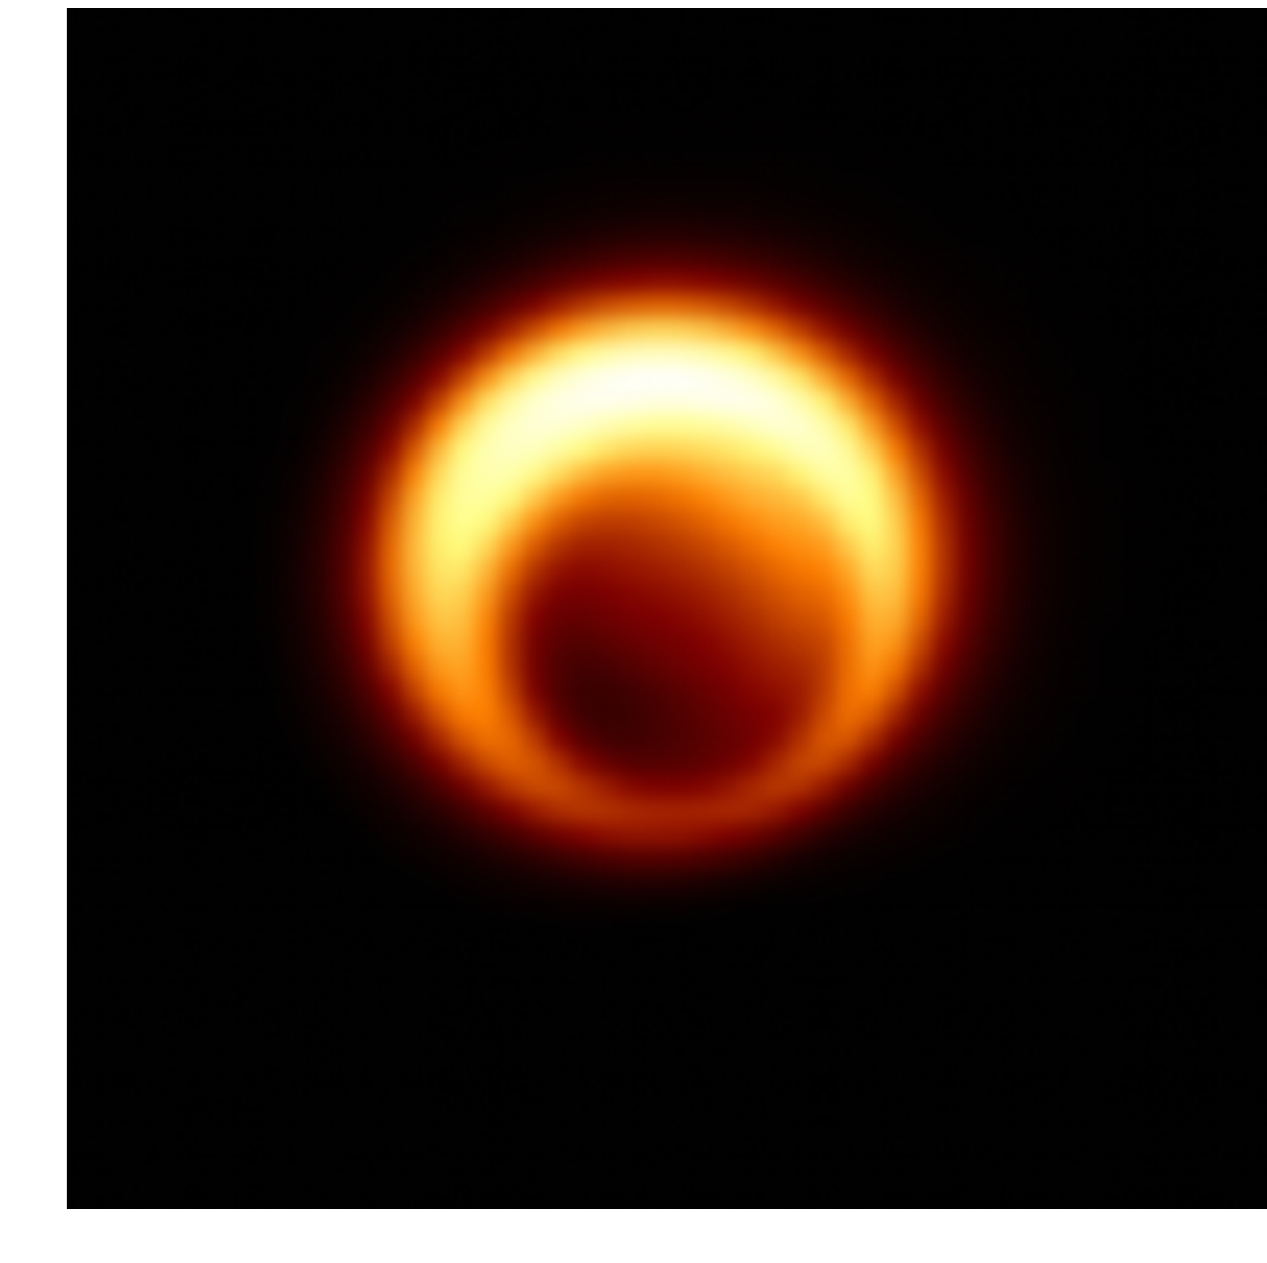}} } &
			\includegraphics[height=0.12\linewidth]{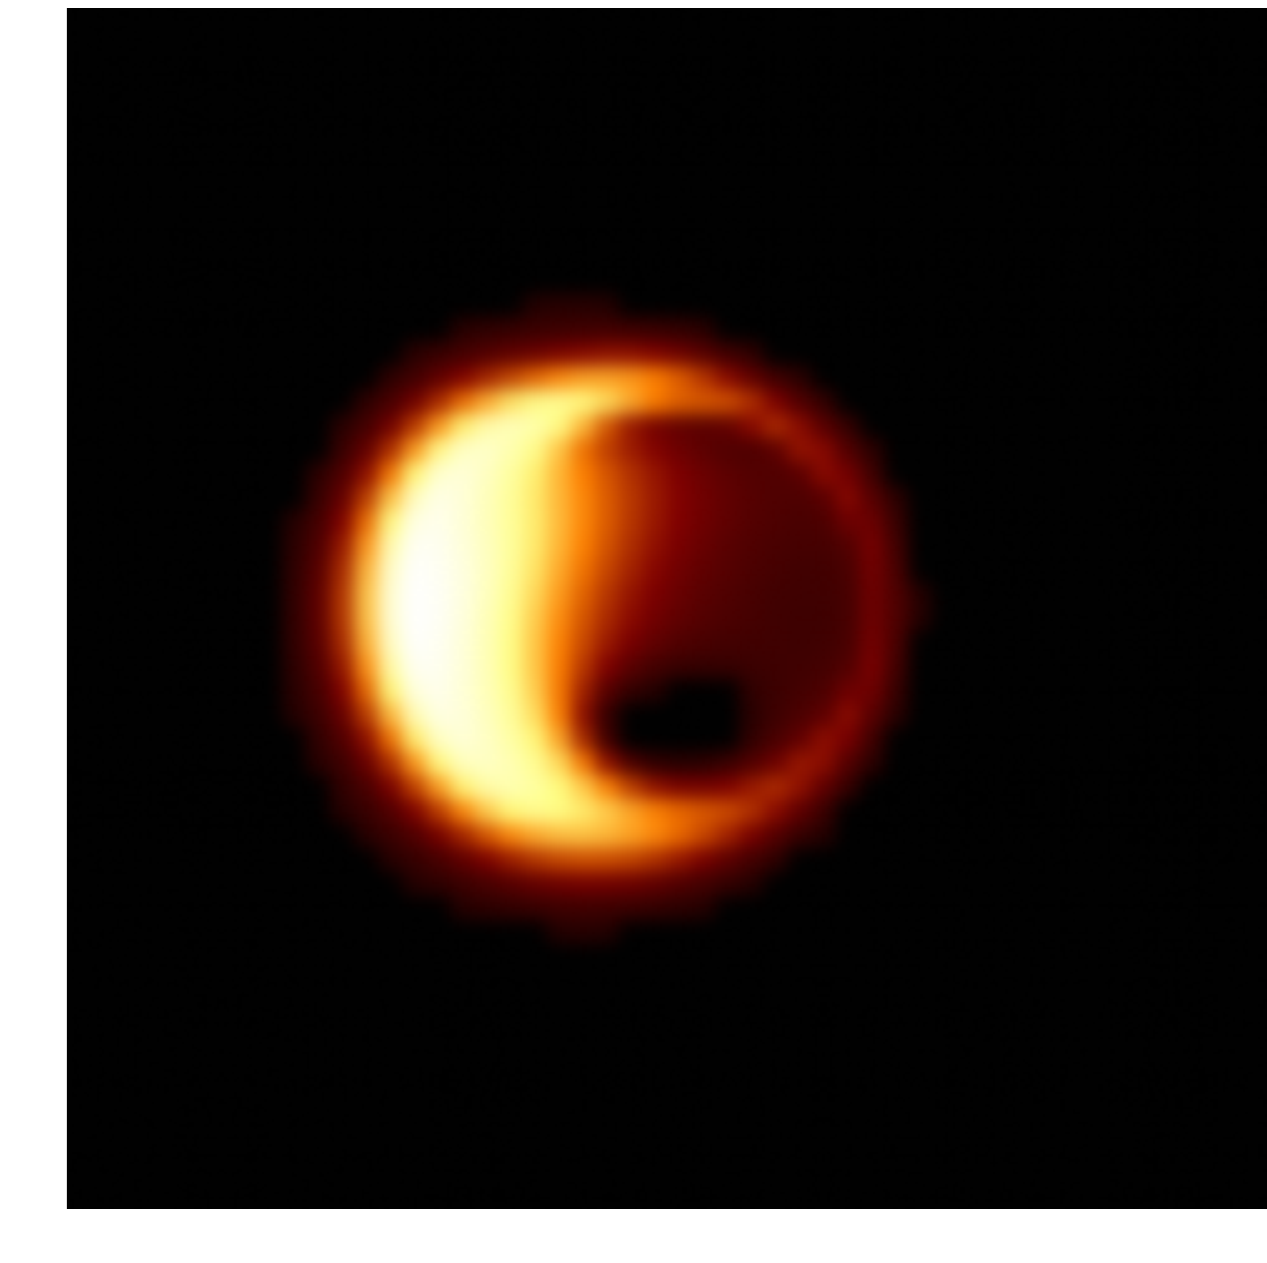} &
			\includegraphics[height=0.12\linewidth]{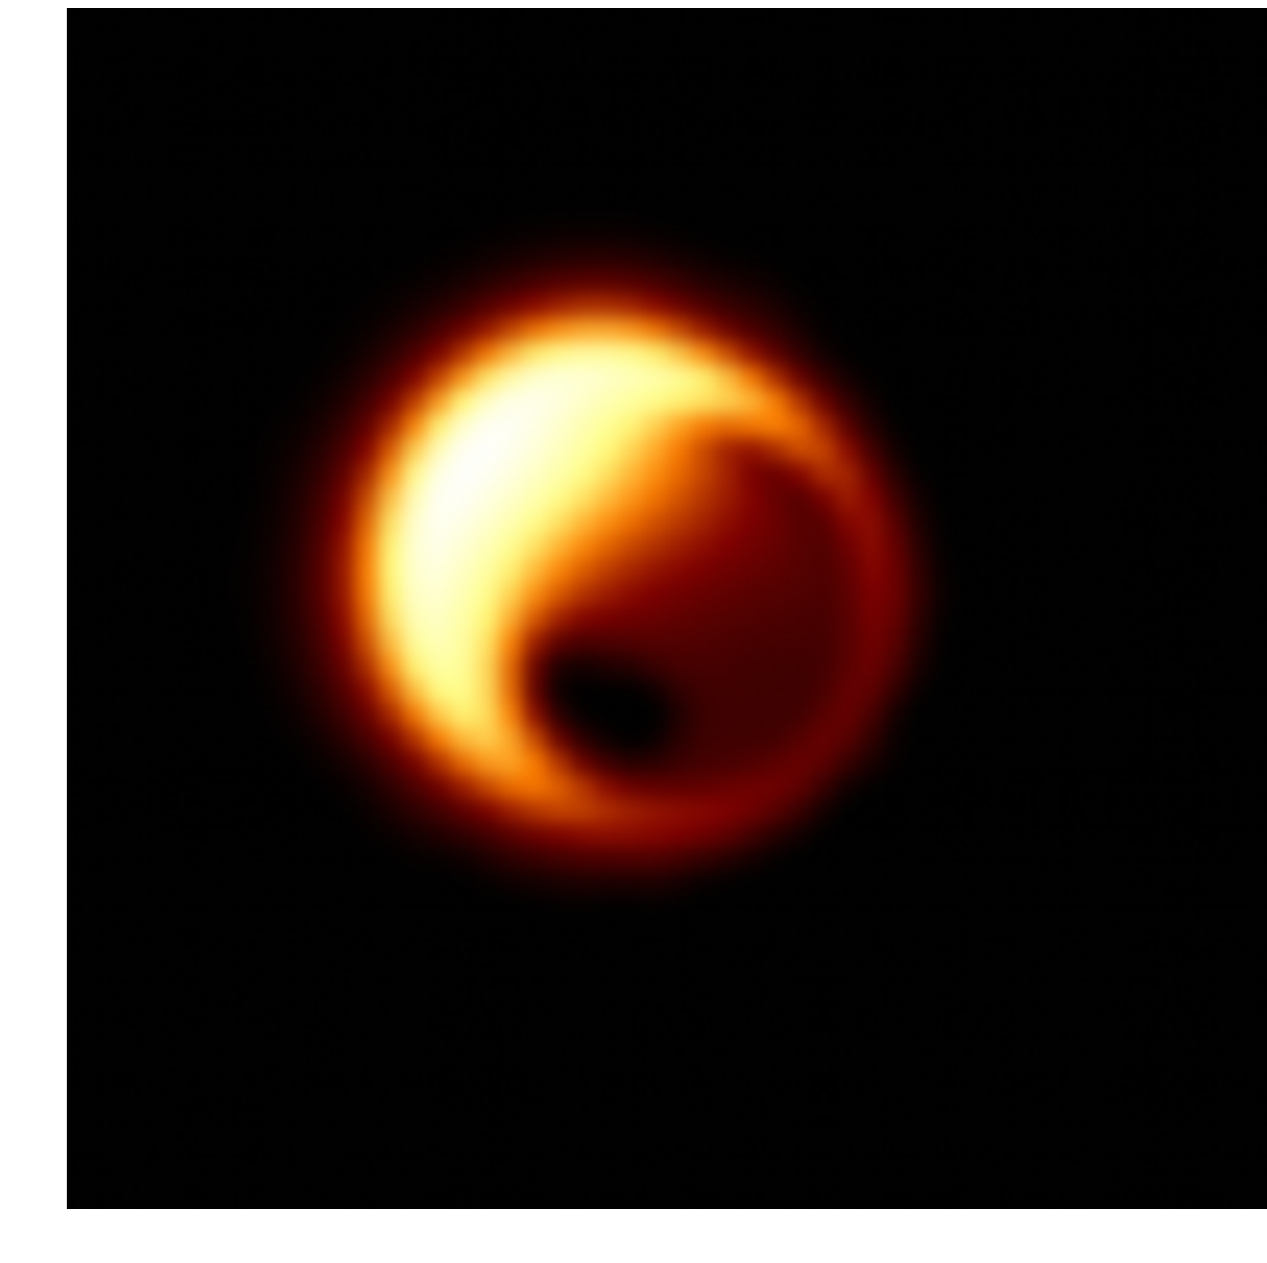} &
			\includegraphics[height=0.12\linewidth]{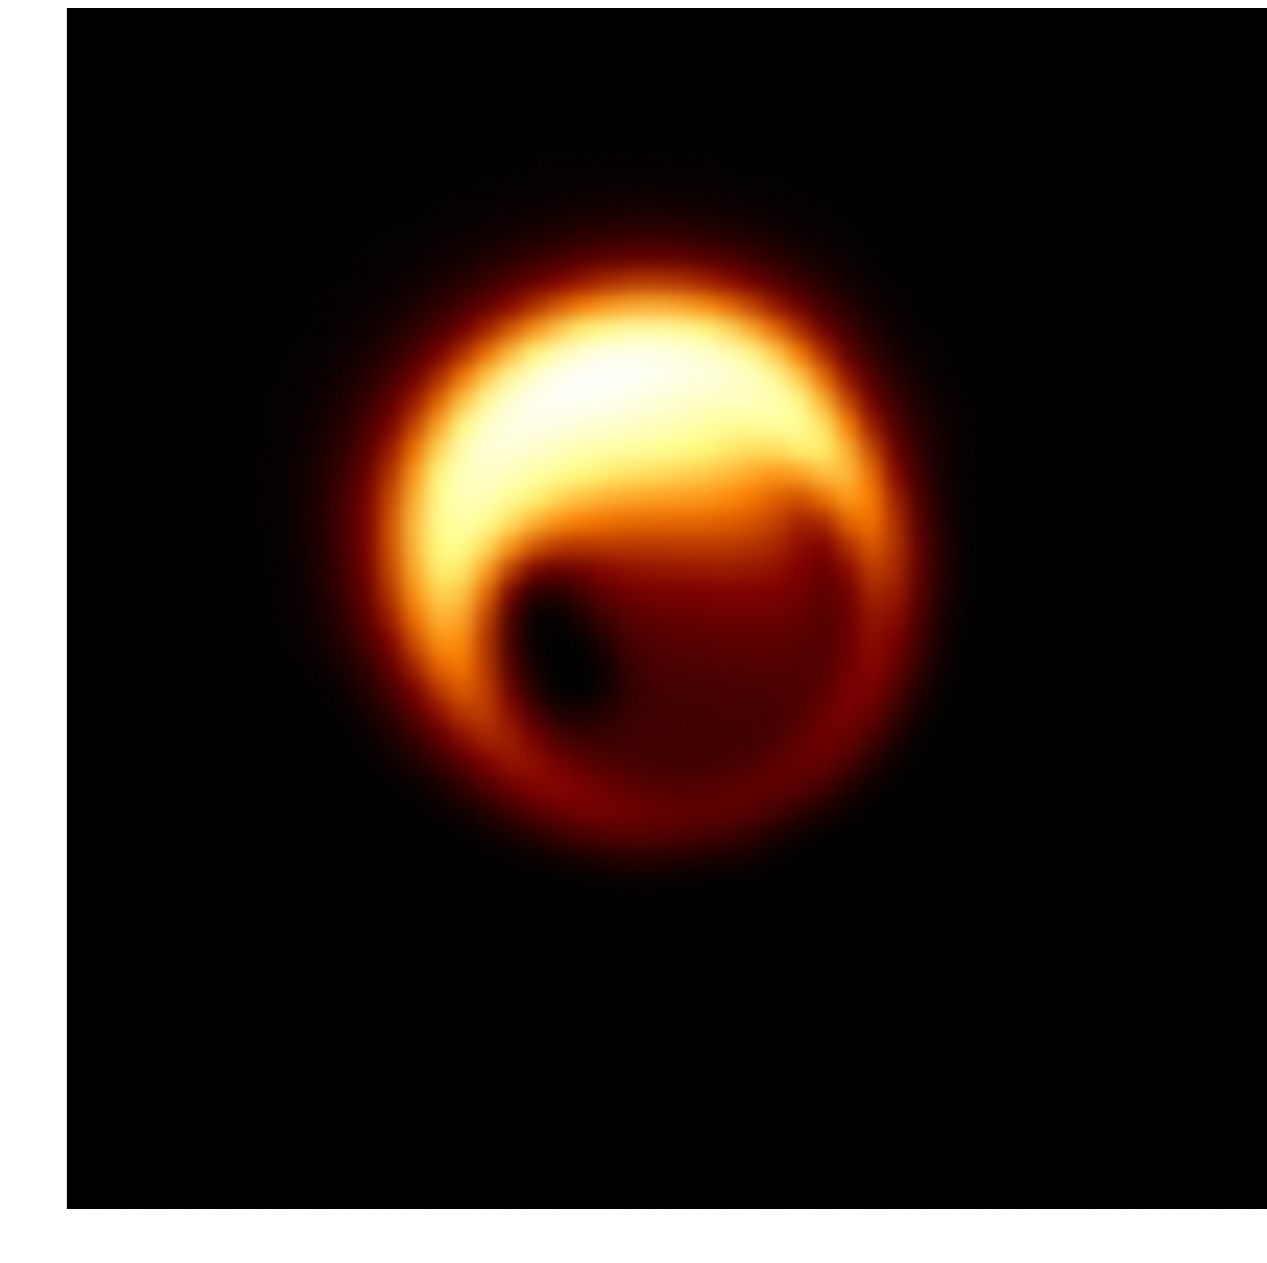} &
			\includegraphics[height=0.12\linewidth]{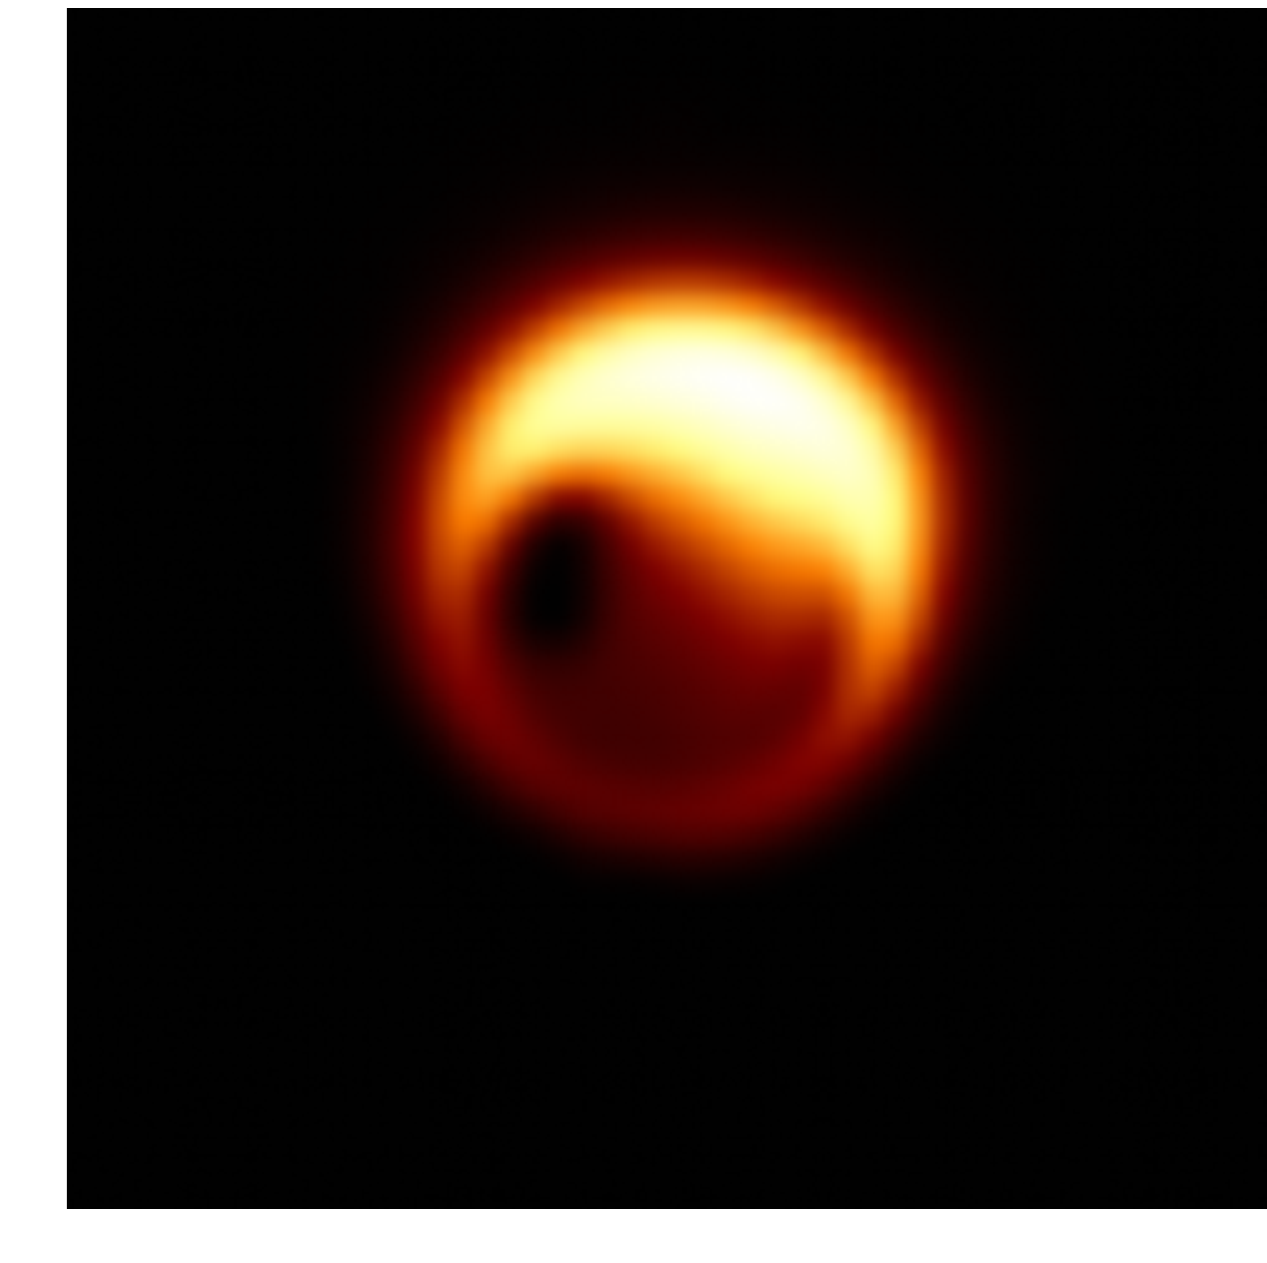} &
			\includegraphics[height=0.12\linewidth]{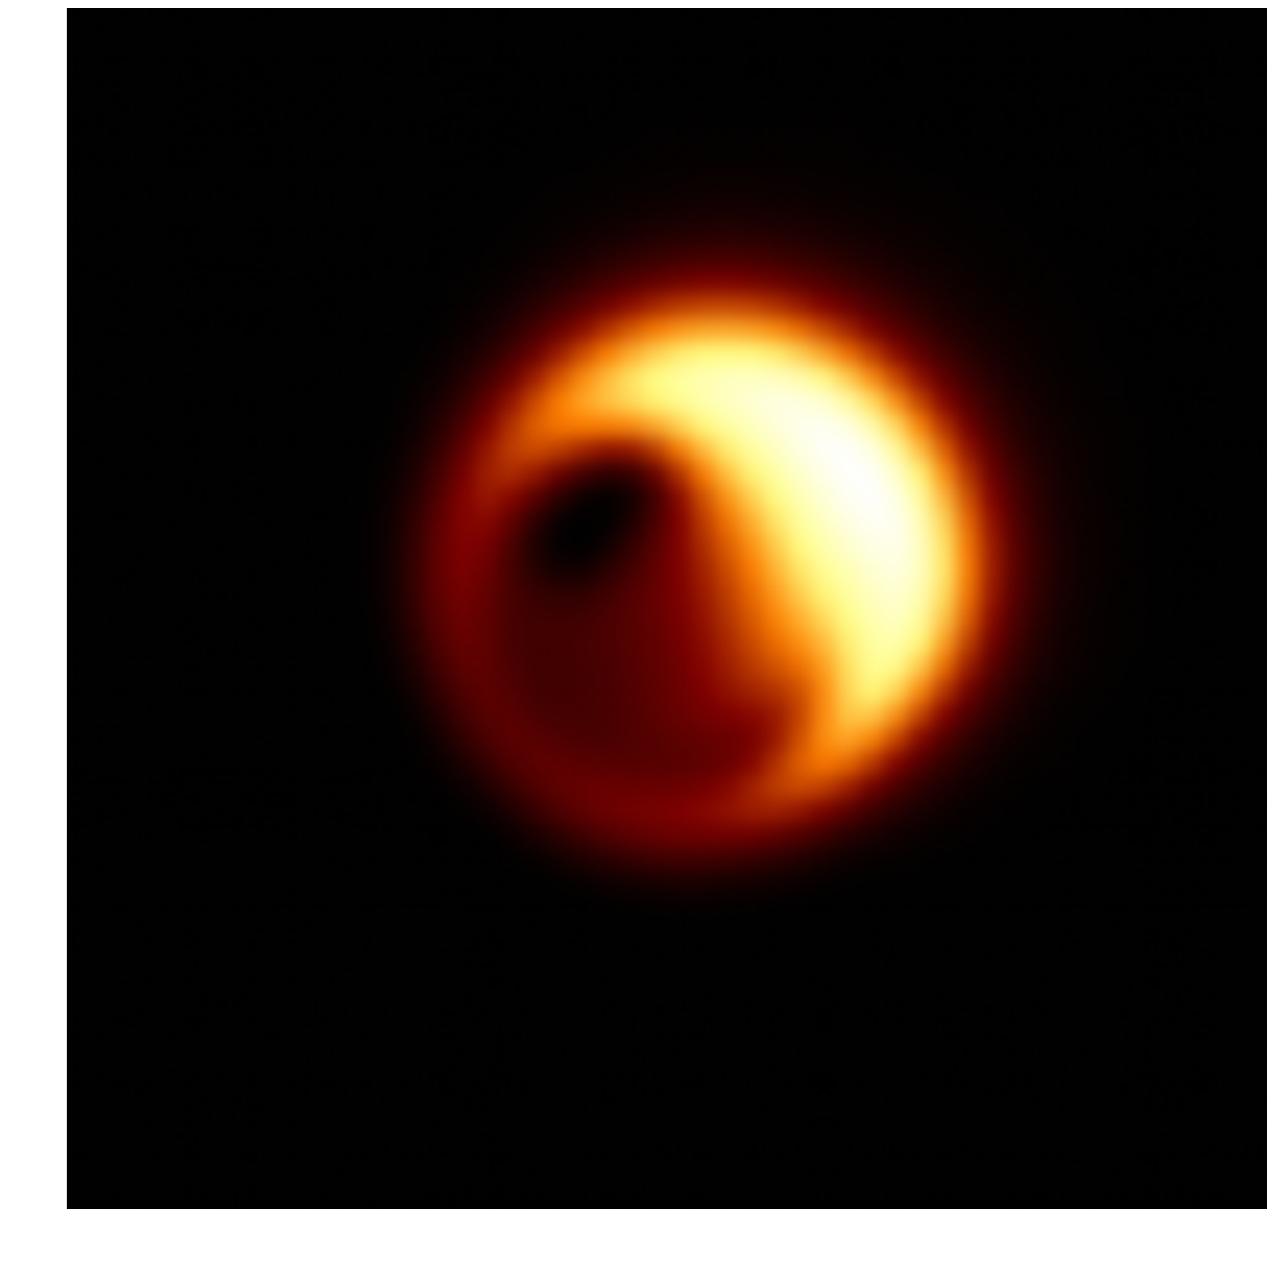} &
			\includegraphics[height=0.12\linewidth]{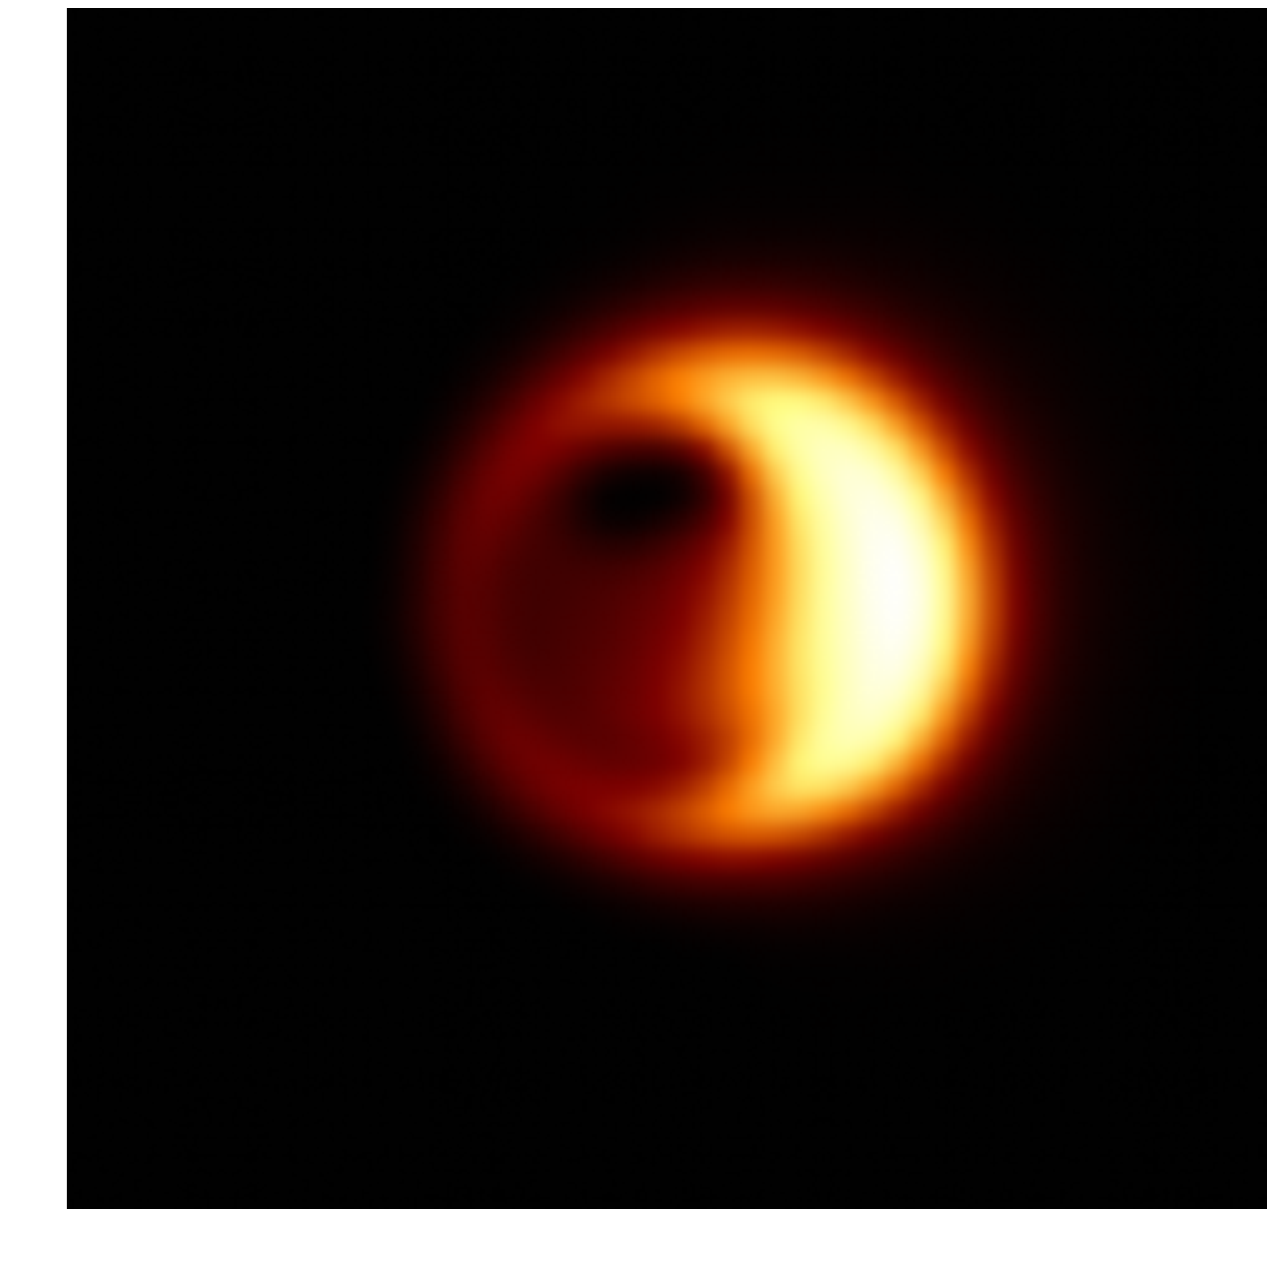} 
			\\   \hline
			&\vspace{-.1in} &&&&&&\\
			\multicolumn{8}{c}{  \large{\textsf{WITH NO ATMOSPHERIC PHASE ERROR }}  }
			\\ \hline
			&\vspace{-.1in} &&&&&&\\
			\multirow{1}{*}[.6in]{ \rotatebox[origin=t]{90}{\small{\textsf{Snapshot}} }}
			&
			{{\includegraphics[height=0.12\linewidth]{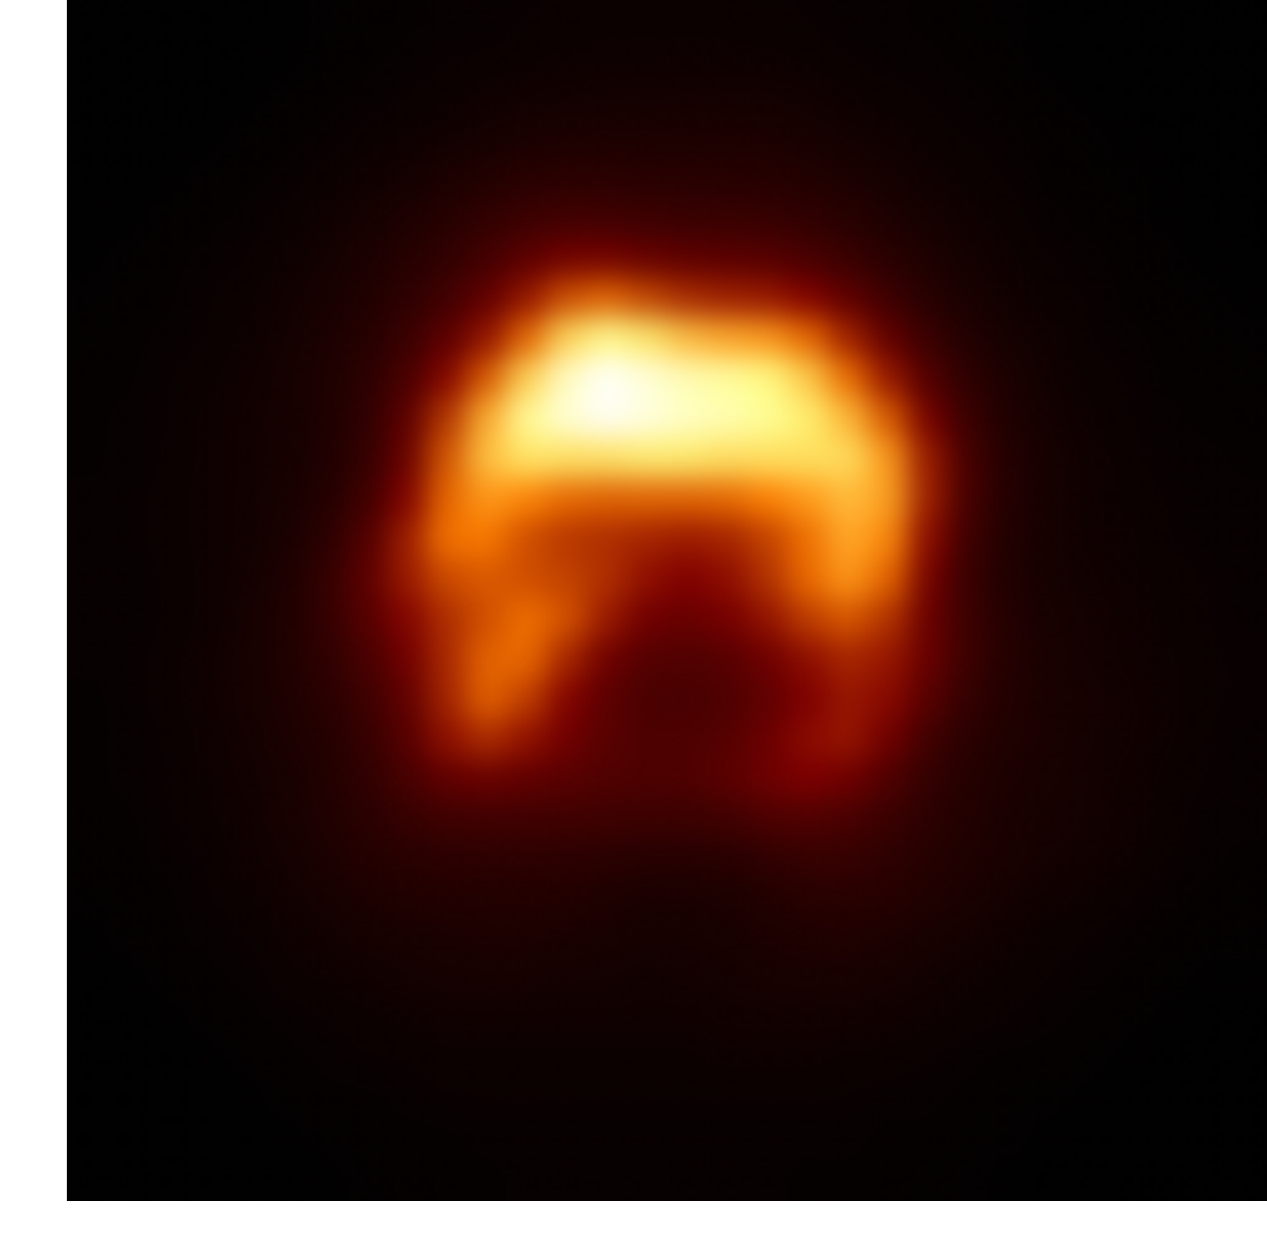}} } &
			\includegraphics[height=0.12\linewidth]{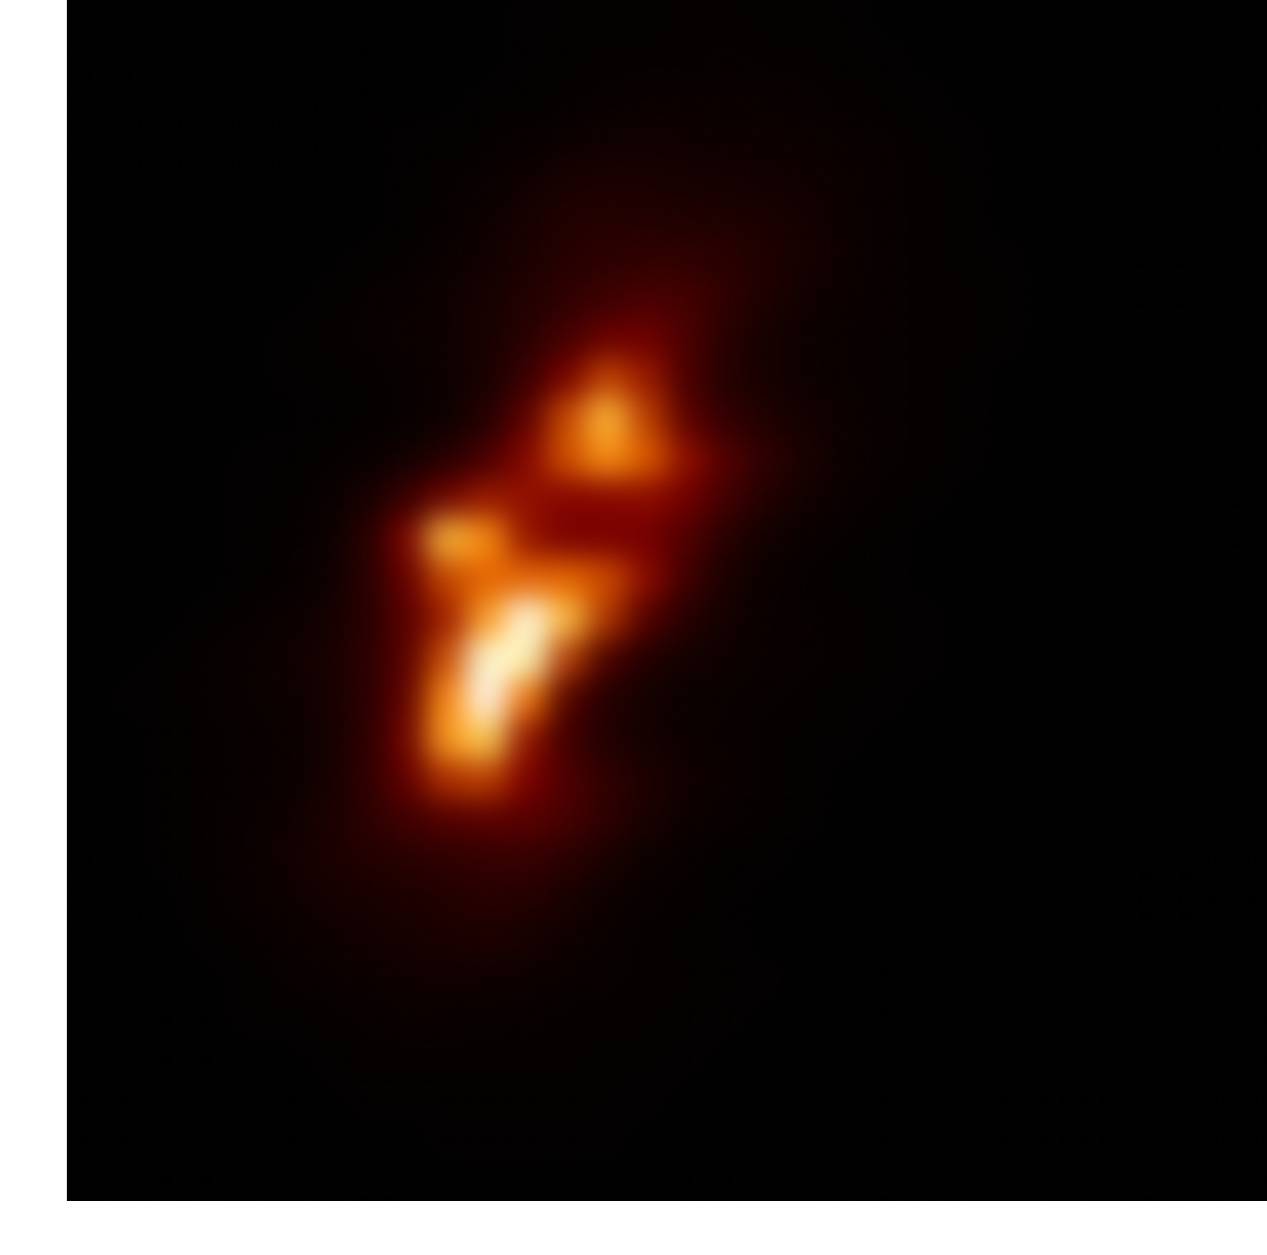} &
			\includegraphics[height=0.12\linewidth]{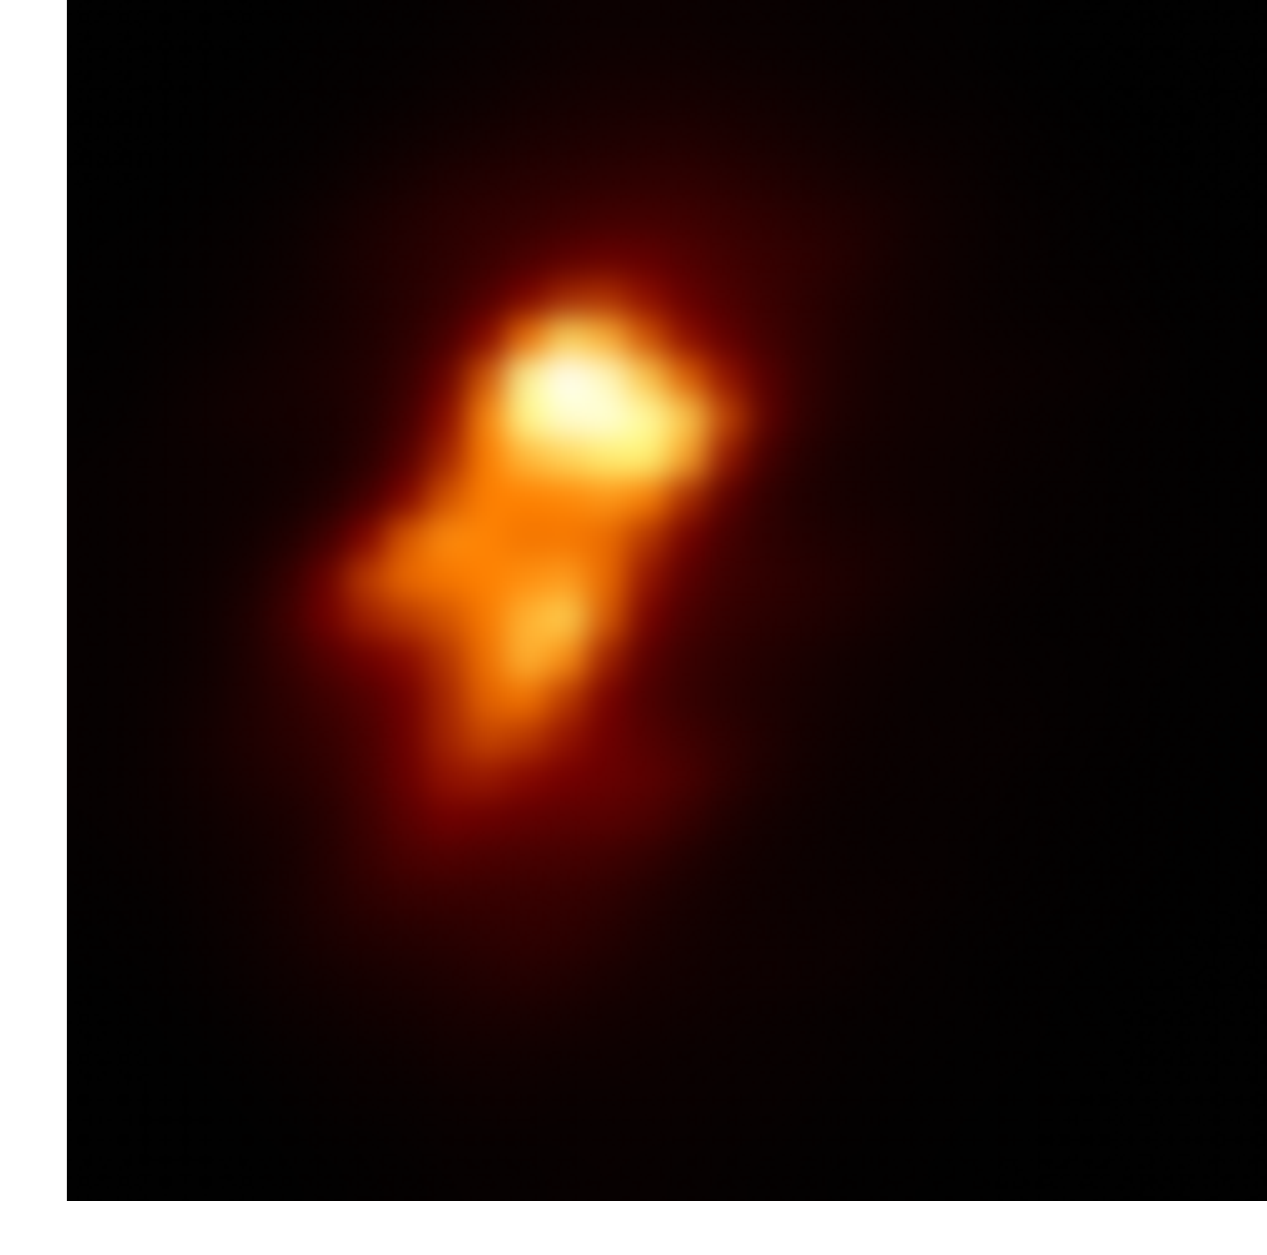} &
			\includegraphics[height=0.12\linewidth]{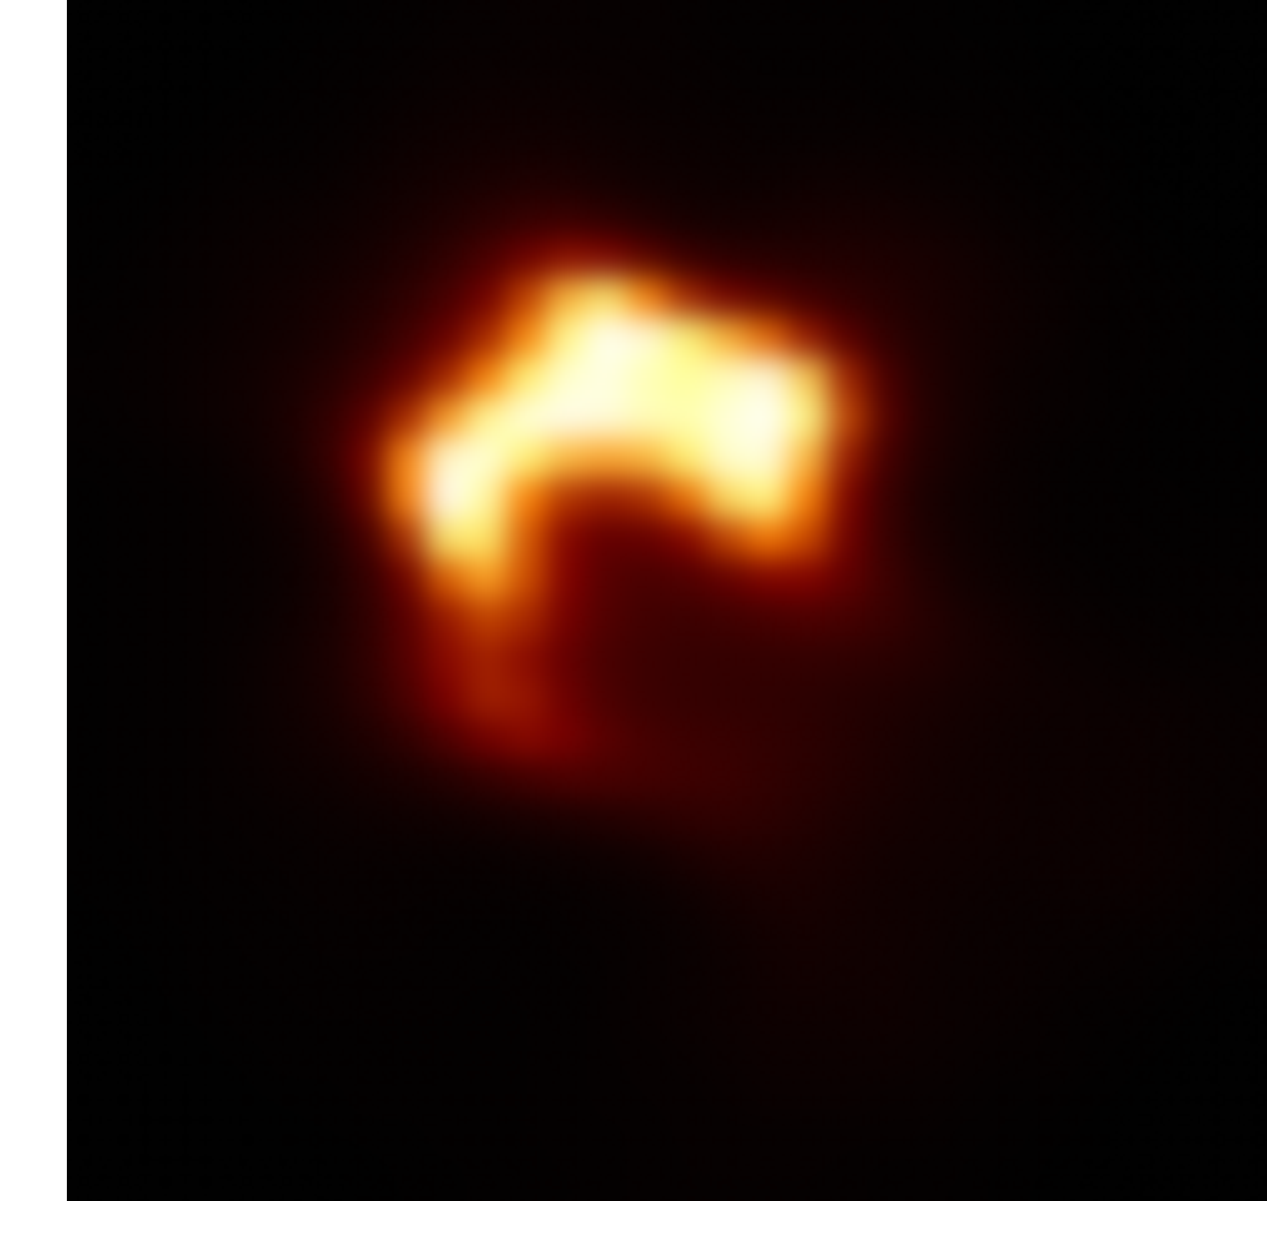} &
			\includegraphics[height=0.12\linewidth]{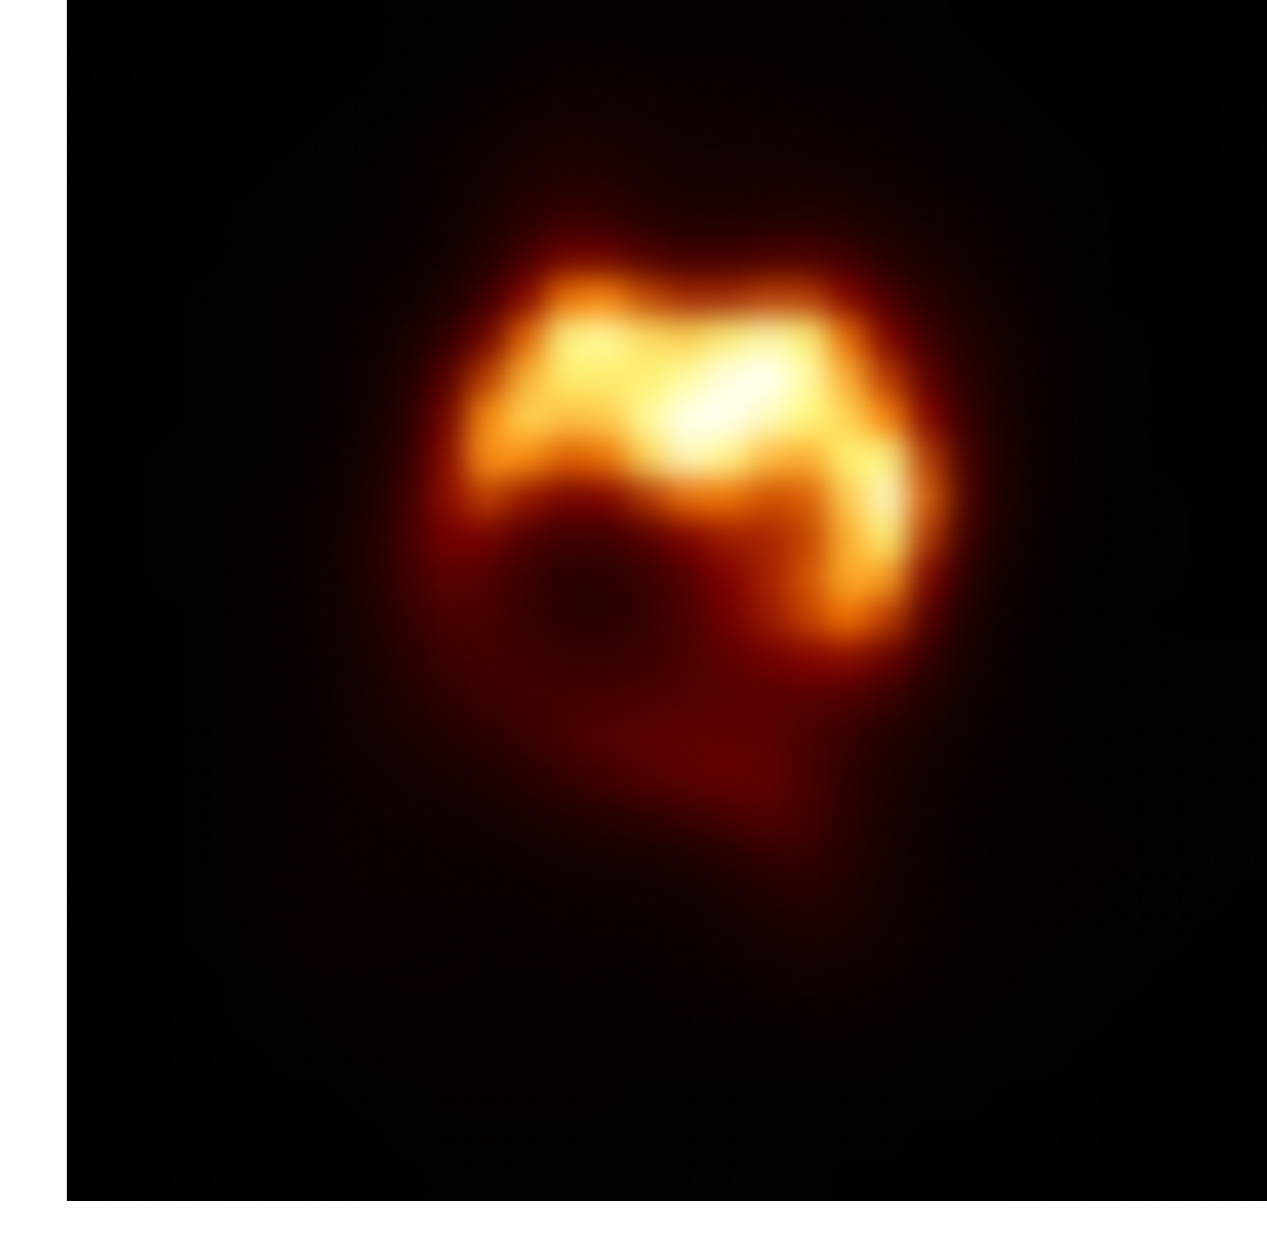} &
			\includegraphics[height=0.12\linewidth]{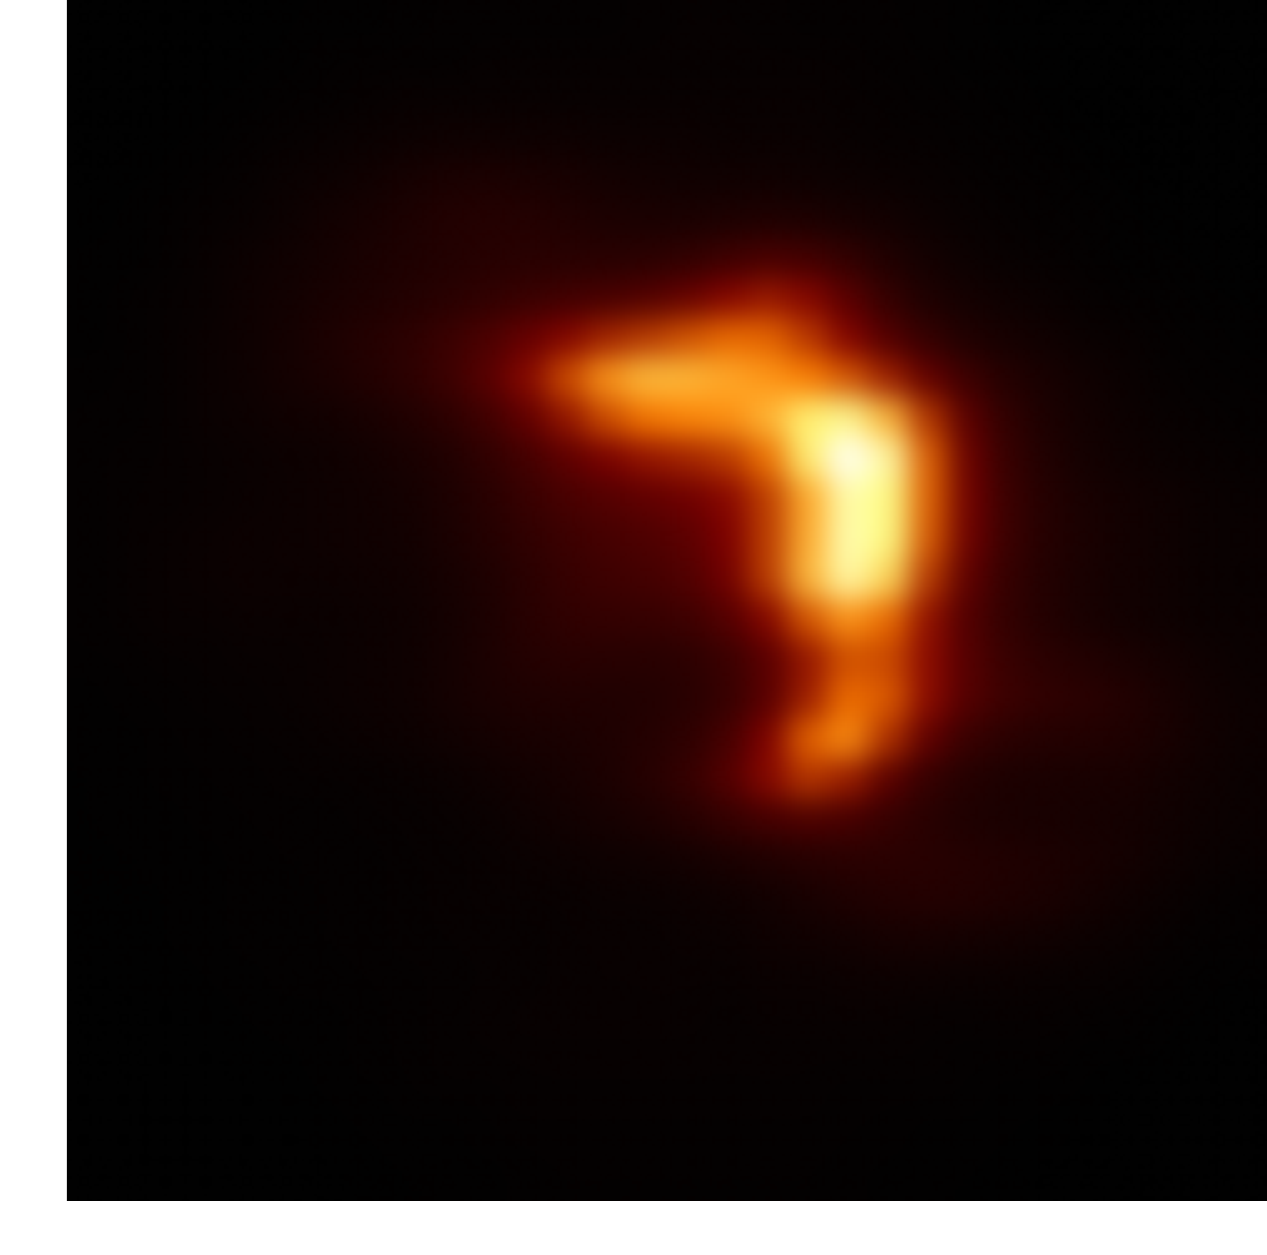} &
			\includegraphics[height=0.12\linewidth]{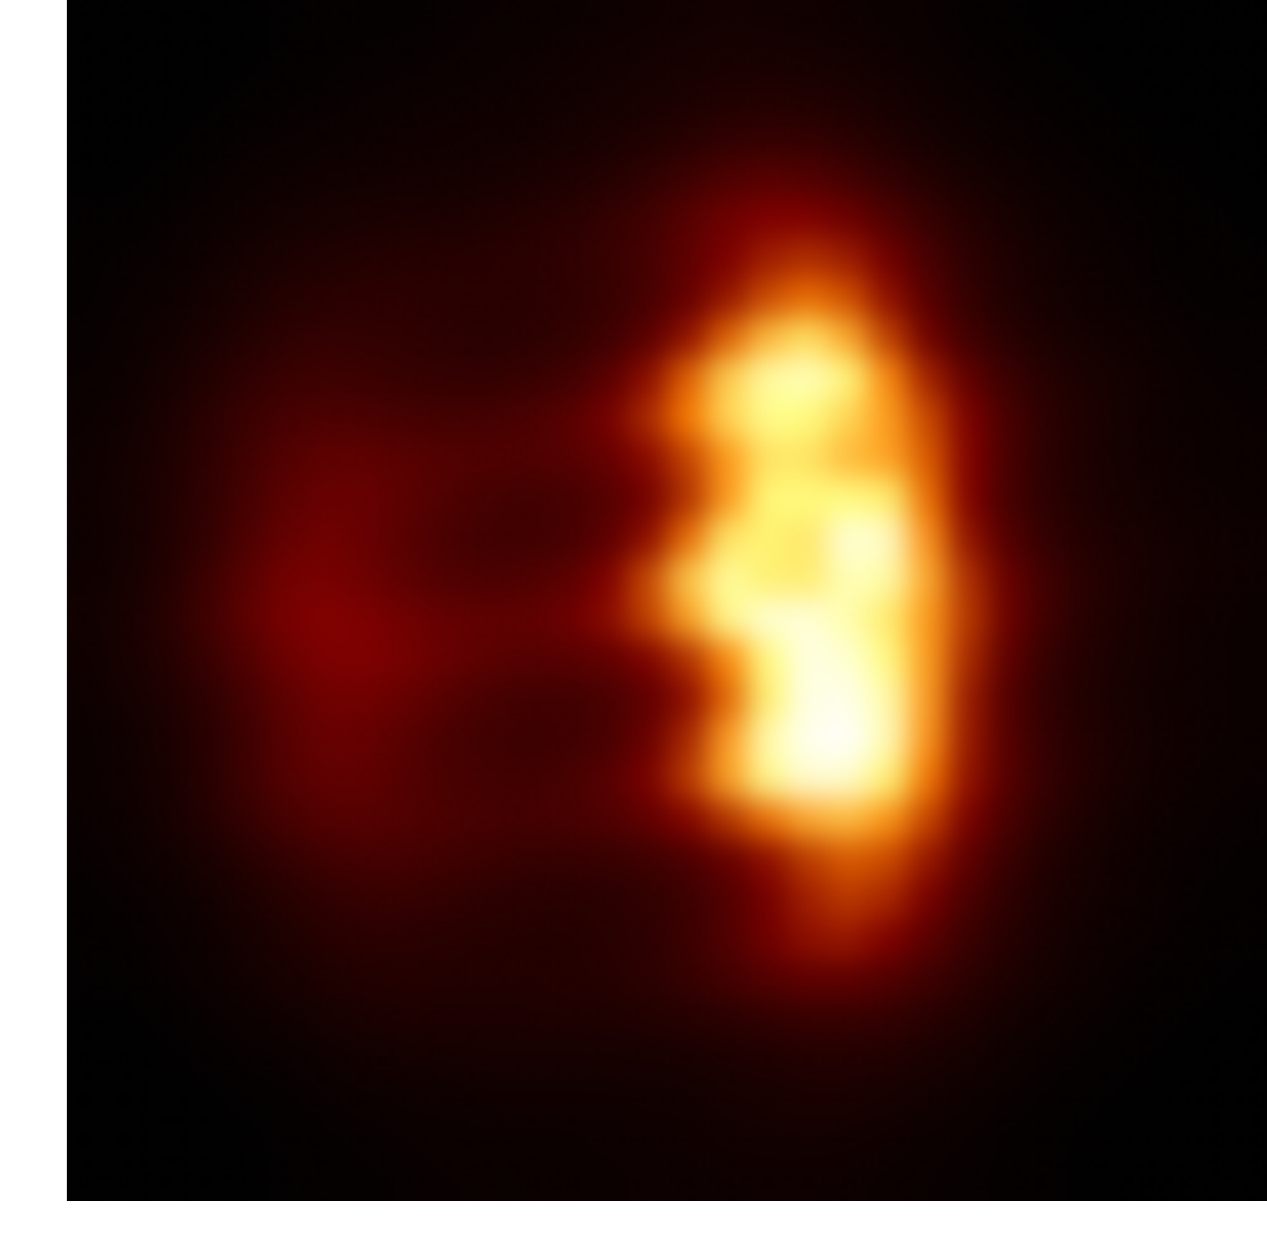} 
			\\          
			&\vspace{-.1in} &&&&&&\\
			\multirow{1}{*}[0.7in]{ \rotatebox[origin=t]{90}{  \specialcell{ \small{\textsf{StarWarps:}} \\  \small{\textsf{No Warp}}}  }}
			&
			{{\includegraphics[height=0.12\linewidth]{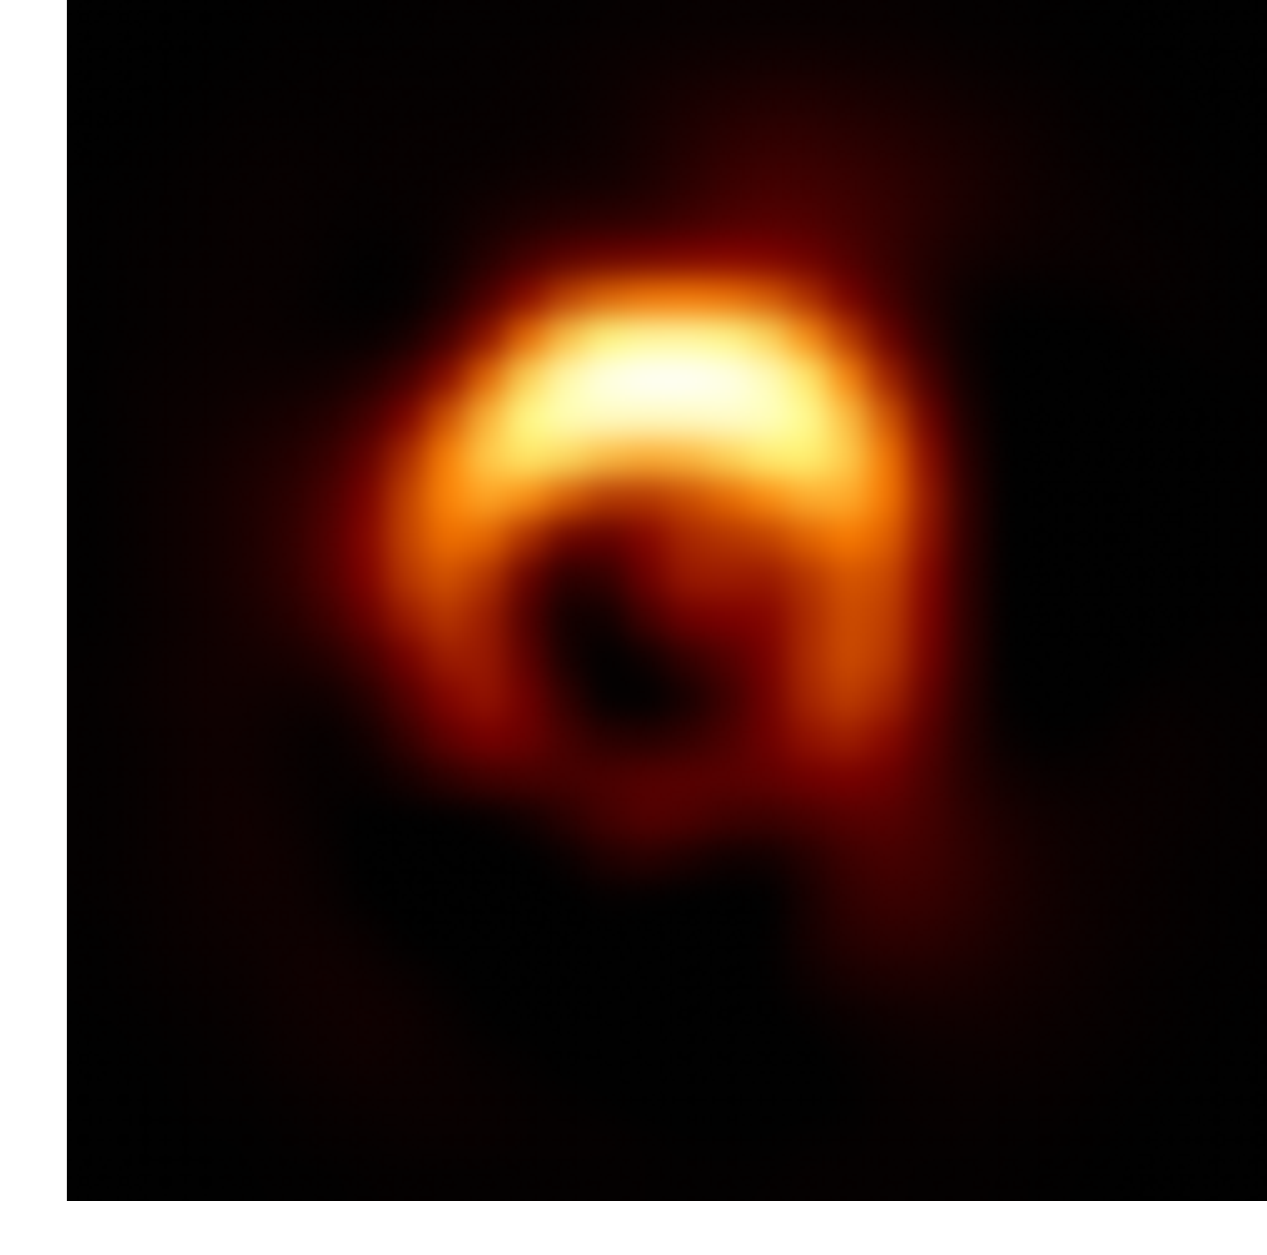}} } &
			\includegraphics[height=0.12\linewidth]{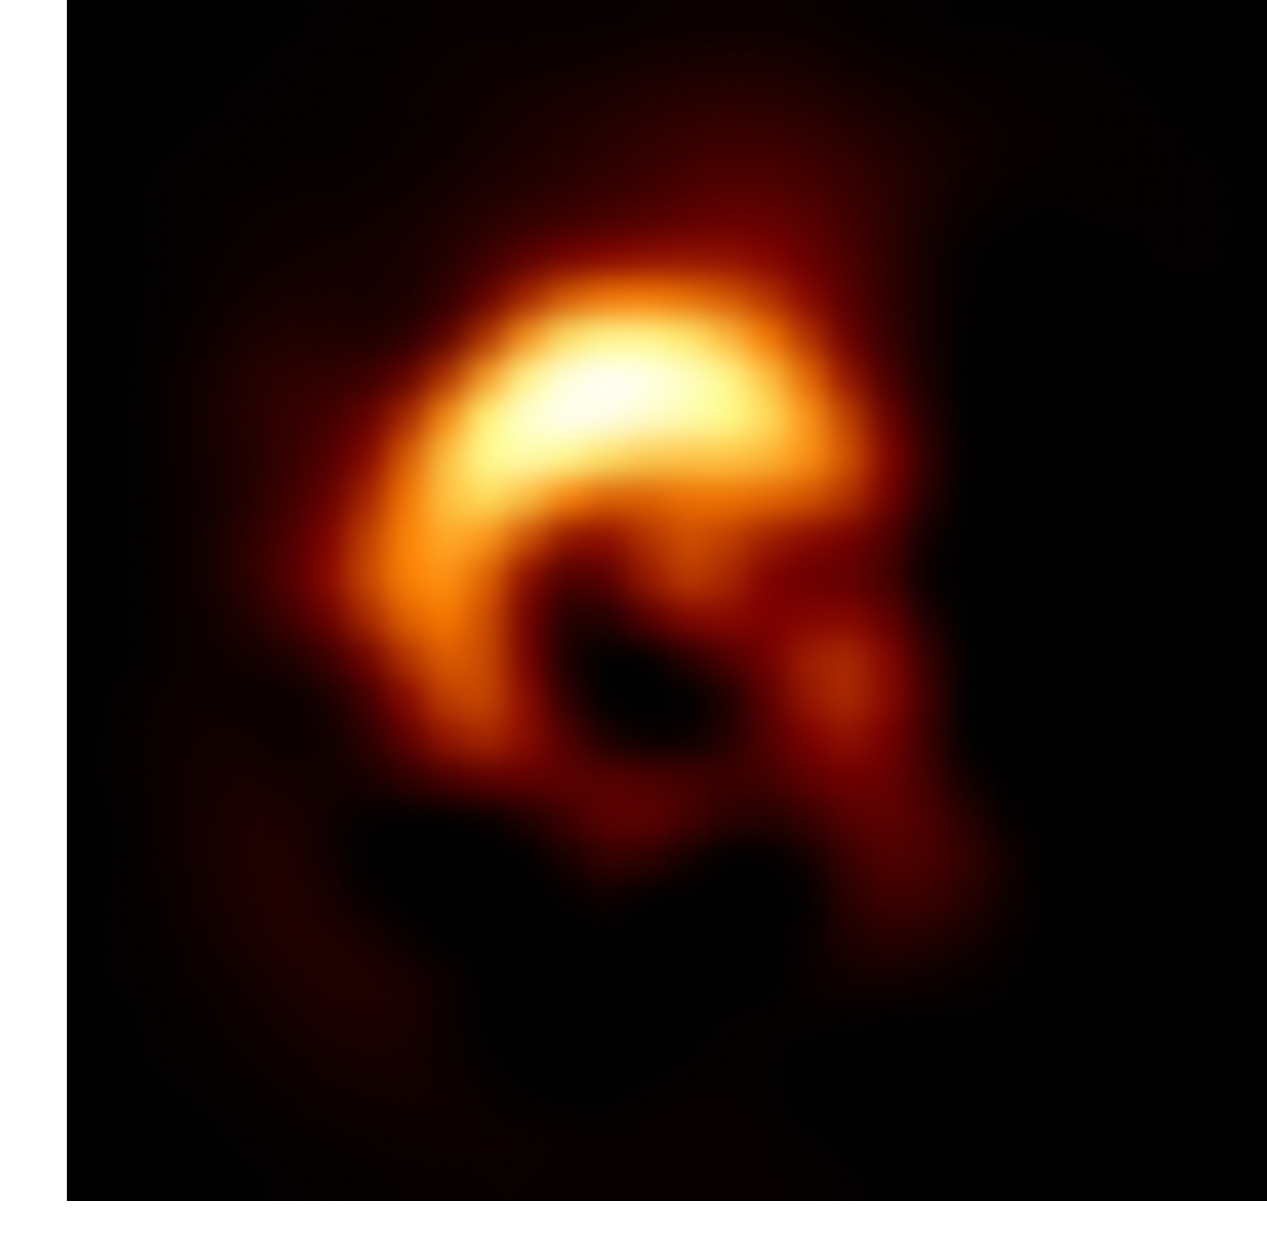} &
			\includegraphics[height=0.12\linewidth]{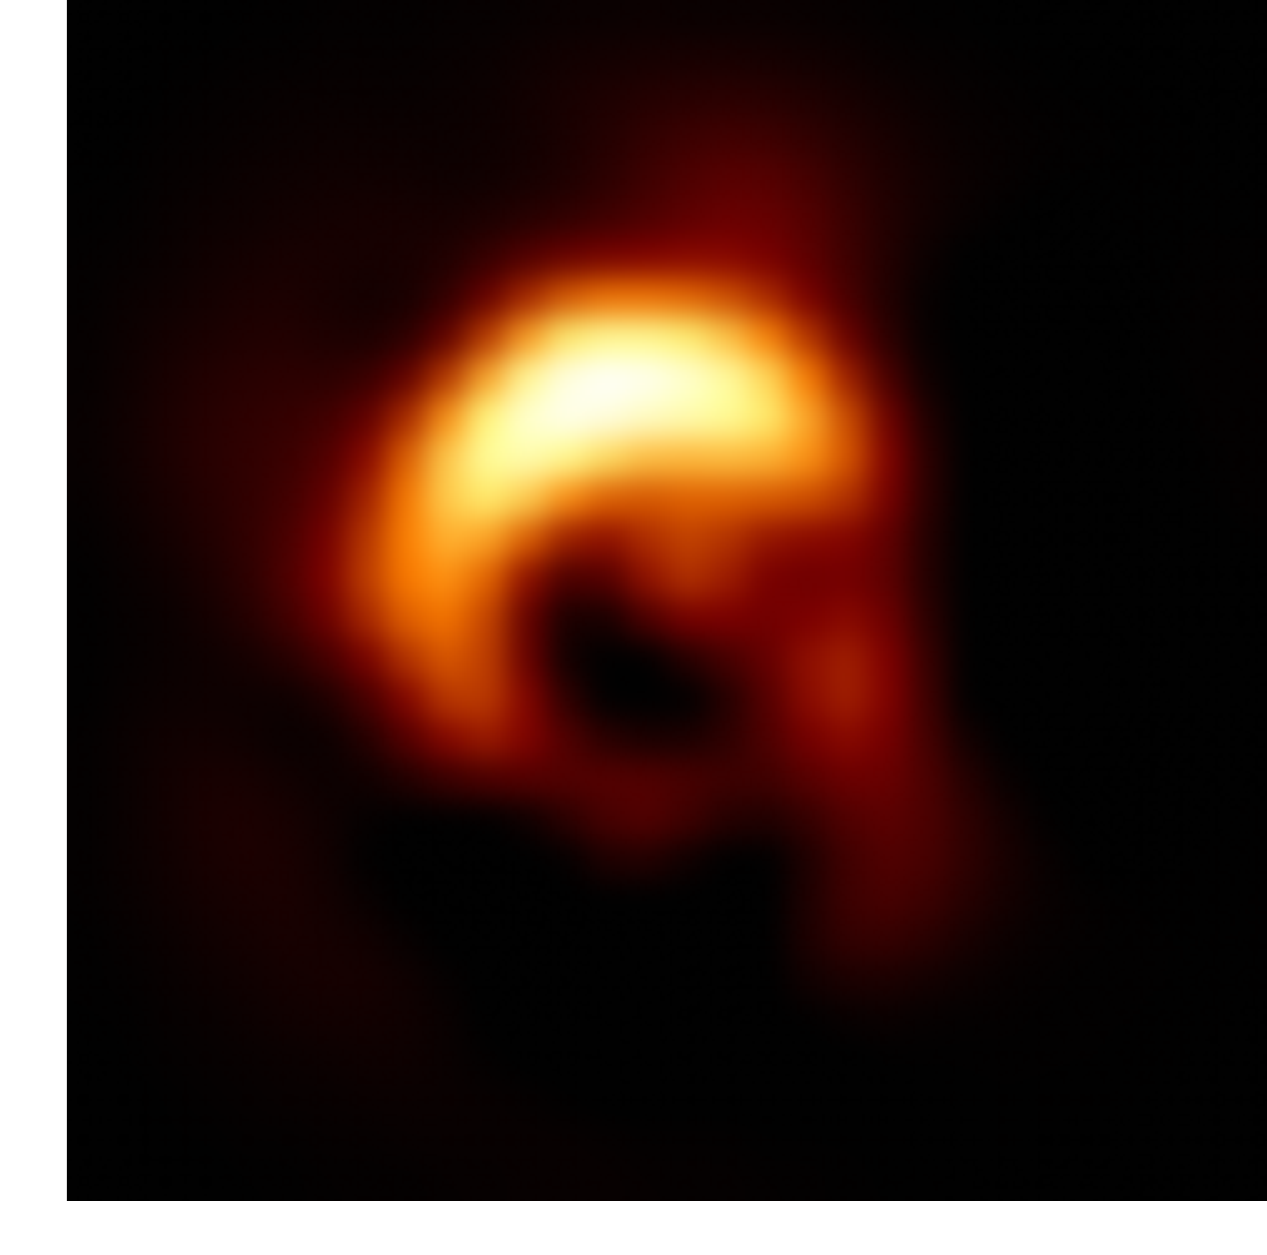} &
			\includegraphics[height=0.12\linewidth]{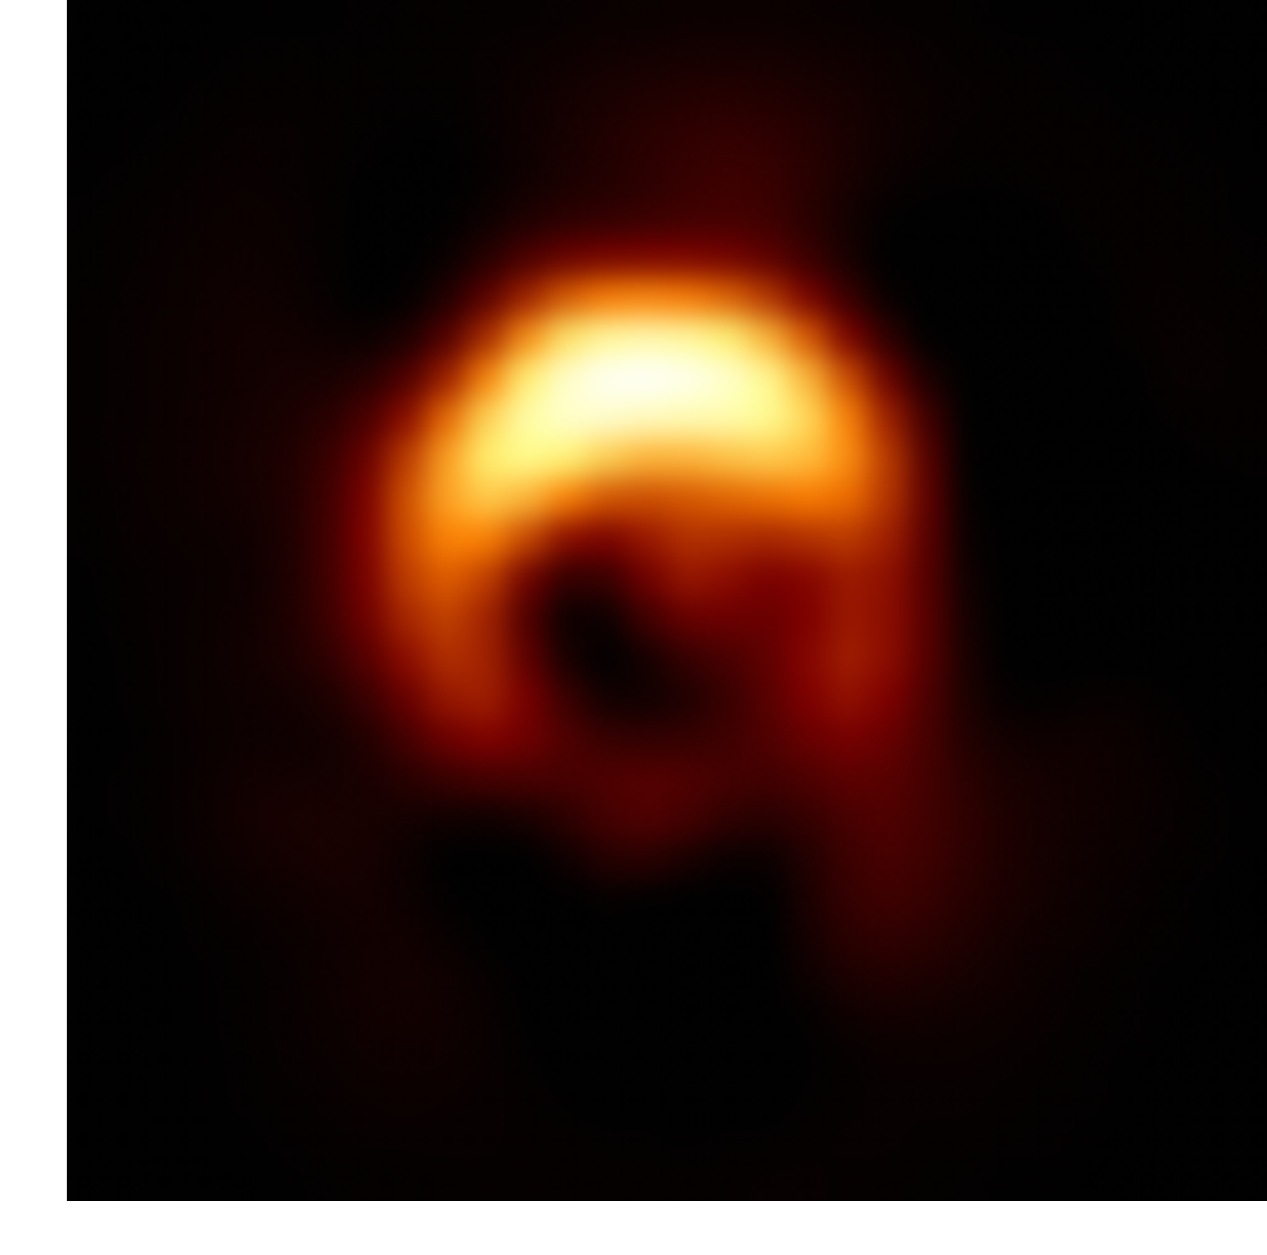} &
			\includegraphics[height=0.12\linewidth]{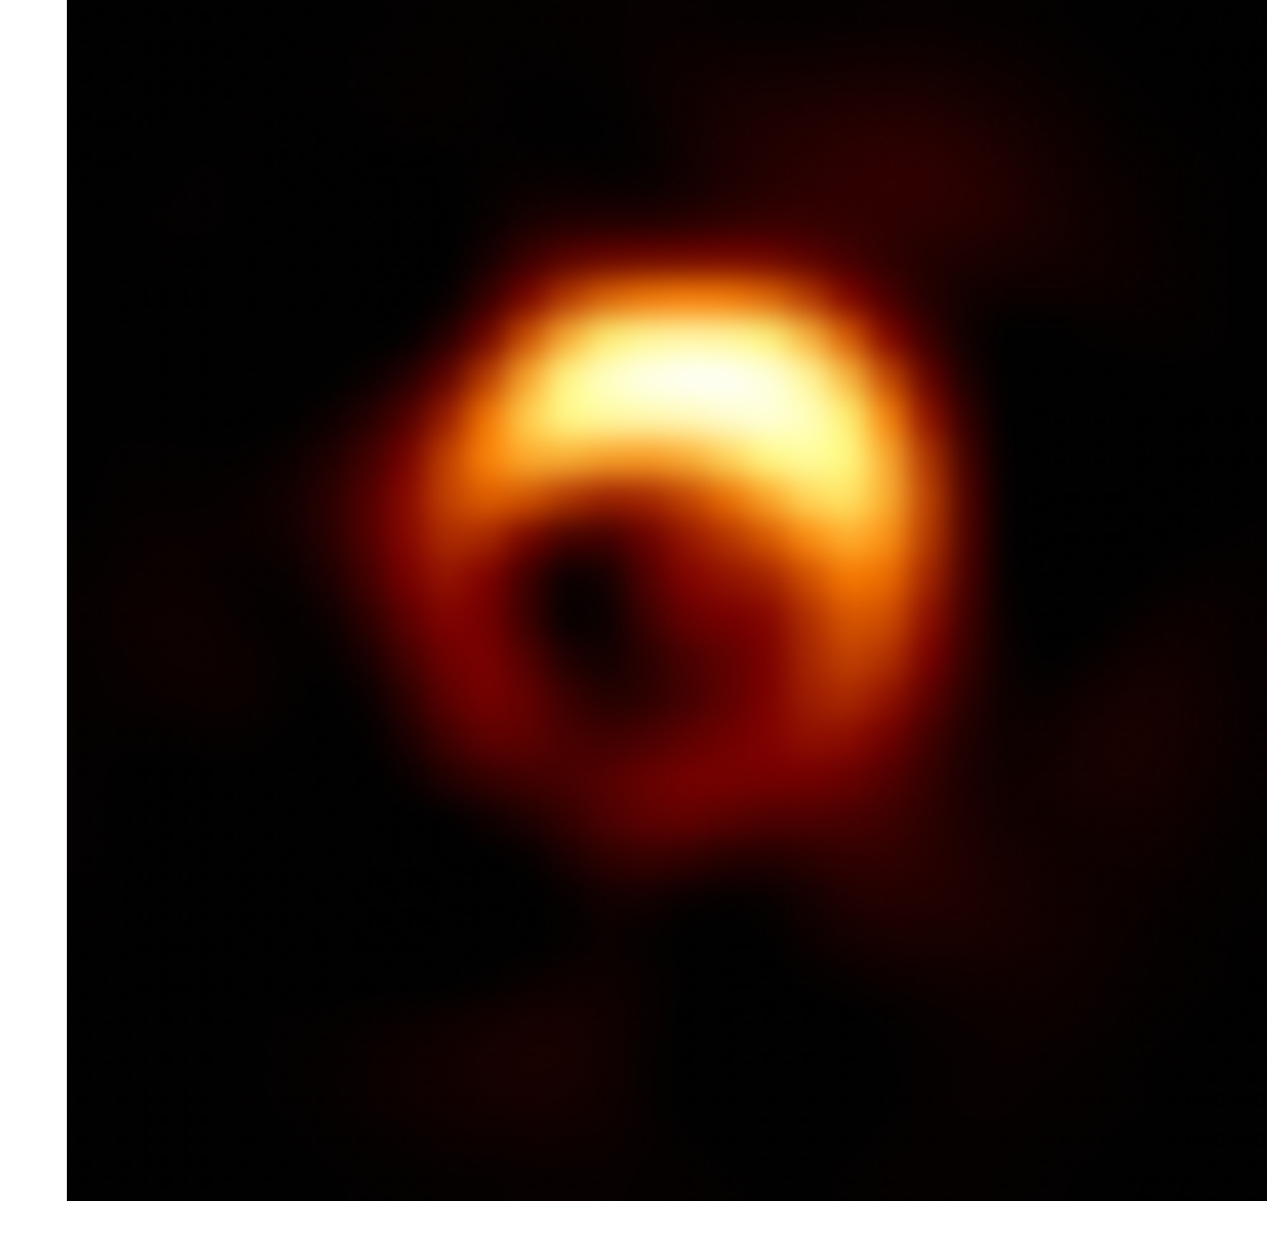} &
			\includegraphics[height=0.12\linewidth]{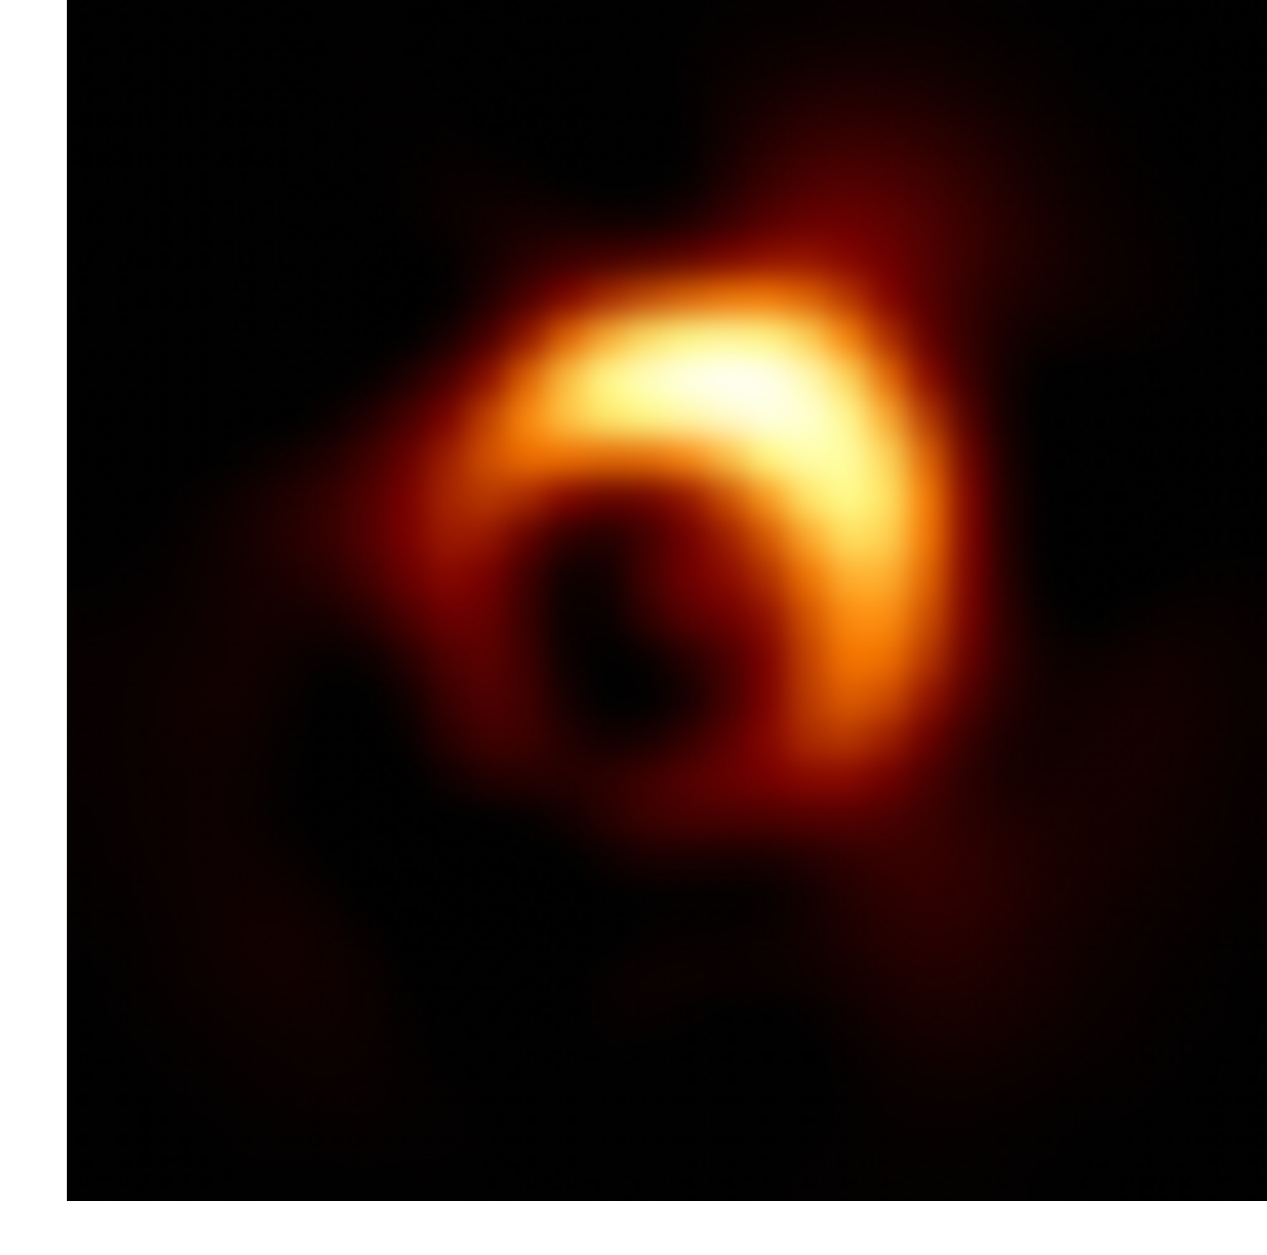} &
			\includegraphics[height=0.12\linewidth]{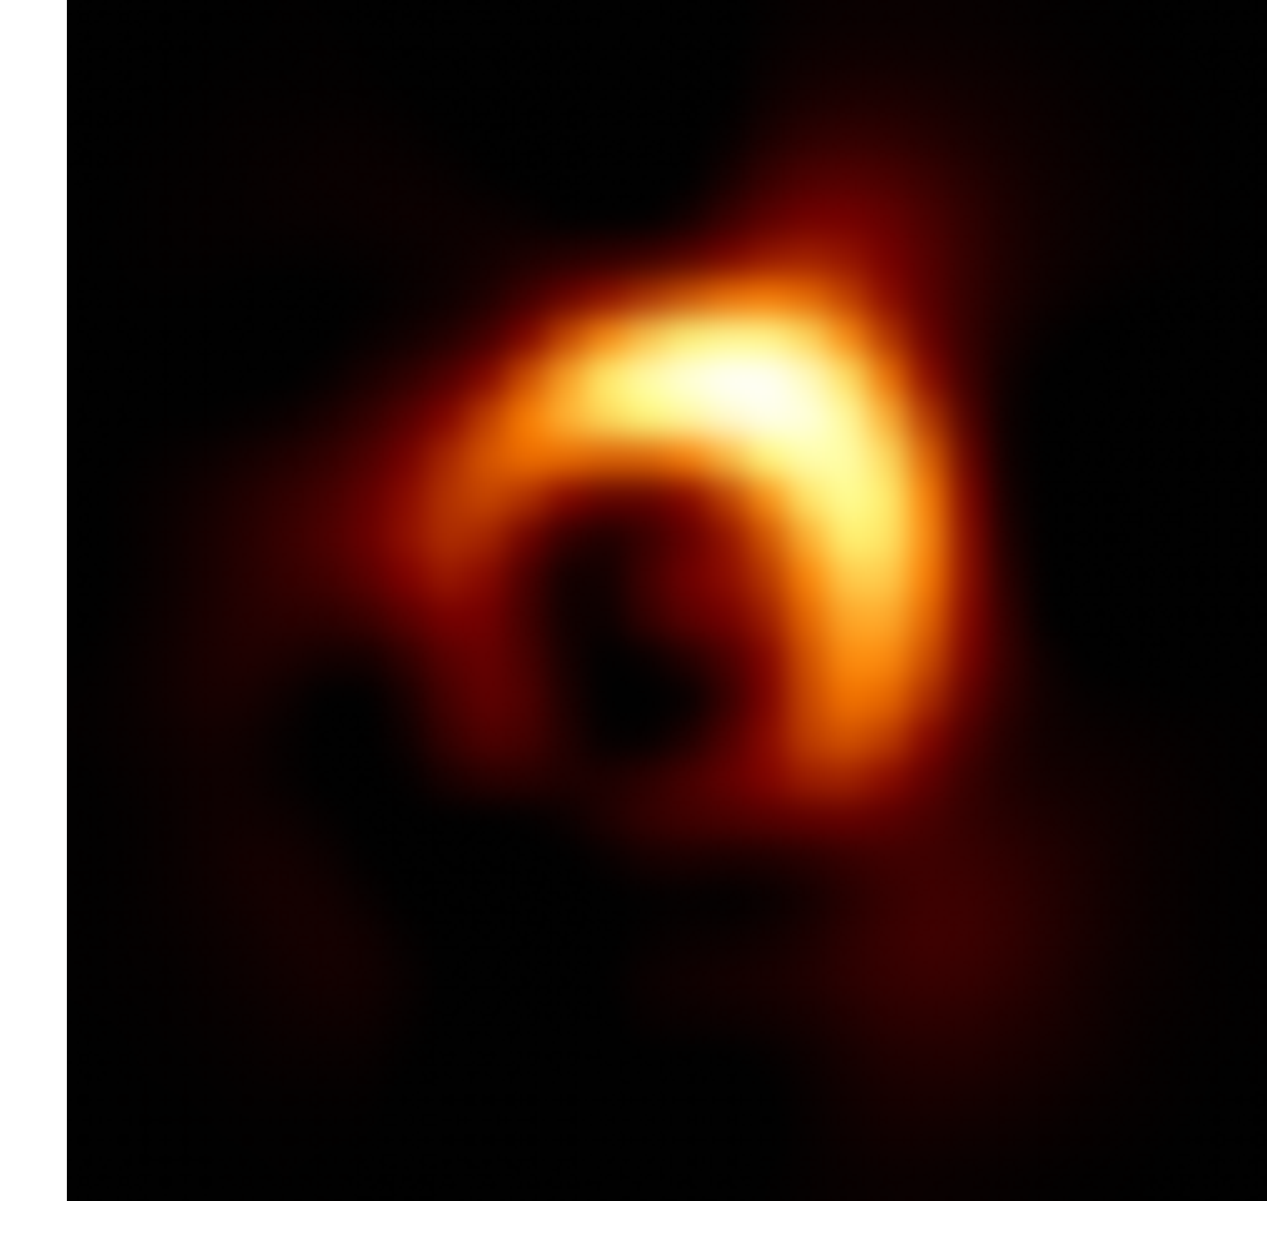} 
			\\          
			&\vspace{-.1in} &&&&&&\\
			\multirow{1}{*}[0.7in]{ \rotatebox[origin=t]{90}{  \specialcell{ \small{\textsf{StarWarps:}} \\  \small{\textsf{Learn Warp}}}  }}
			&
			%{{\includegraphics[height=0.12\linewidth]{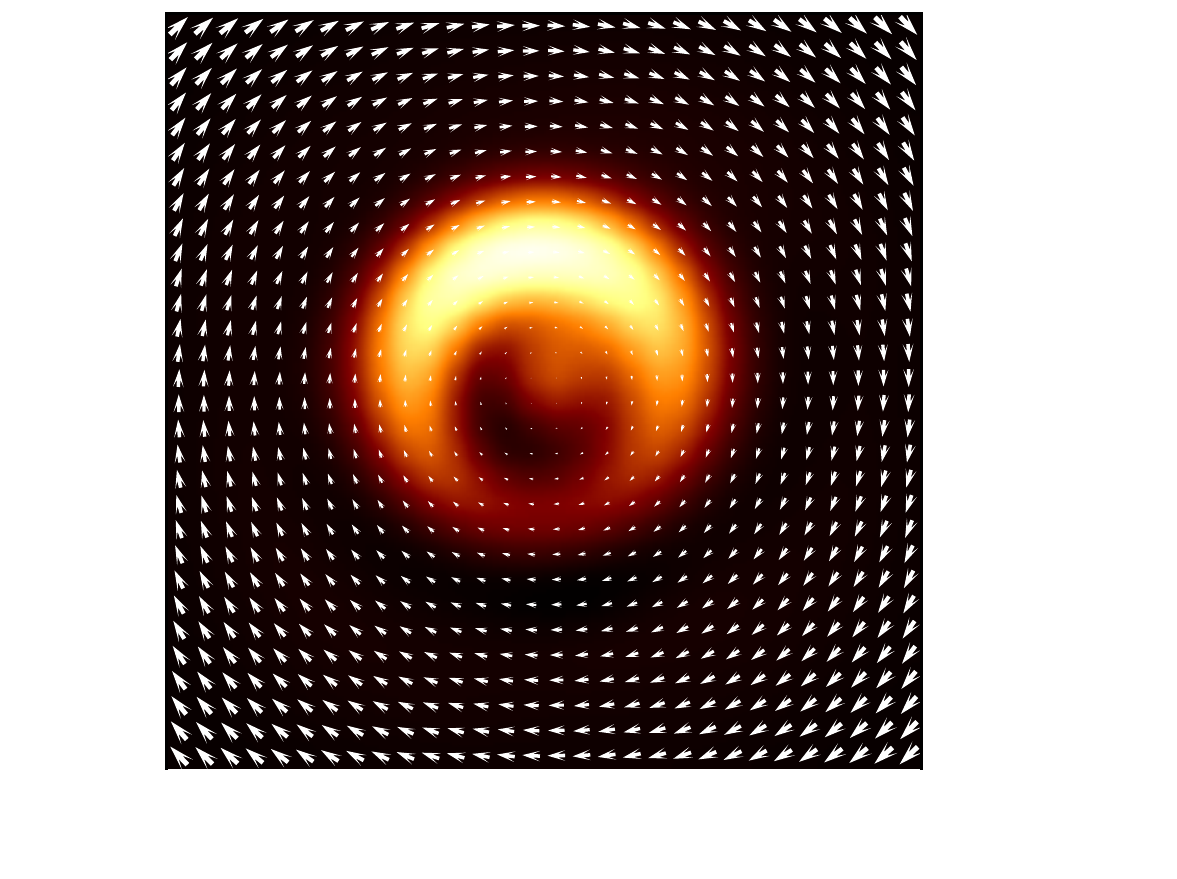}} } 
			%\hspace{0.02in} 
			{{\includegraphics[height=0.12\linewidth]{figures/recov_flowfields/rot30_vis/flow_noaxis.pdf}} } &
			\includegraphics[height=0.12\linewidth]{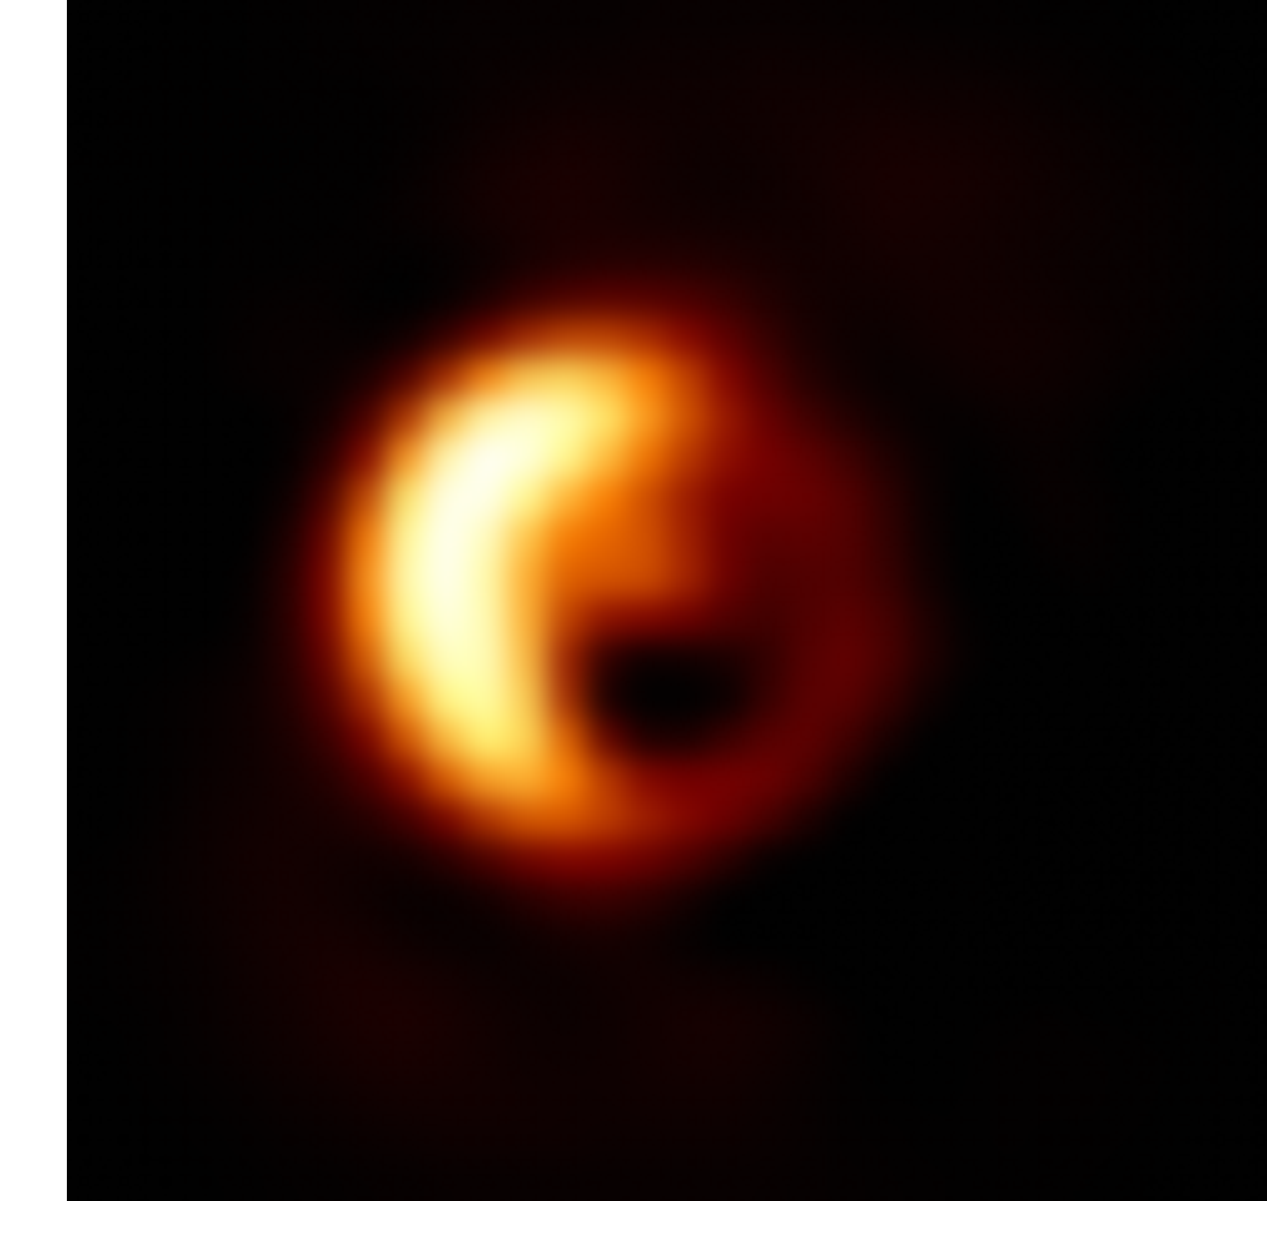} &
			\includegraphics[height=0.12\linewidth]{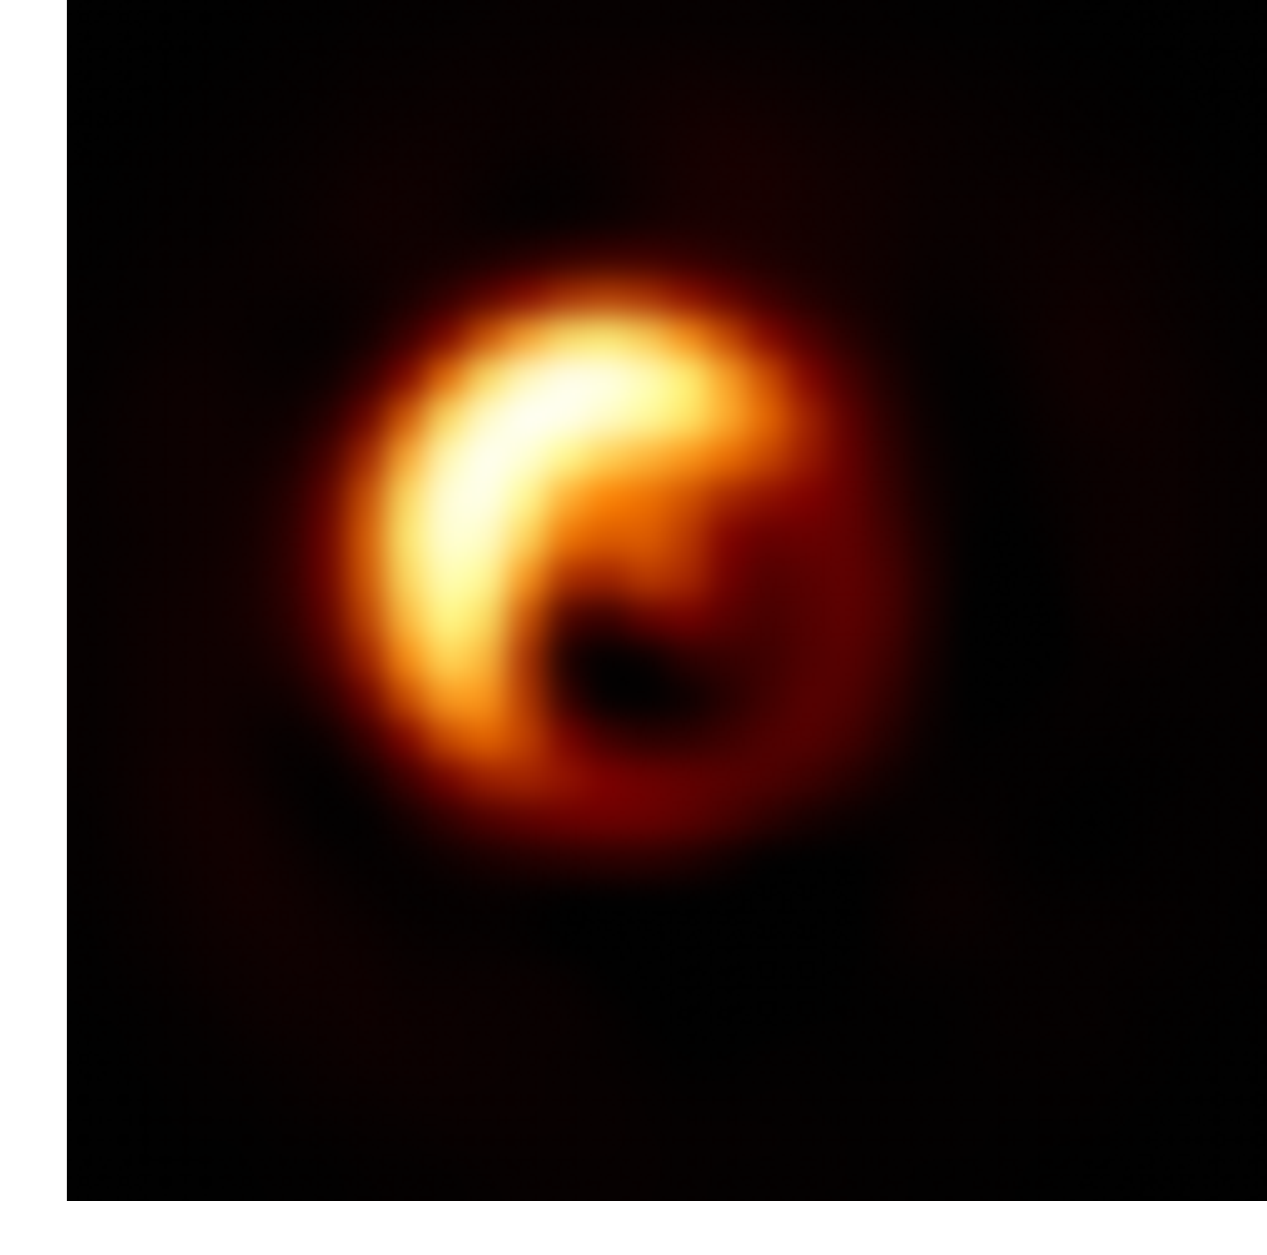} &
			\includegraphics[height=0.12\linewidth]{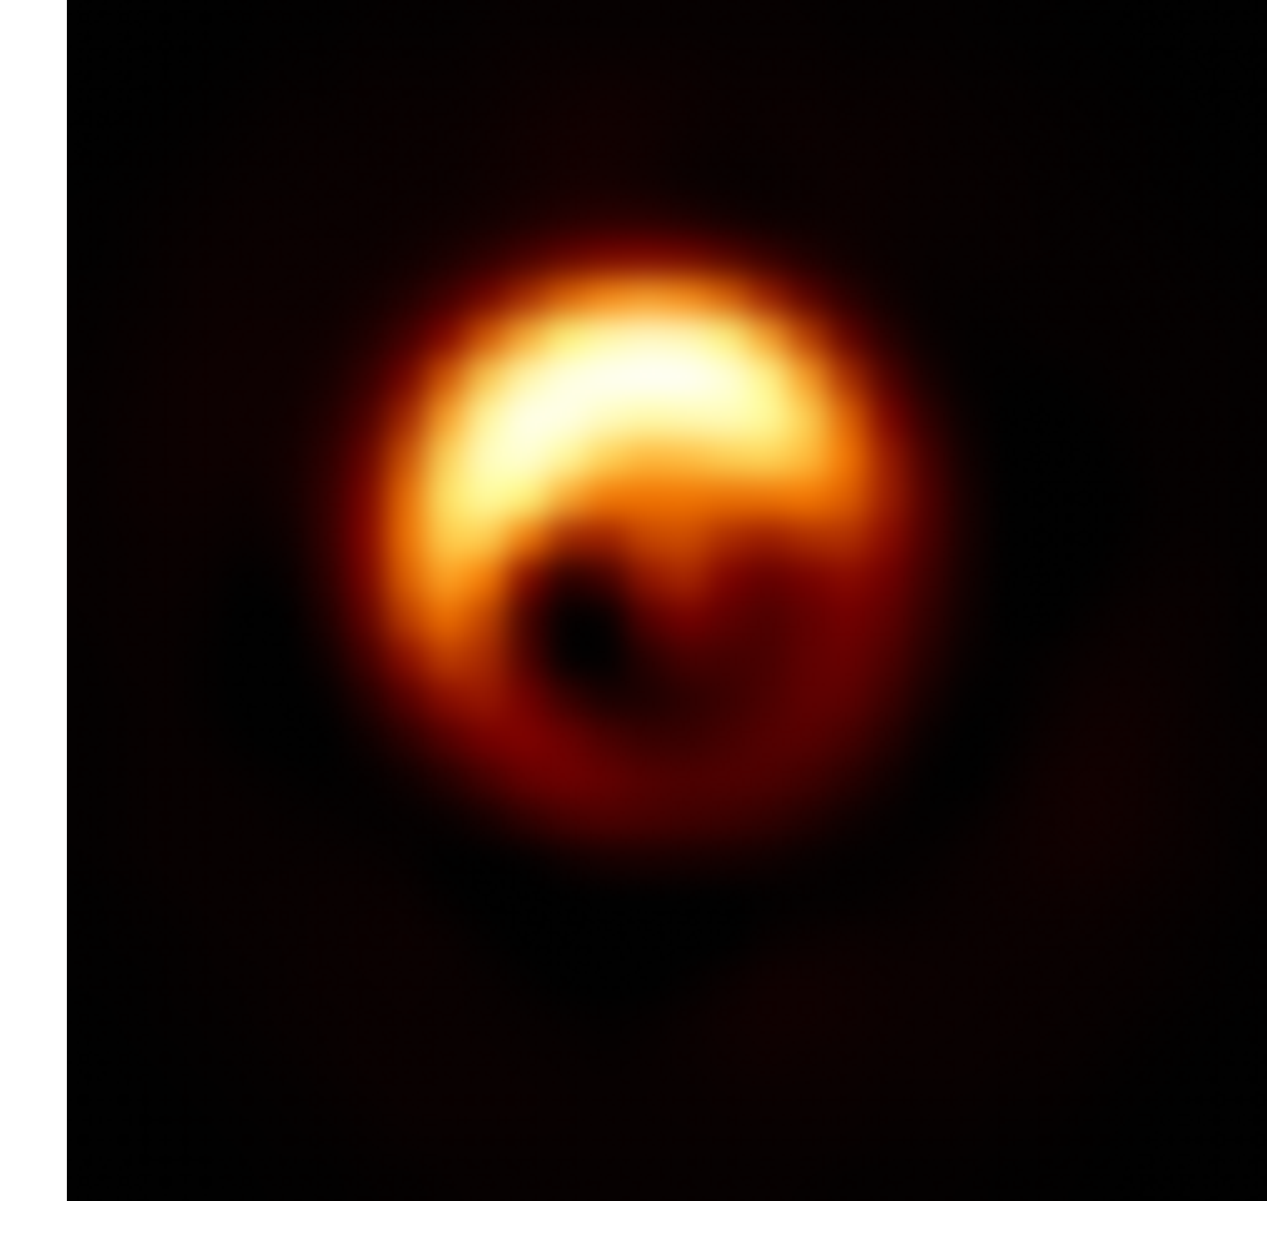} &
			\includegraphics[height=0.12\linewidth]{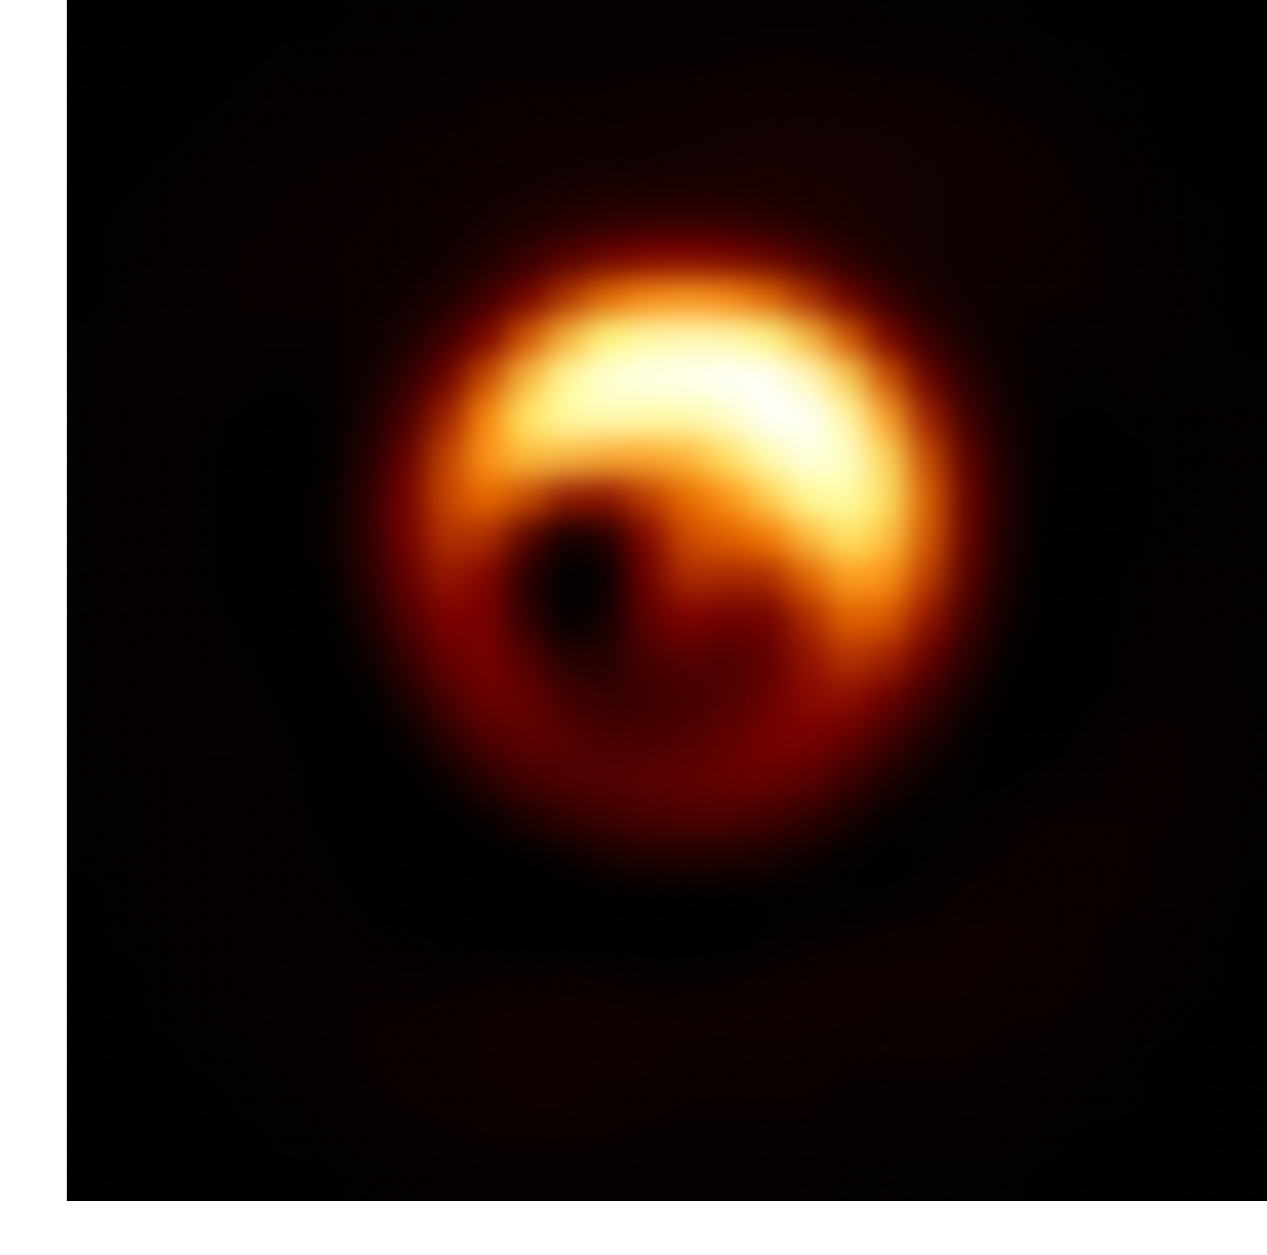} &
			\includegraphics[height=0.12\linewidth]{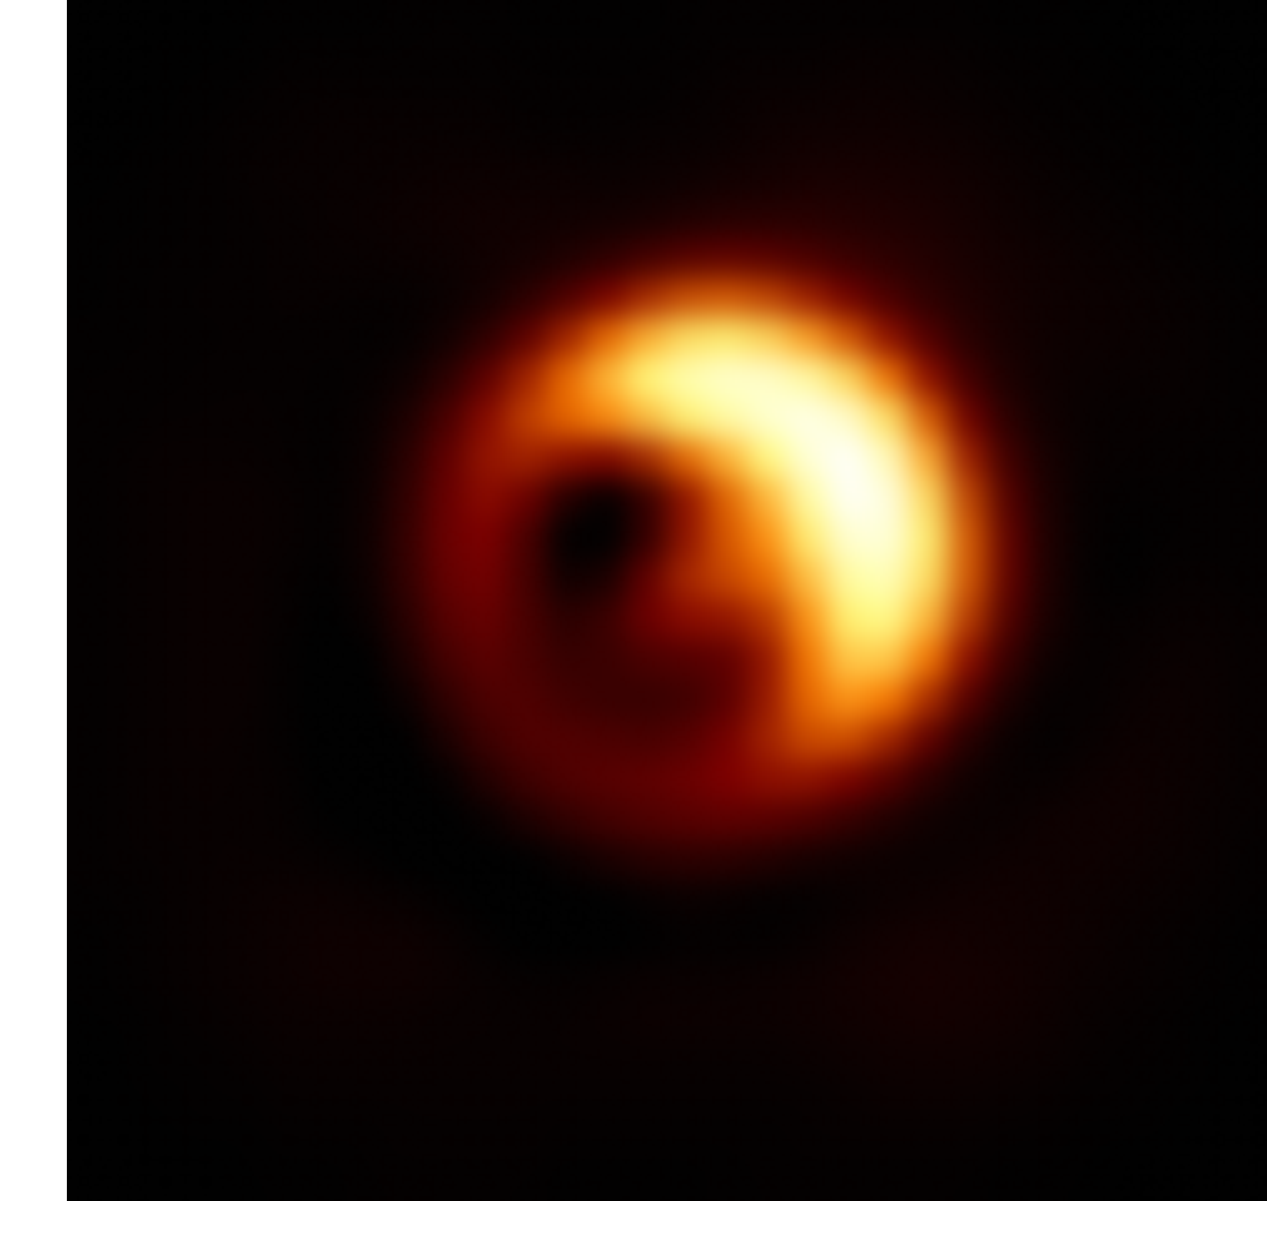} &
			\includegraphics[height=0.12\linewidth]{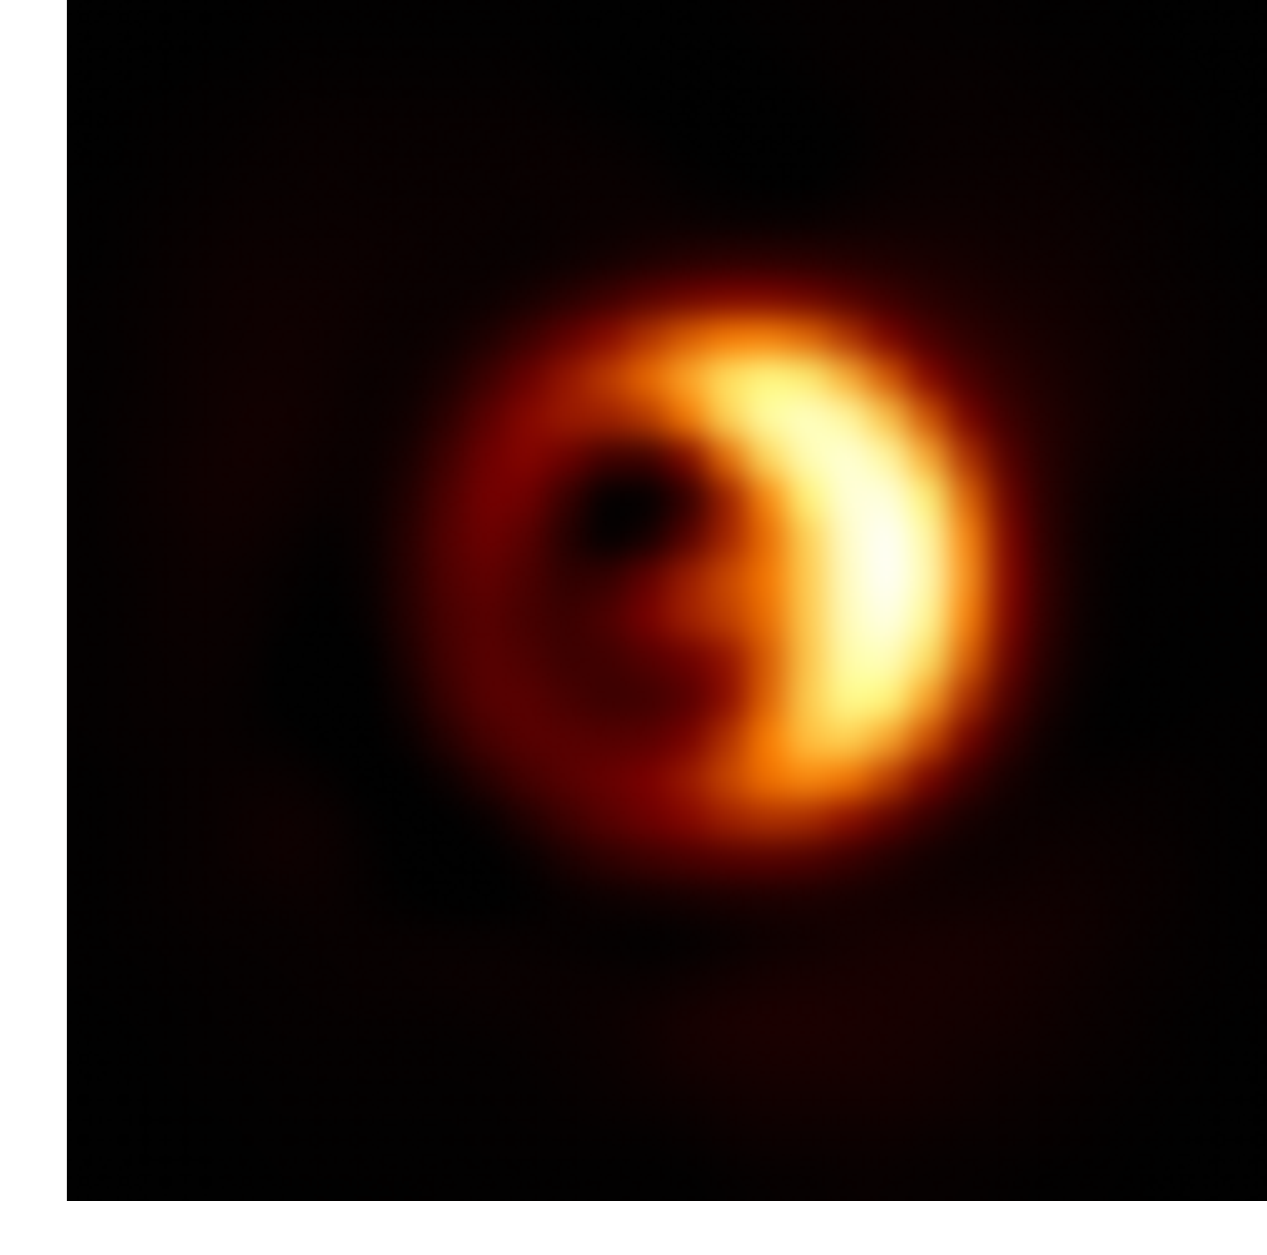}  
			\\ \hline  	
			&\vspace{-.1in} &&&&&&\\
			\multicolumn{8}{c}{  \large{\textsf{ WITH ATMOSPHERIC PHASE ERROR  }}  }
			\\ \hline
			&\vspace{-.1in} &&&&&&\\
			\multirow{1}{*}[.6in]{ \rotatebox[origin=t]{90}{\small{\textsf{Snapshot}} }}
			&
			{{\includegraphics[height=0.12\linewidth]{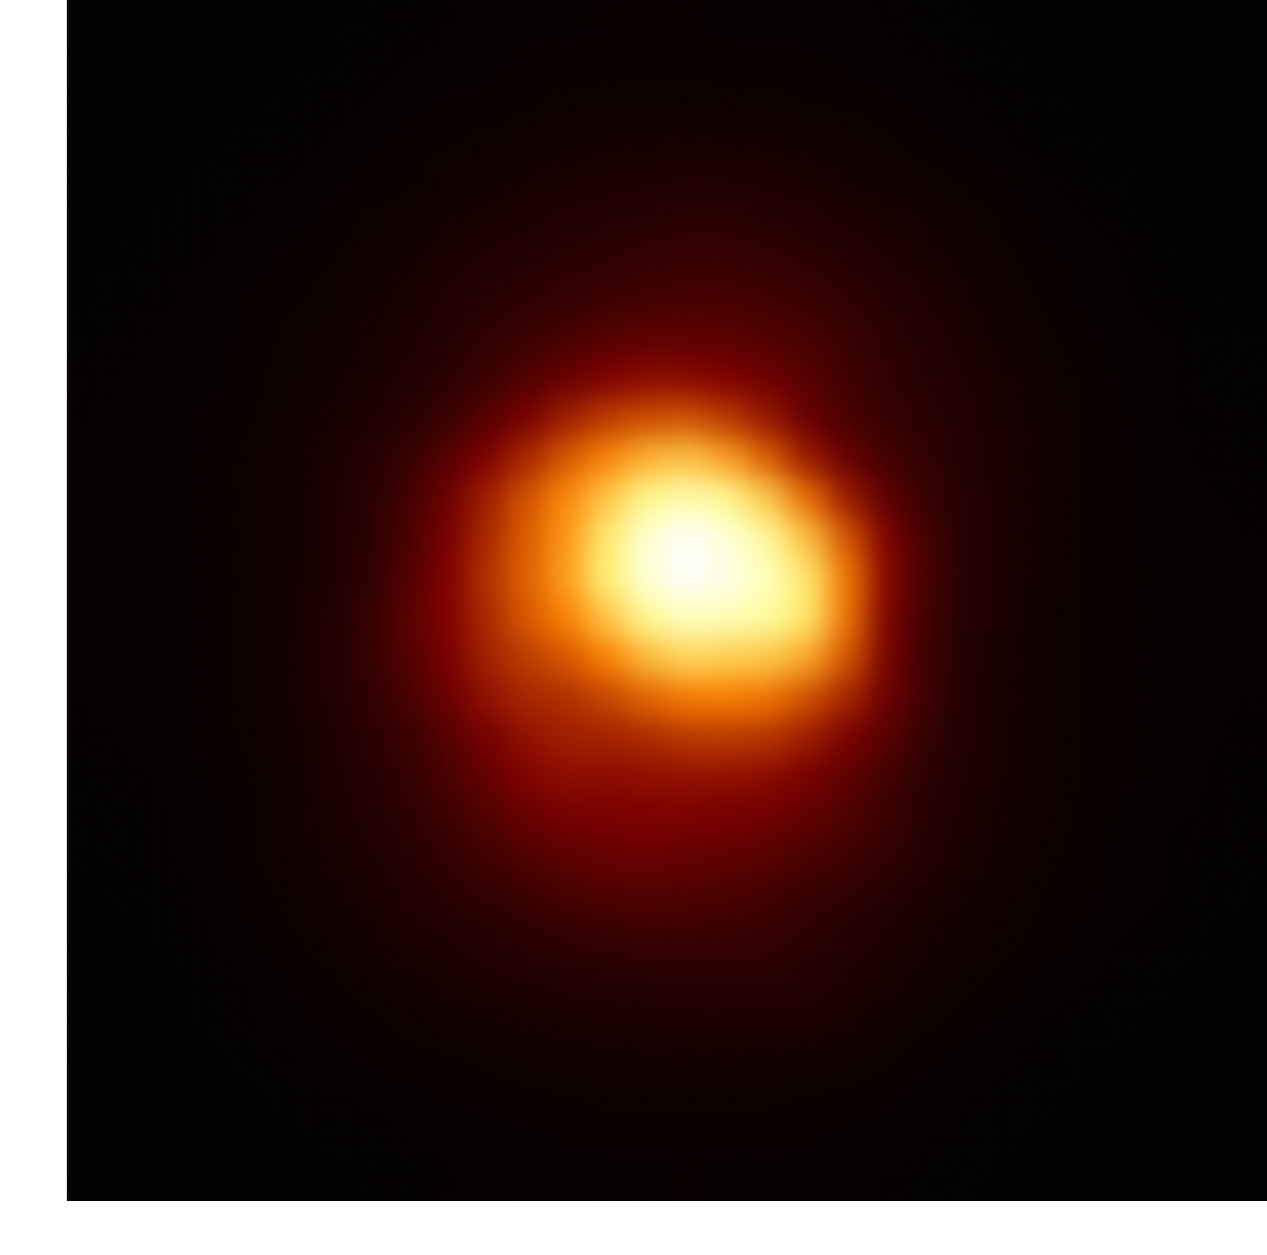}} } &
			\includegraphics[height=0.12\linewidth]{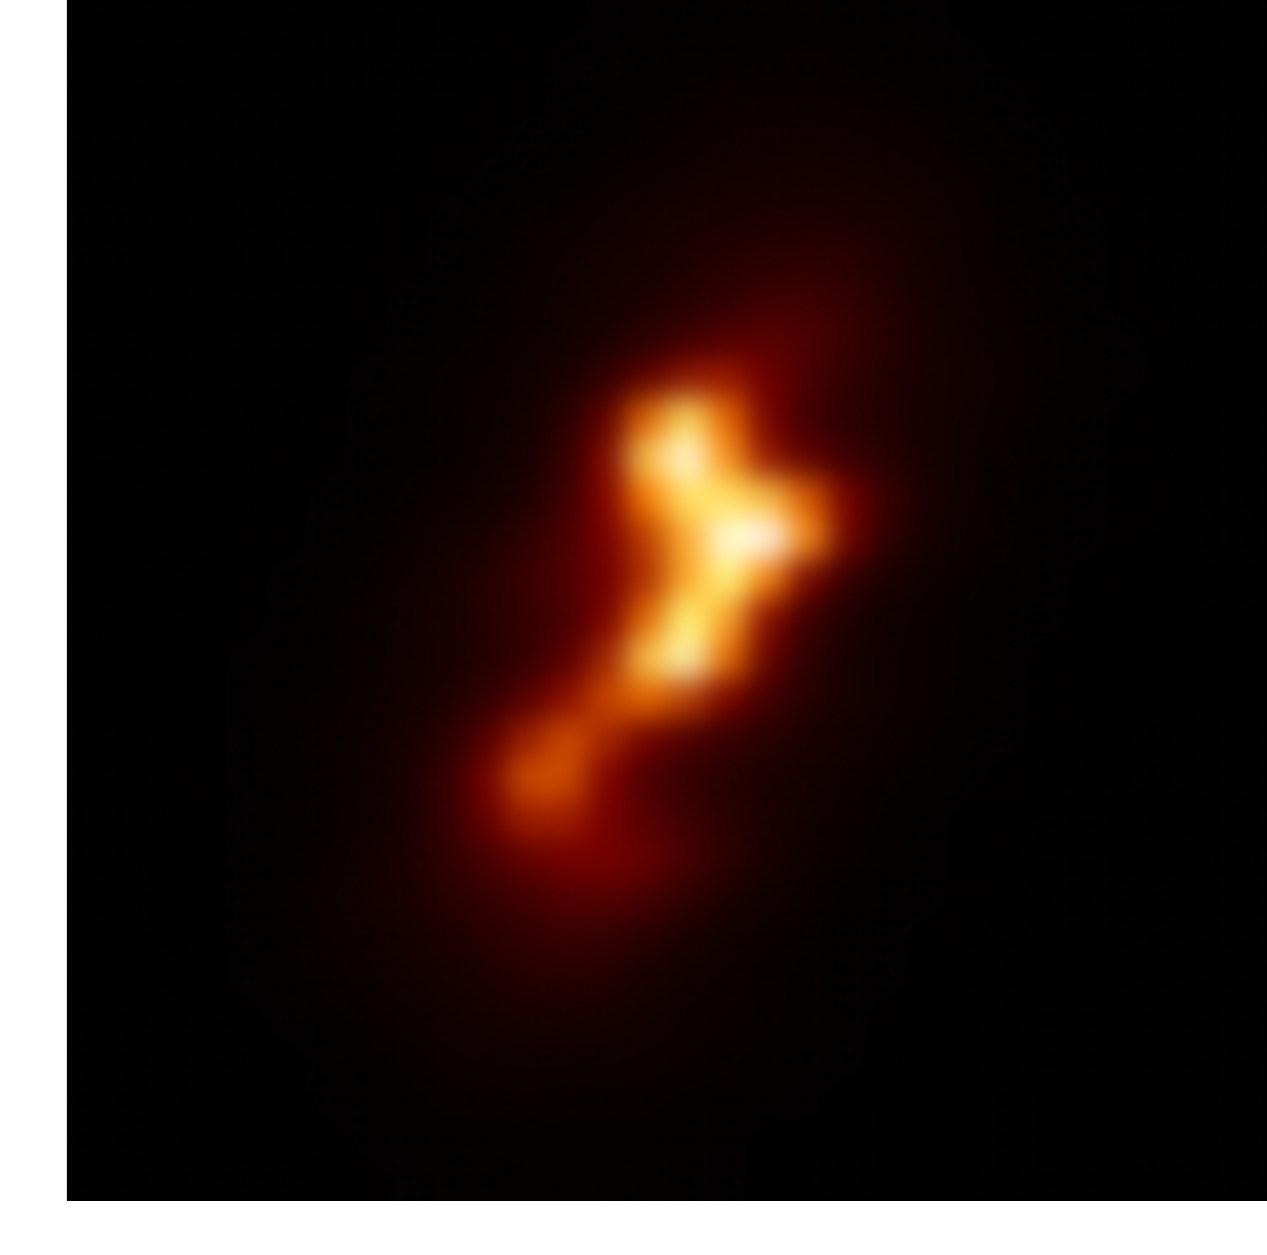} &
			\includegraphics[height=0.12\linewidth]{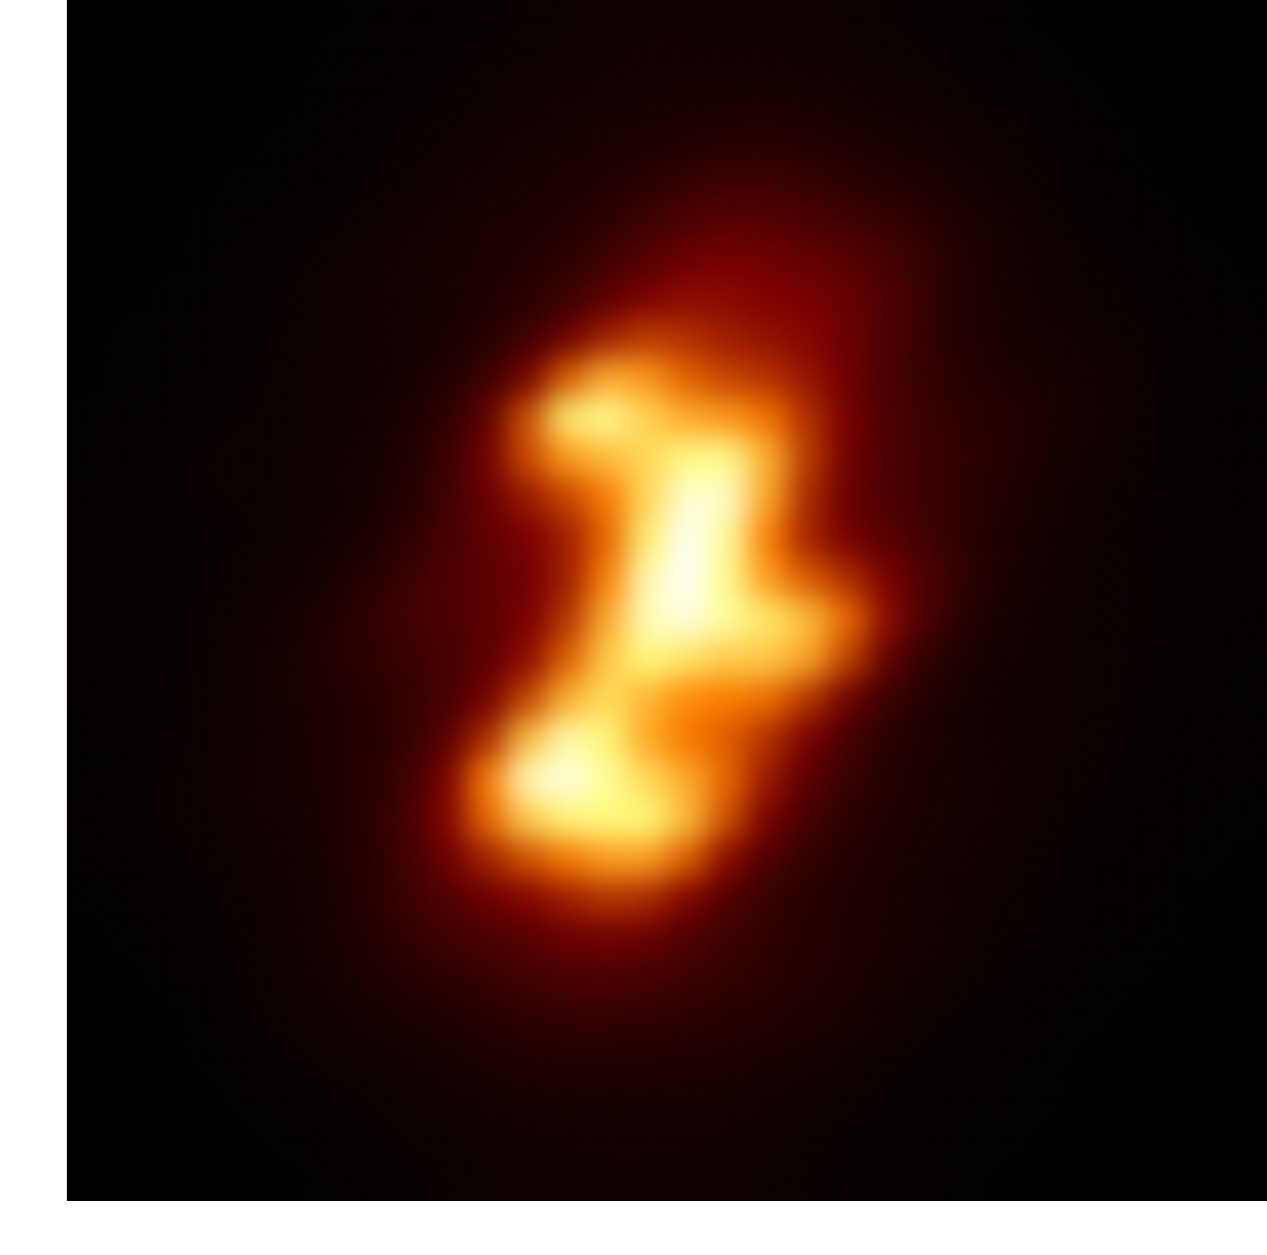} &
			\includegraphics[height=0.12\linewidth]{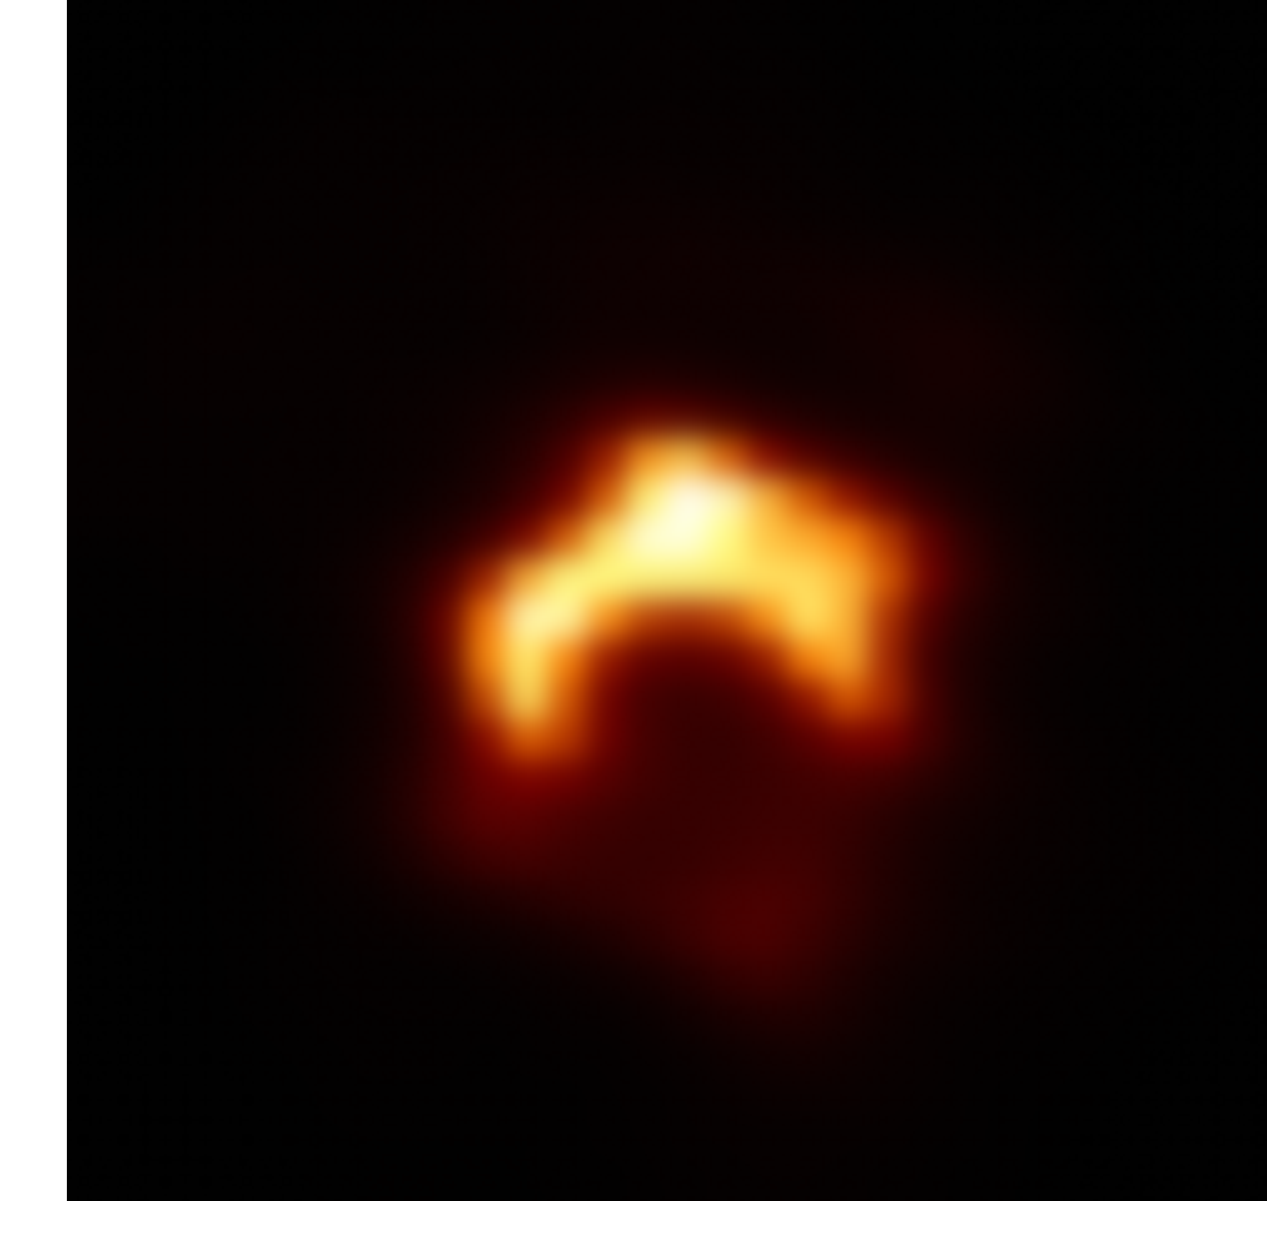} &
			\includegraphics[height=0.12\linewidth]{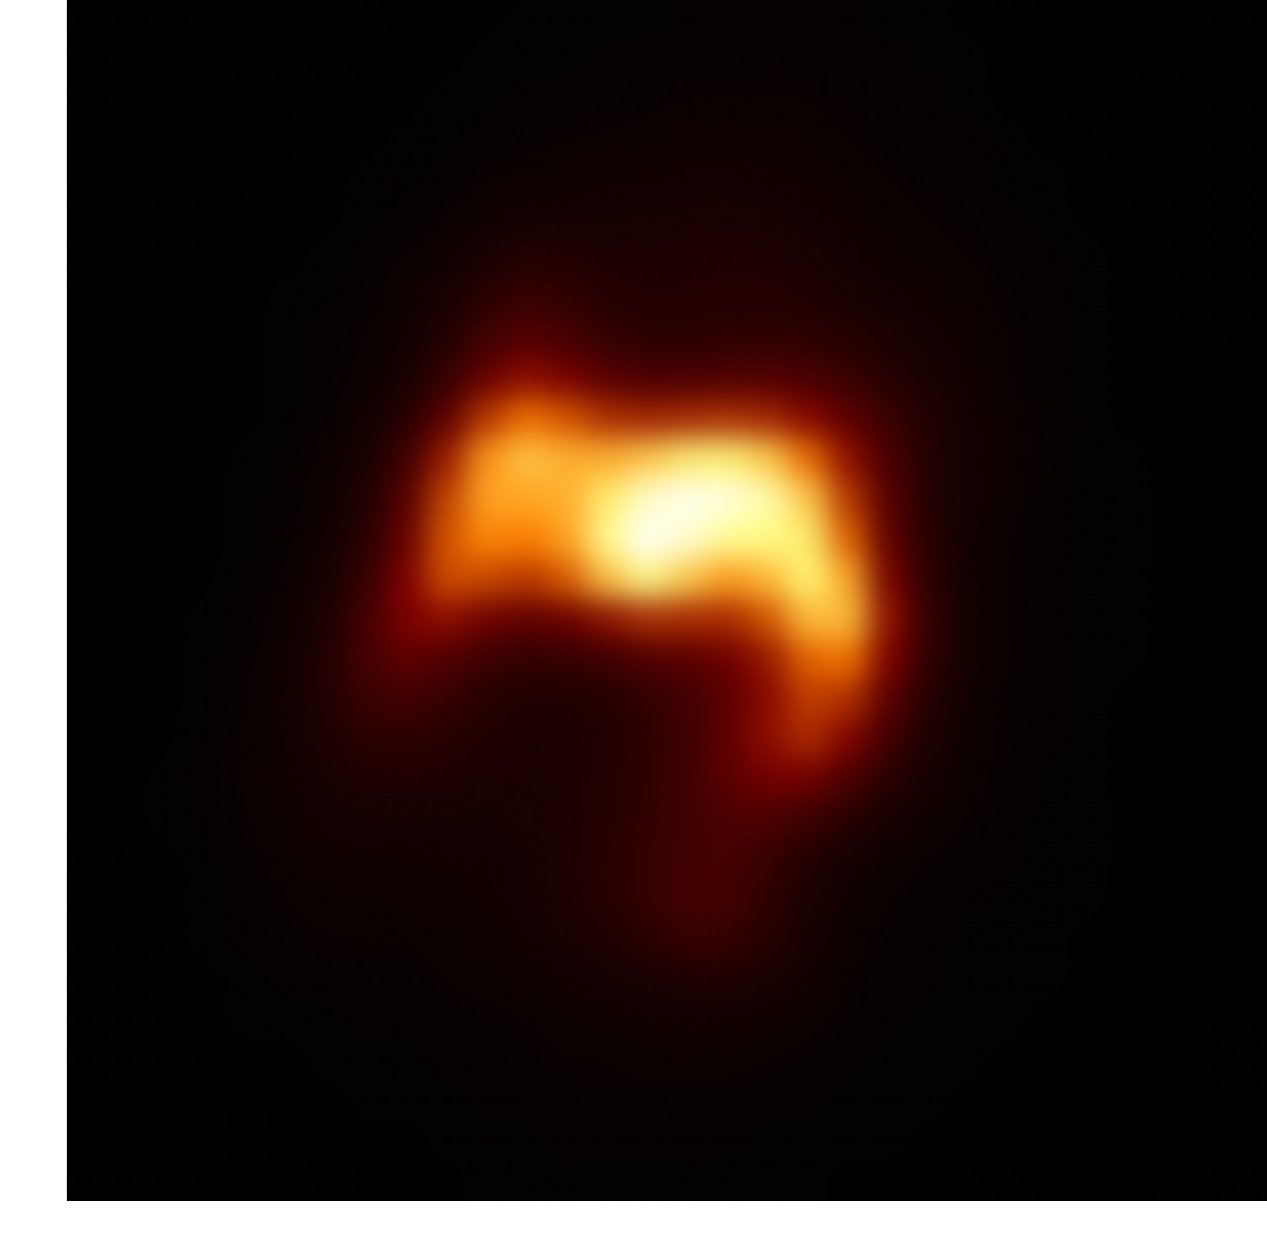} &
			\includegraphics[height=0.12\linewidth]{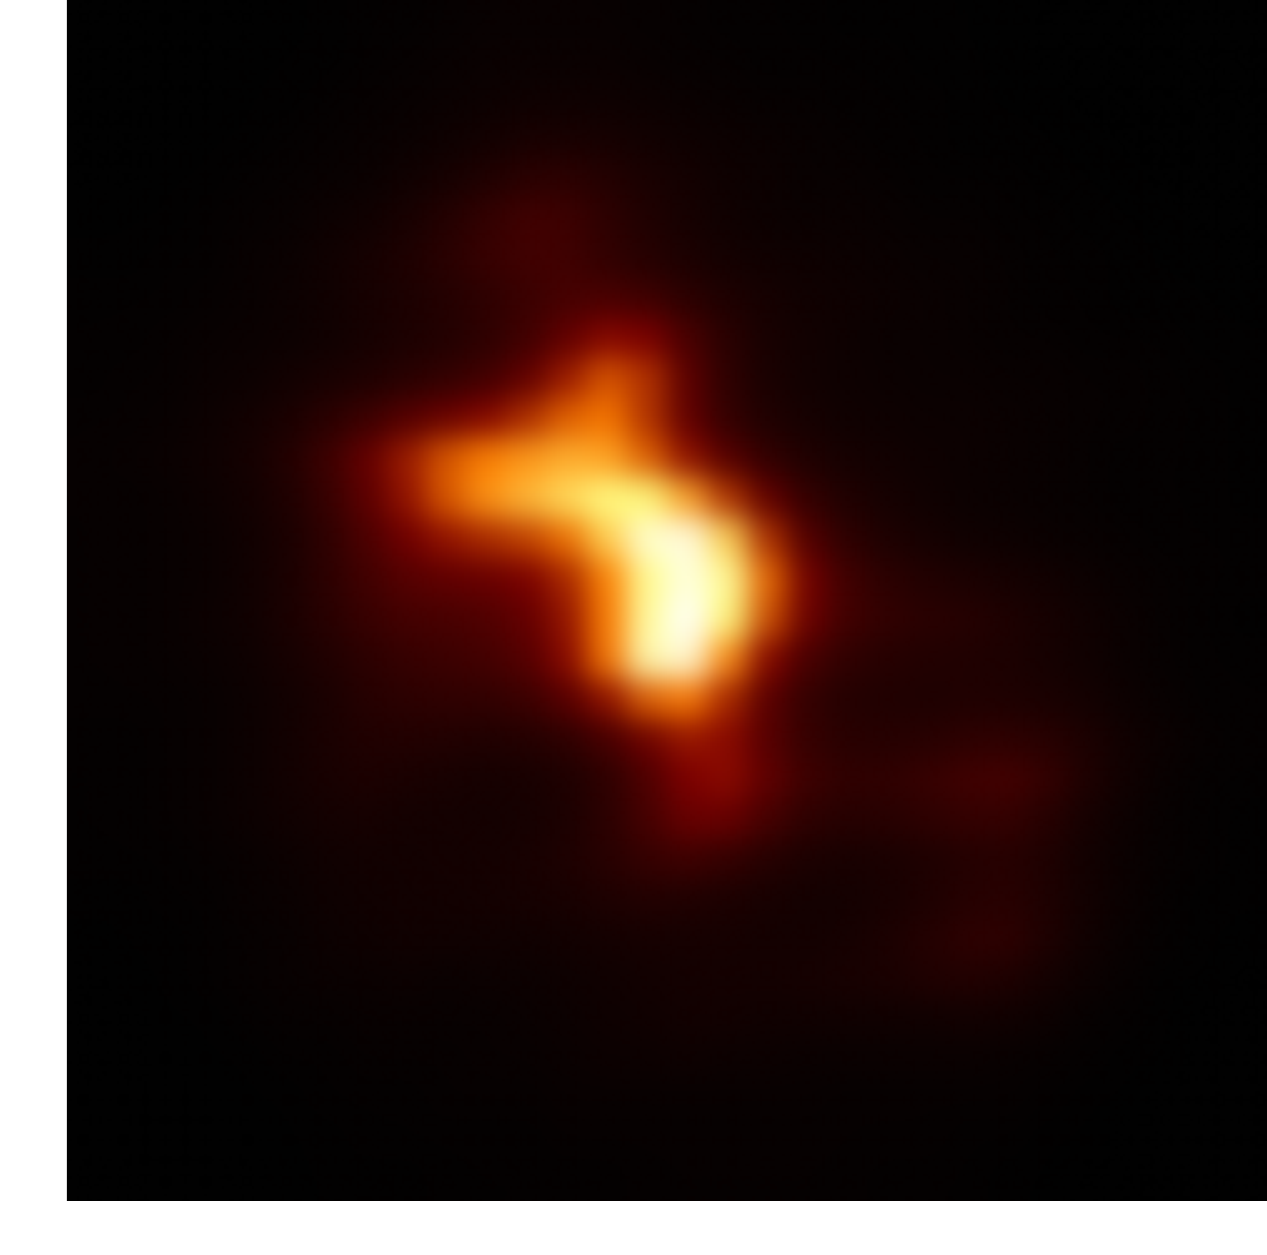} &
			\includegraphics[height=0.12\linewidth]{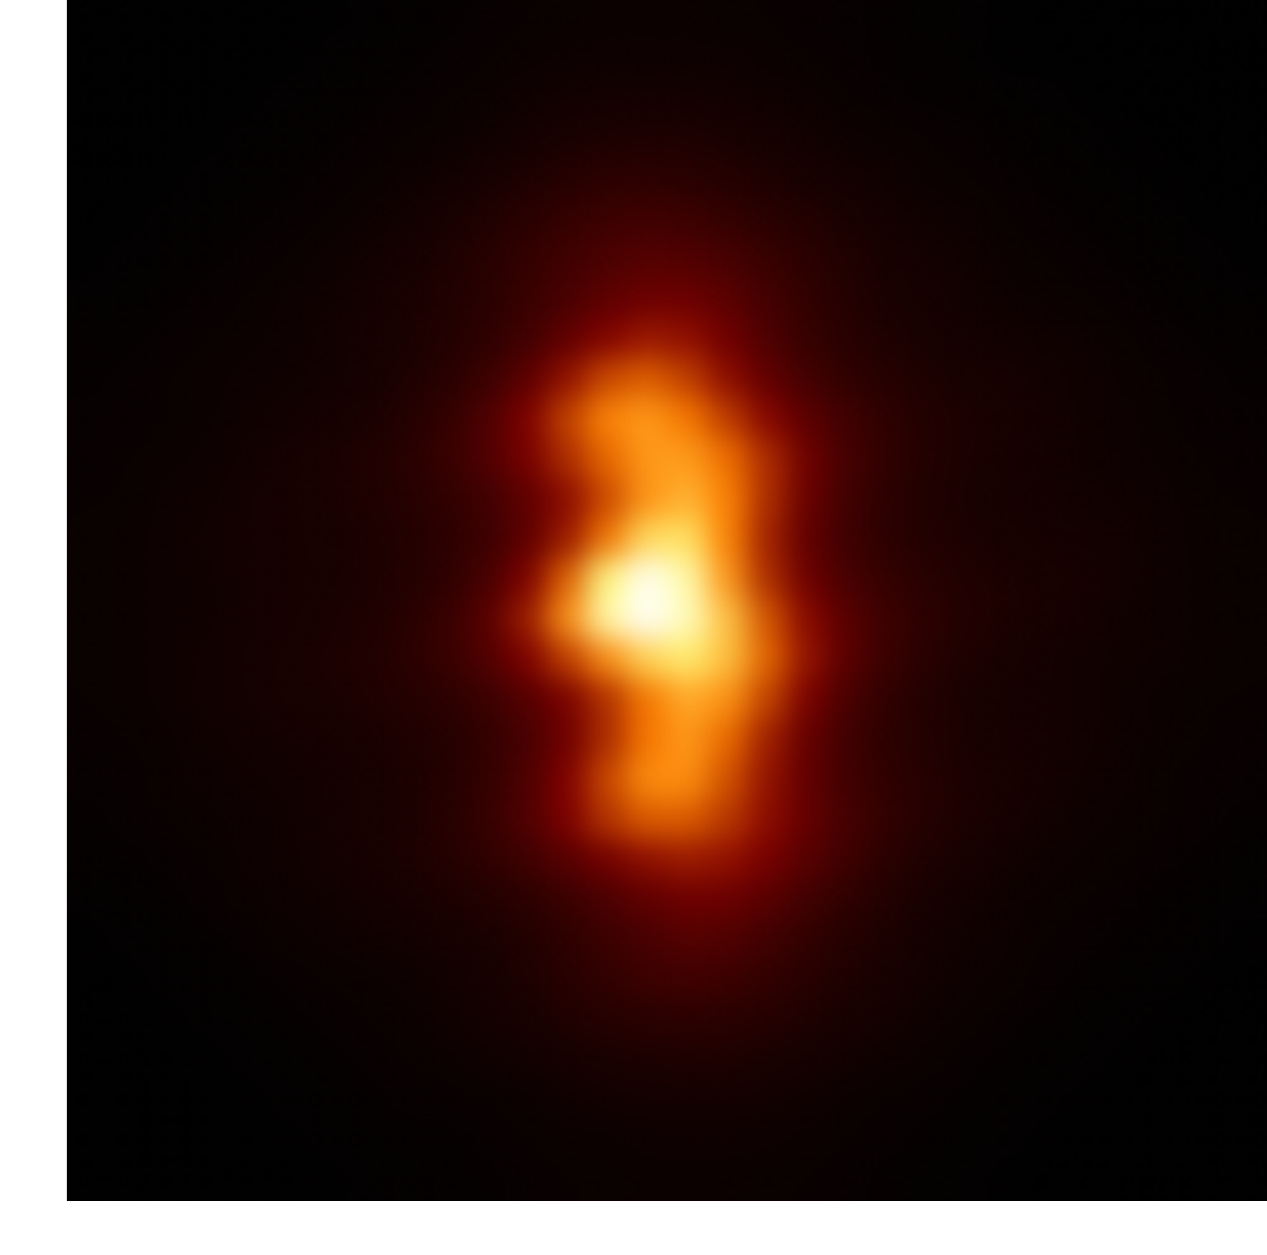} 
			\\          
			&\vspace{-.1in} &&&&&&\\
			\multirow{1}{*}[0.7in]{ \rotatebox[origin=t]{90}{  \specialcell{ \small{\textsf{StarWarps:}} \\  \small{\textsf{No Warp}}}  }}
			&
			{{\includegraphics[height=0.12\linewidth]{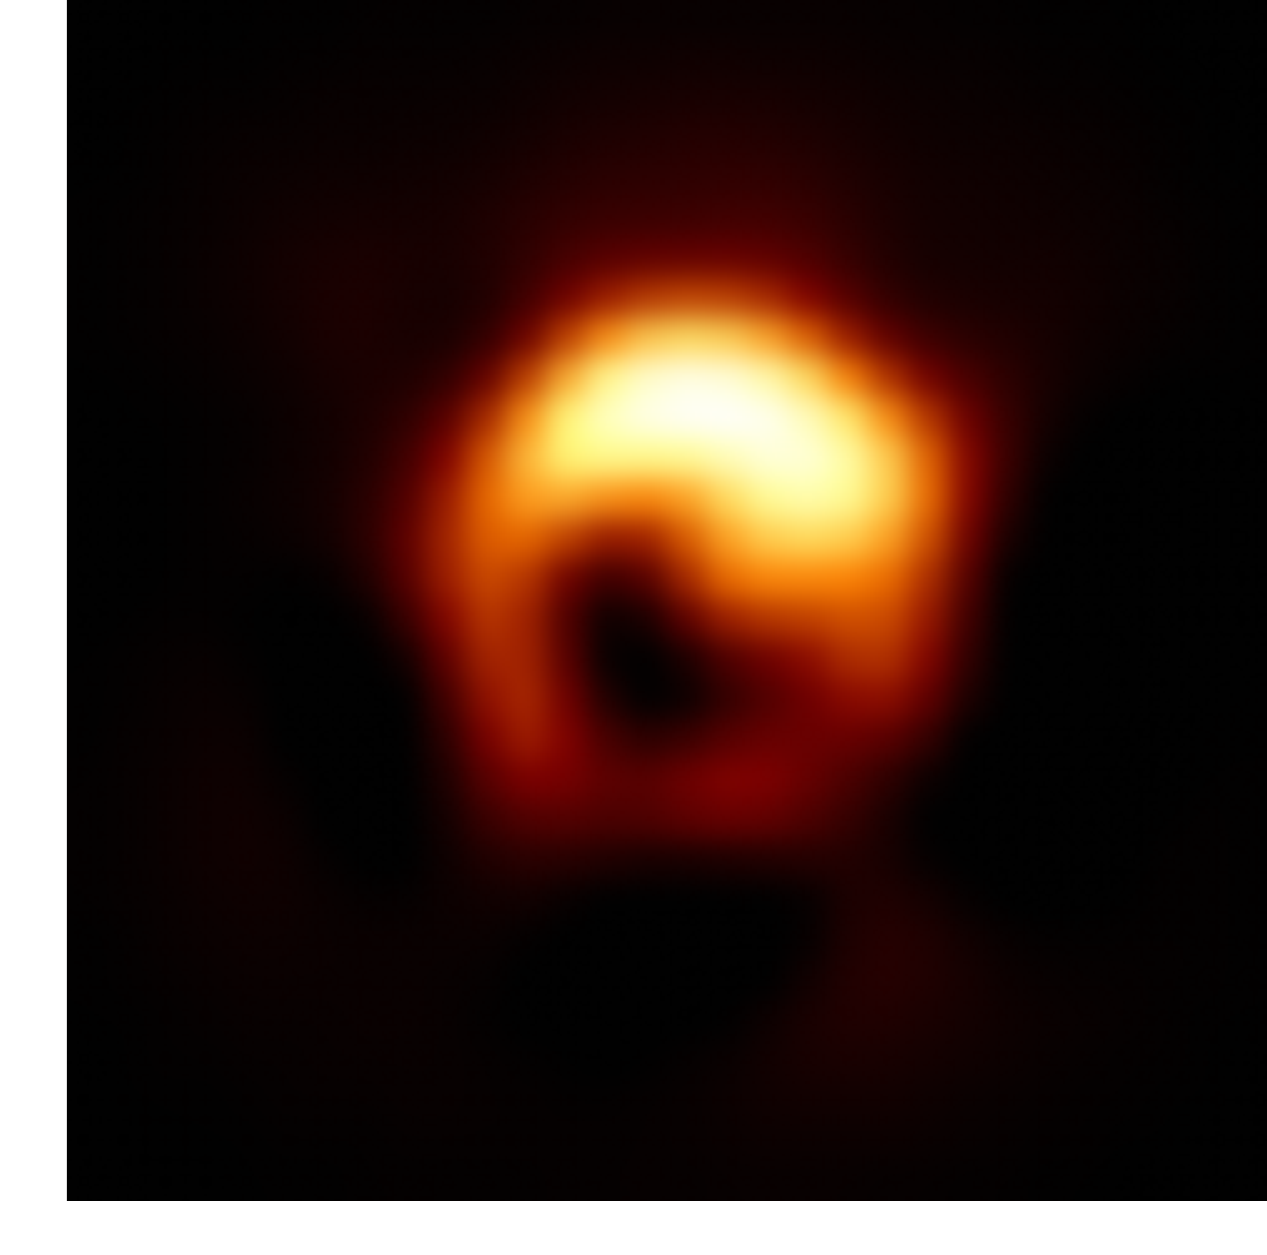}} } &
			\includegraphics[height=0.12\linewidth]{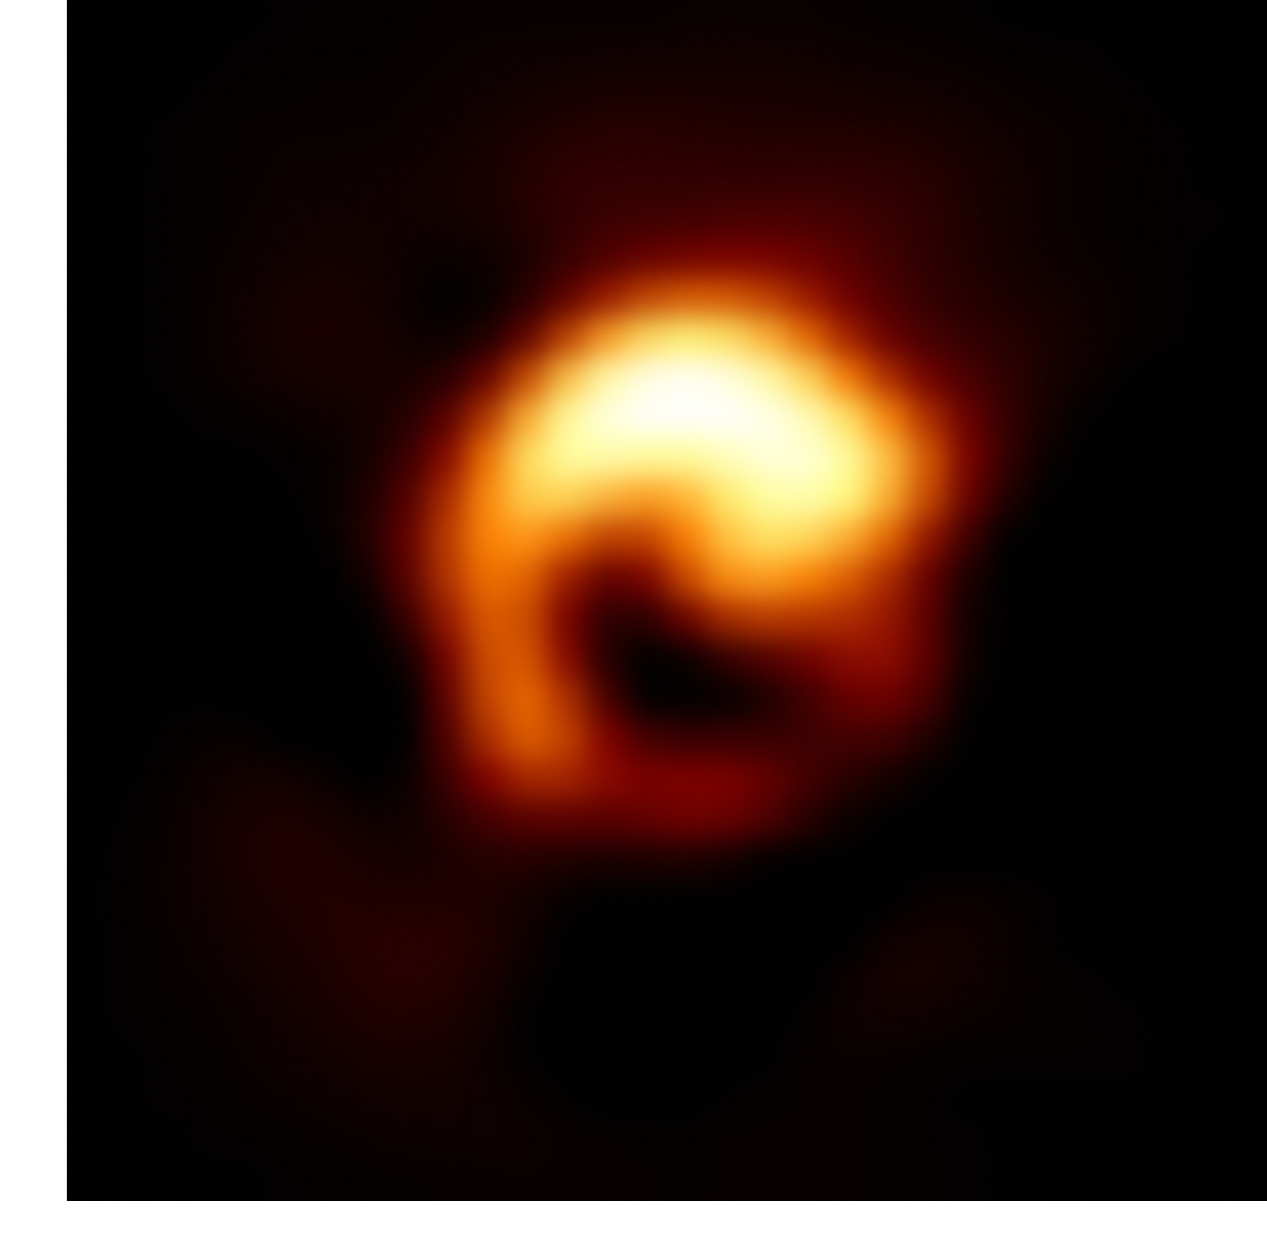} &
			\includegraphics[height=0.12\linewidth]{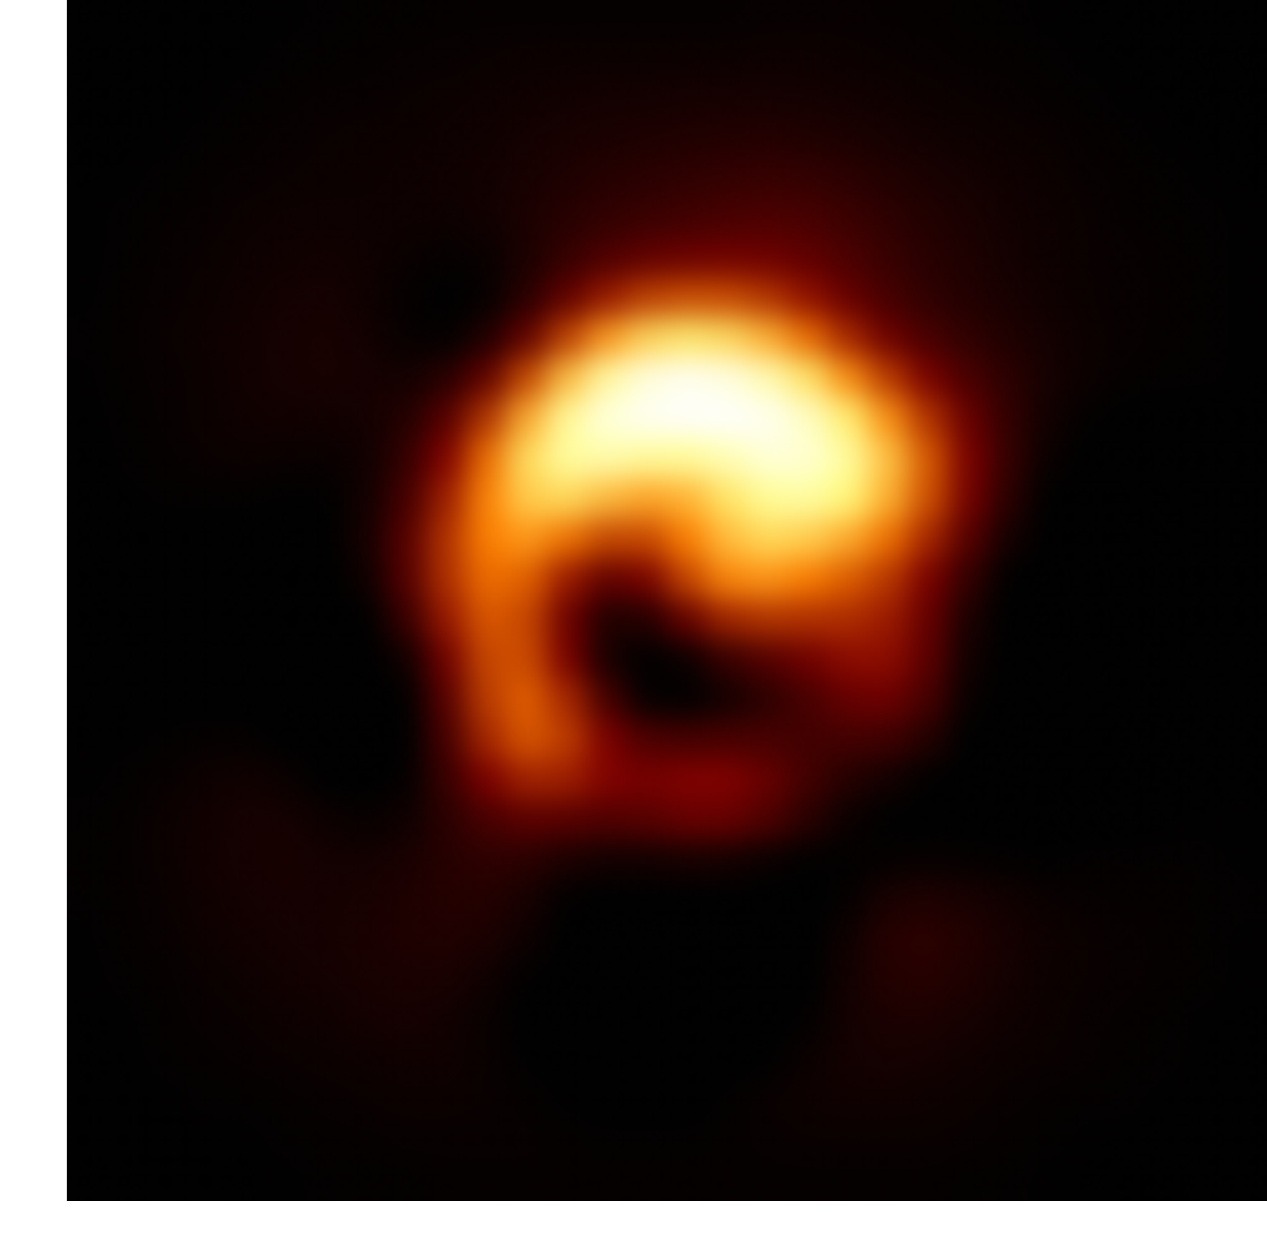} &
			\includegraphics[height=0.12\linewidth]{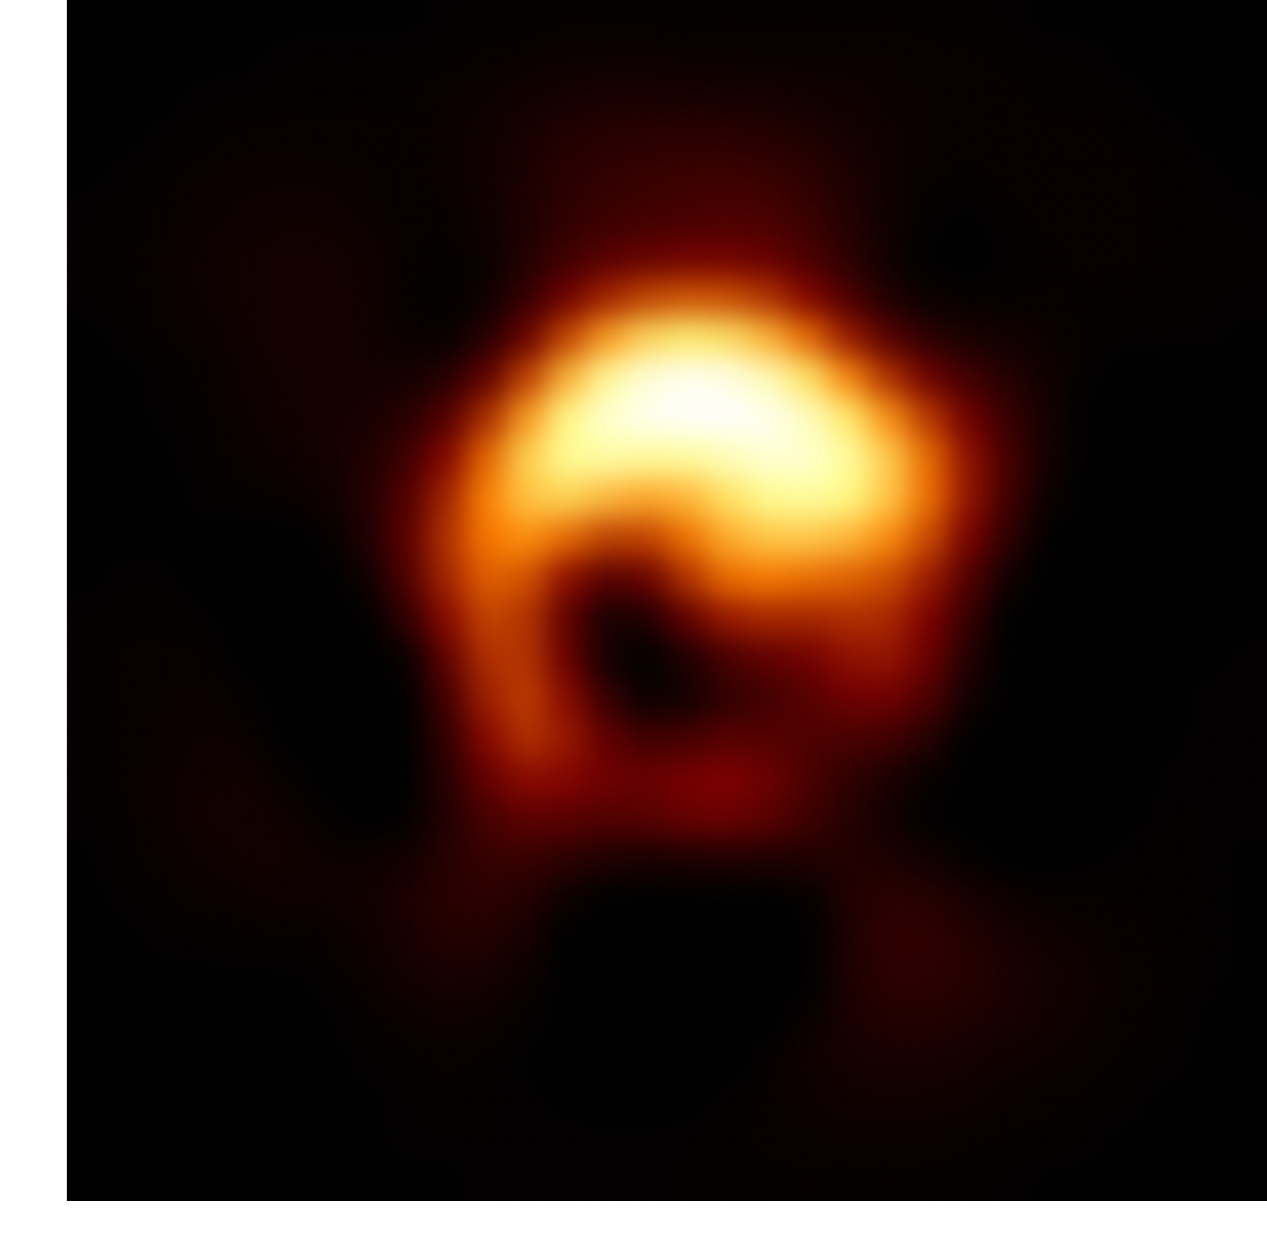} &
			\includegraphics[height=0.12\linewidth]{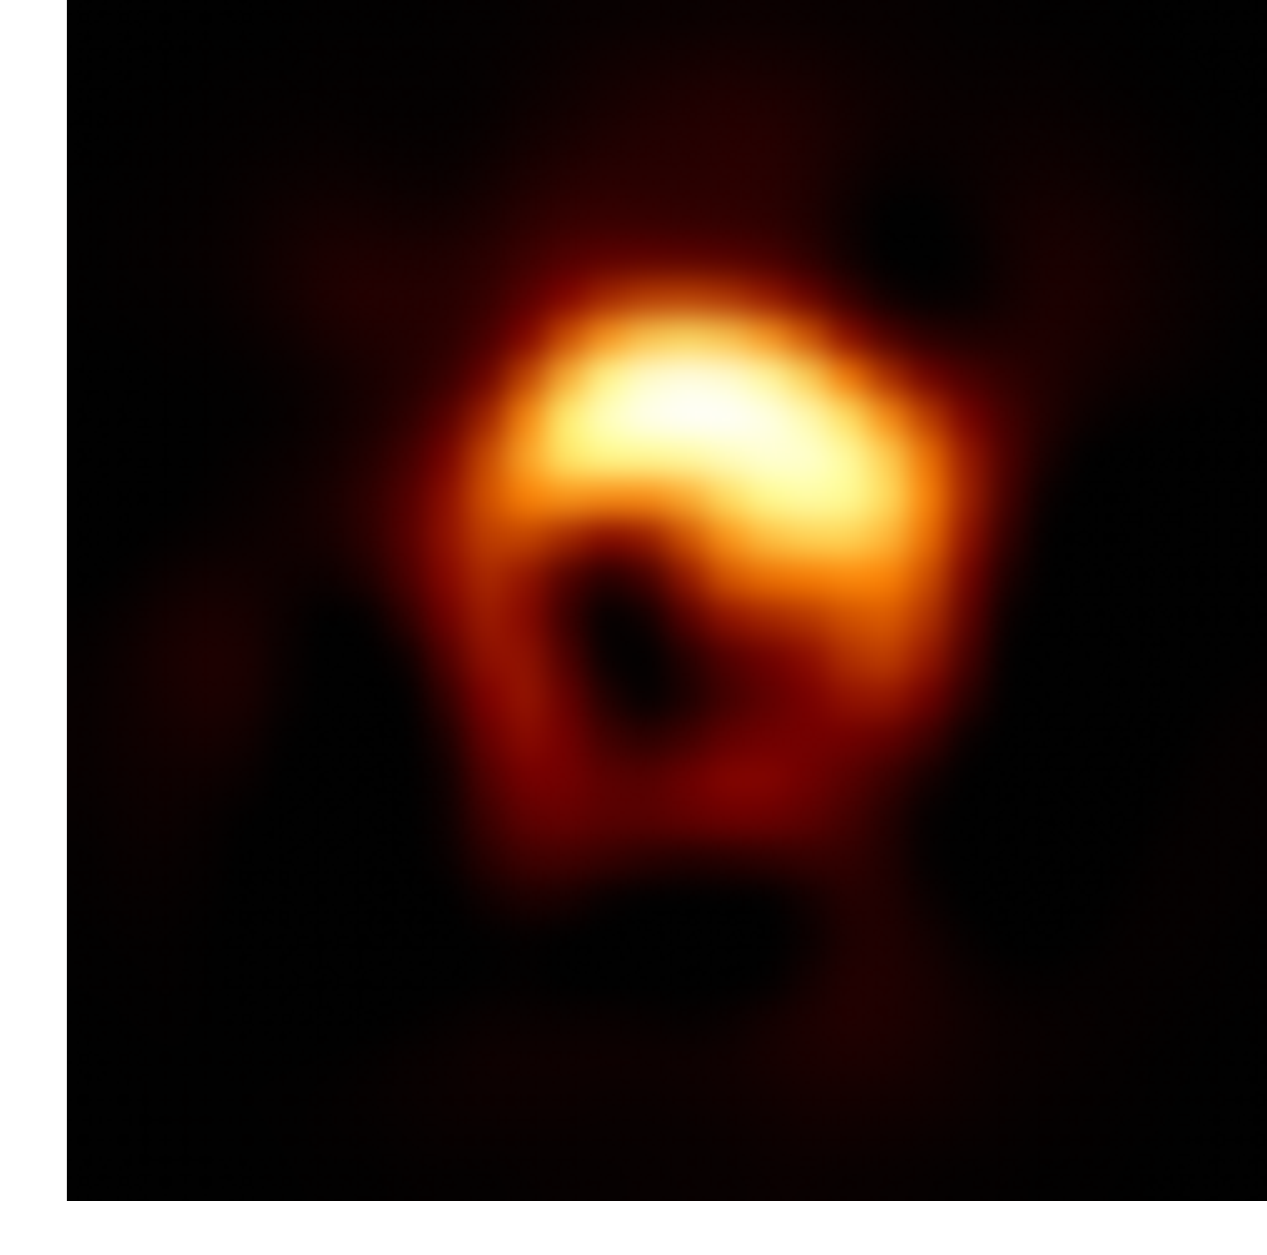} &
			\includegraphics[height=0.12\linewidth]{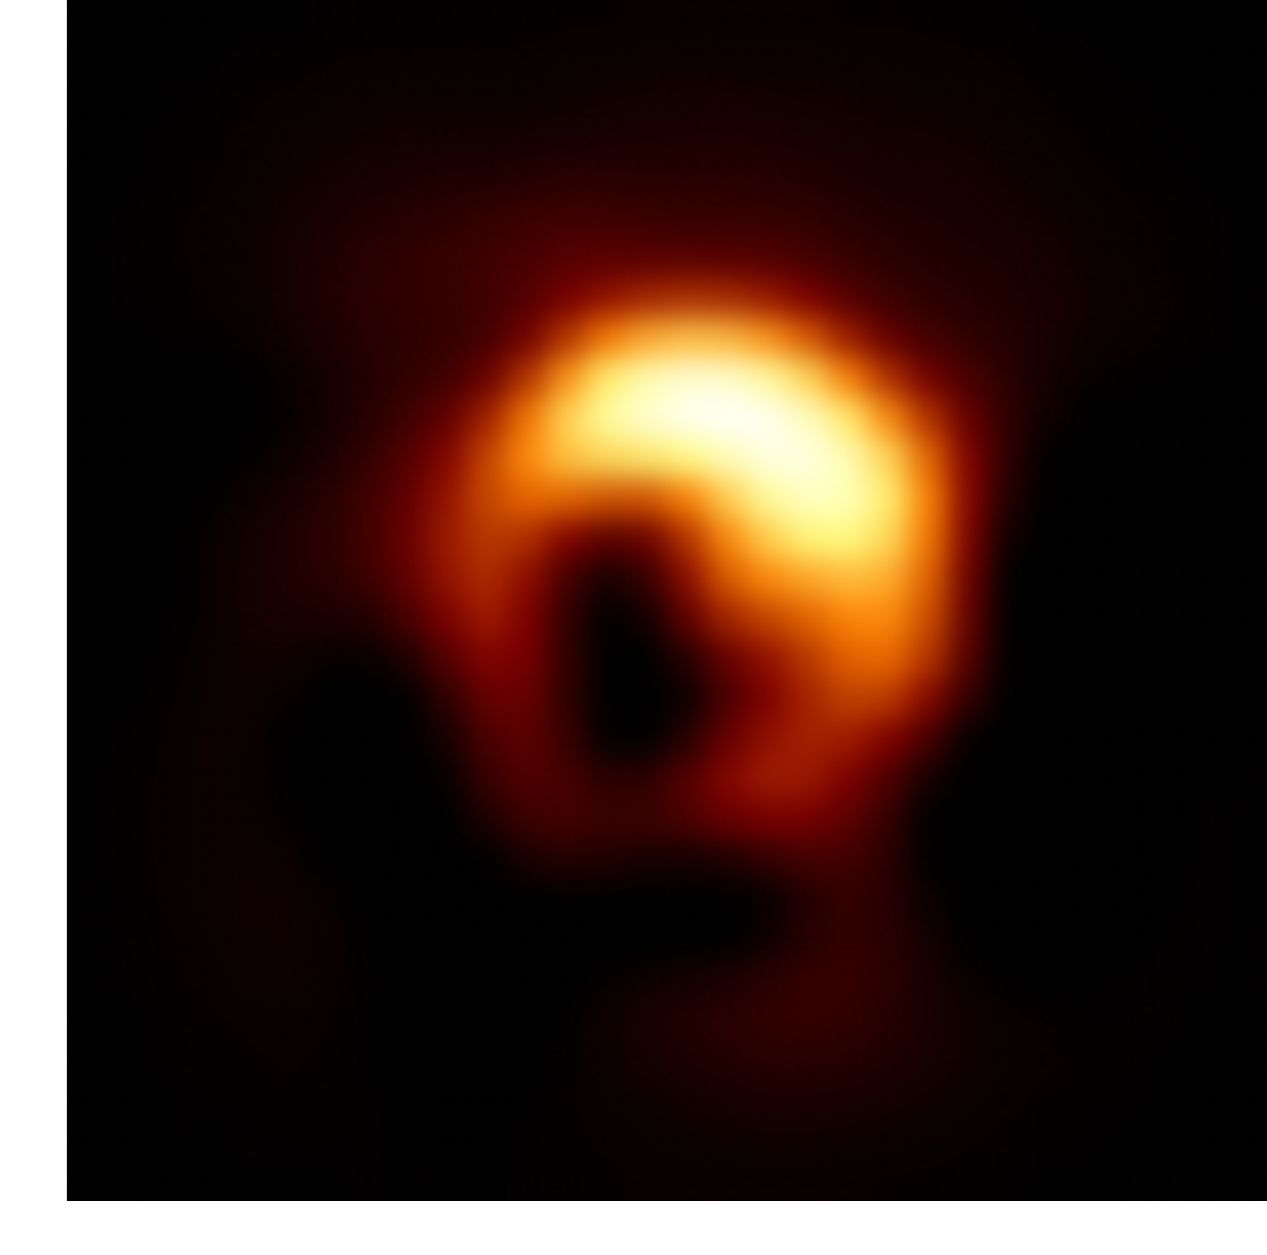} &
			\includegraphics[height=0.12\linewidth]{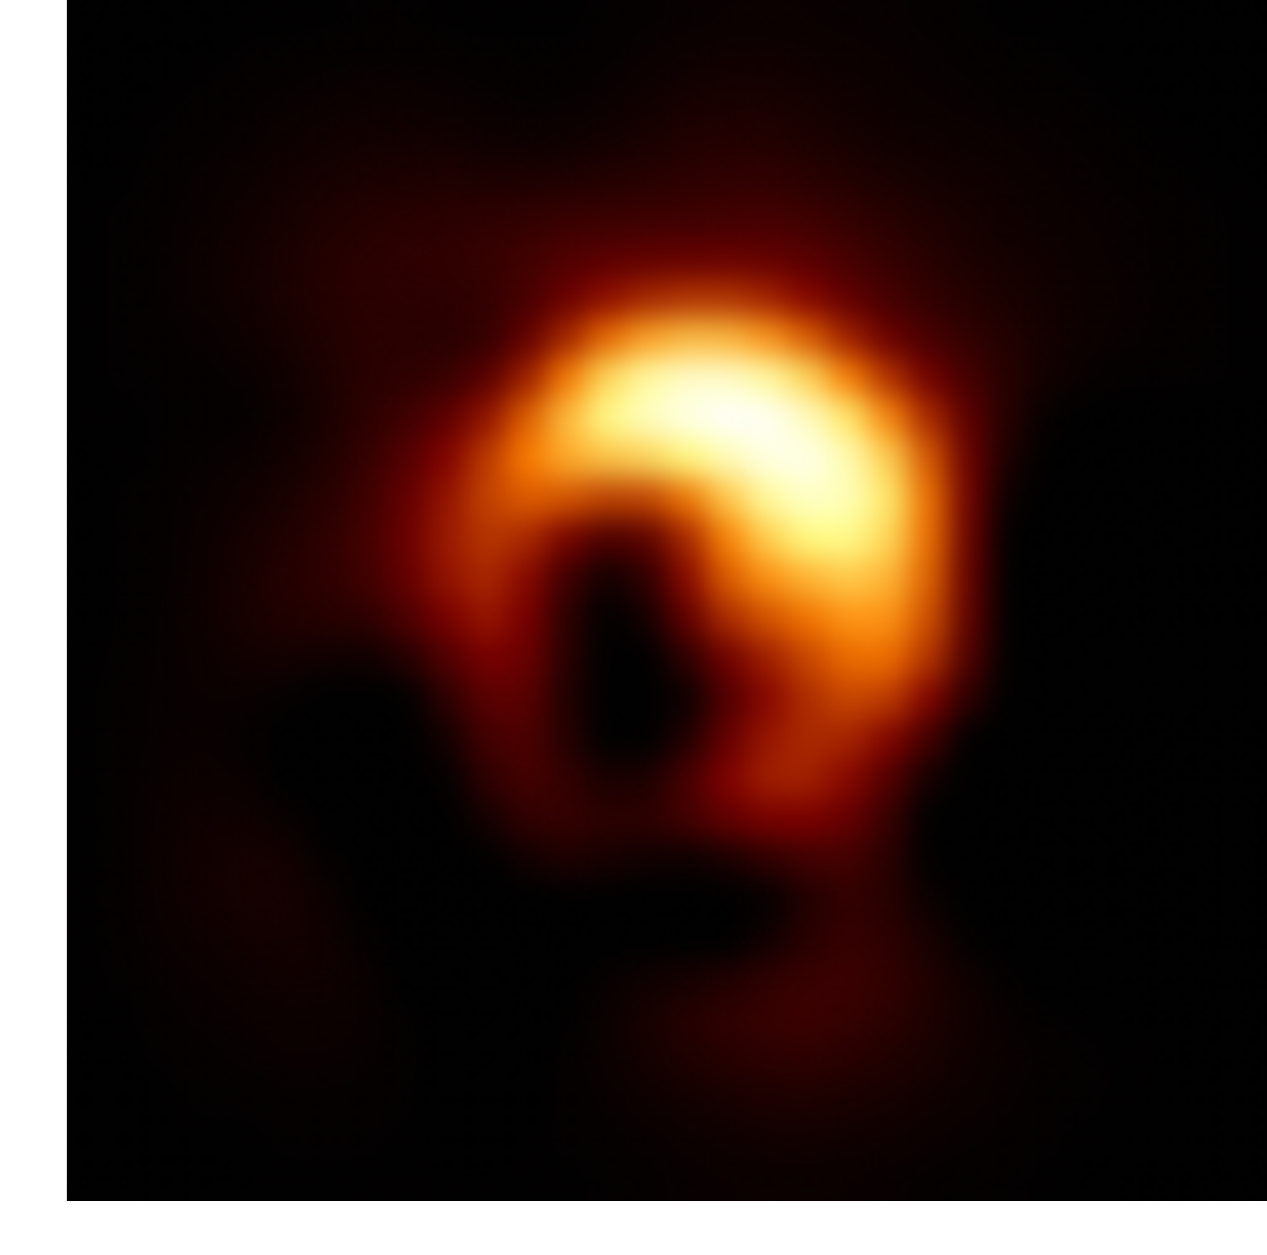} 
			\\          
			&\vspace{-.1in} &&&&&&\\
			\multirow{1}{*}[0.7in]{ \rotatebox[origin=t]{90}{  \specialcell{ \small{\textsf{StarWarps:}} \\  \small{\textsf{Learn Warp}}}  }}
			&
			%{{\includegraphics[height=0.12\linewidth]{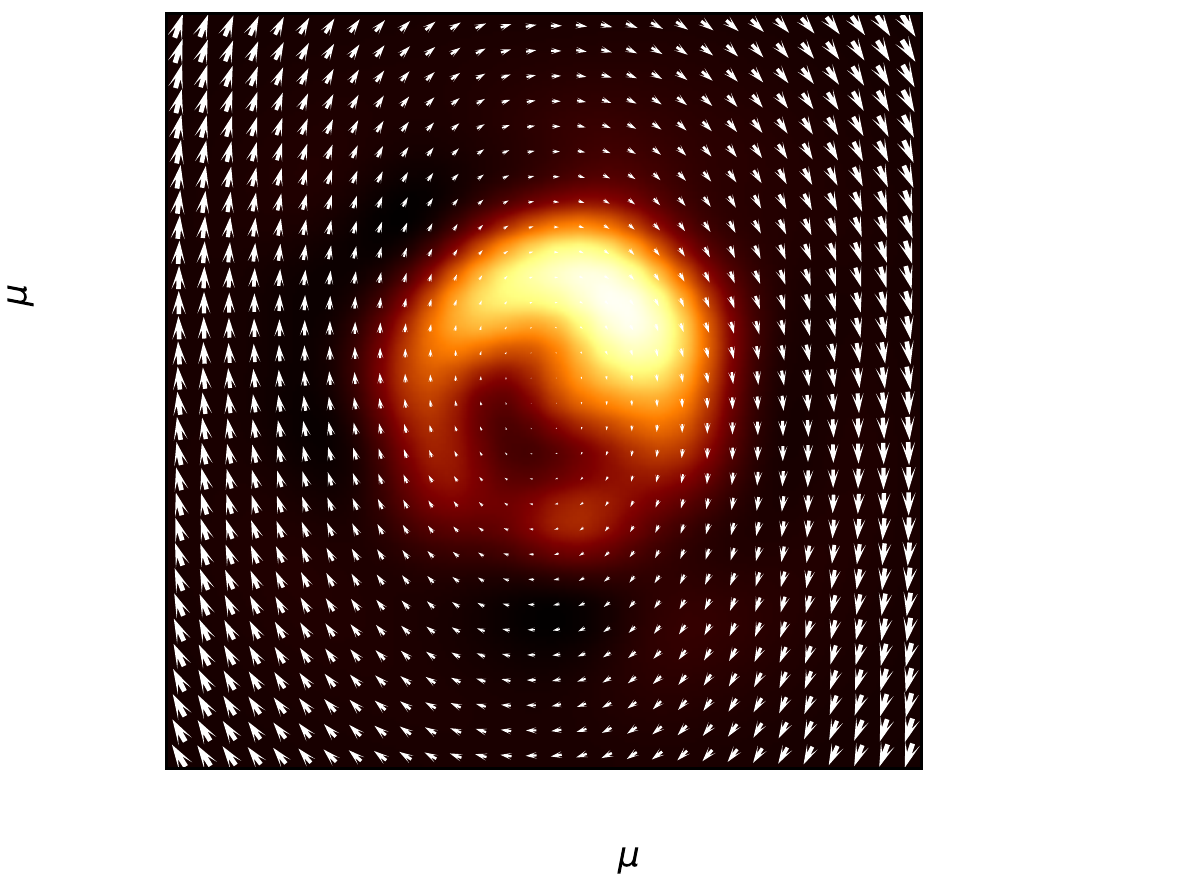}} }
			%\hspace{0.02in} 
			{{\includegraphics[height=0.12\linewidth]{figures/recov_flowfields/rot30_bis/flow_noaxis.pdf}} } &
			\includegraphics[height=0.12\linewidth]{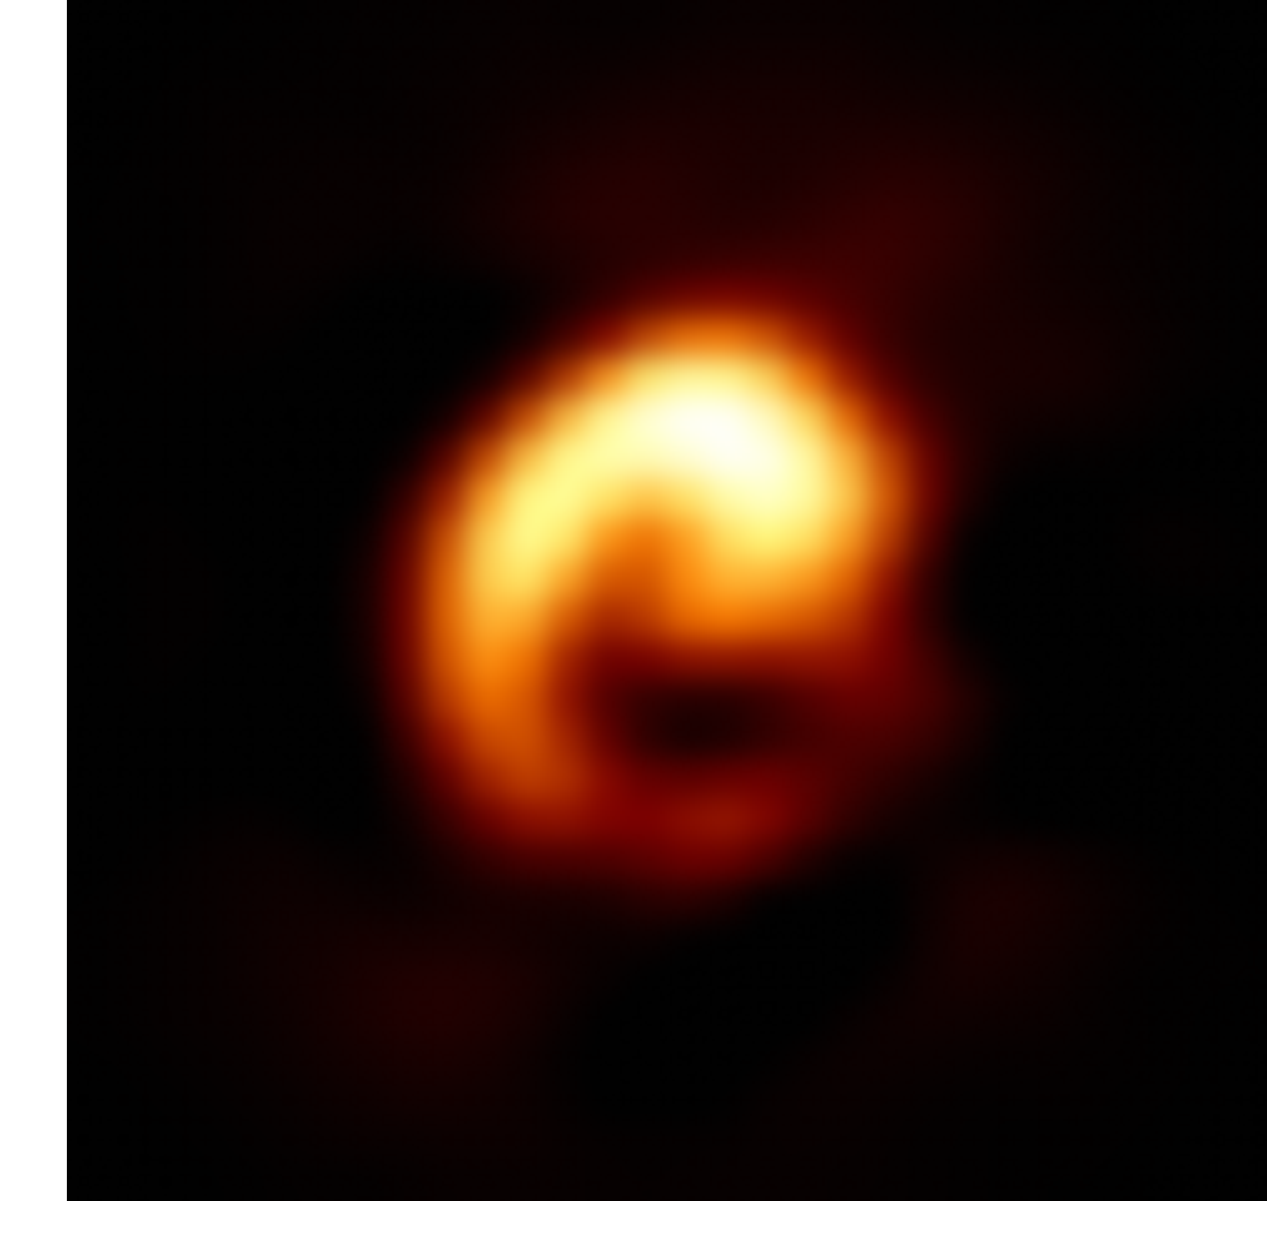} &
			\includegraphics[height=0.12\linewidth]{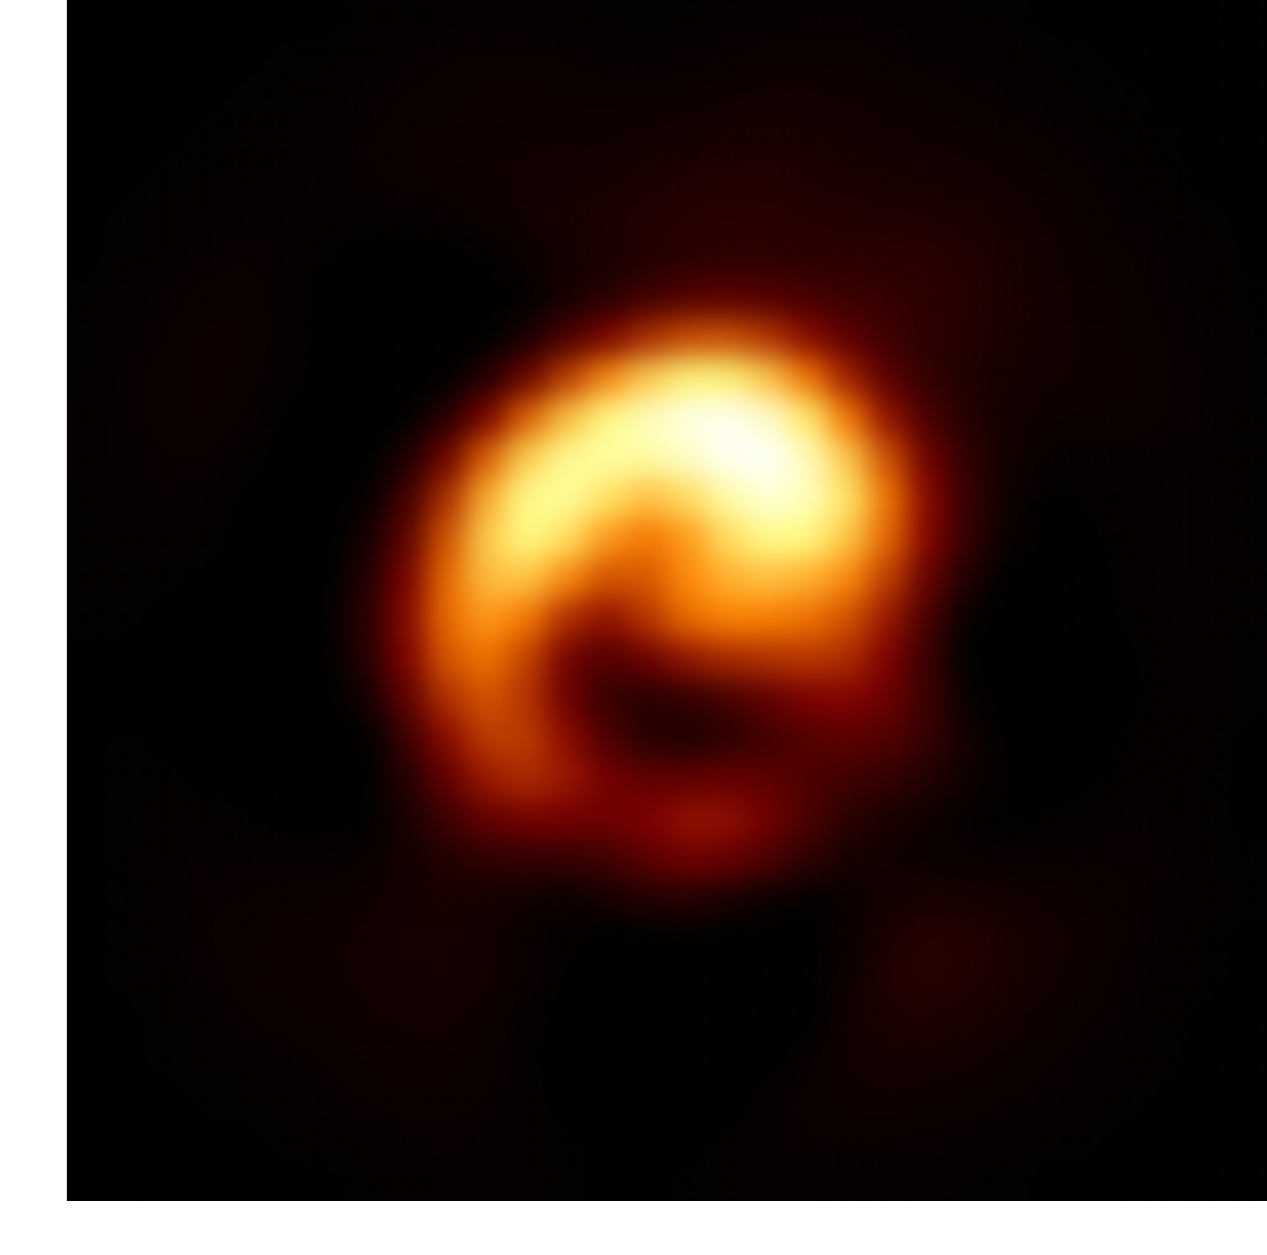} &
			\includegraphics[height=0.12\linewidth]{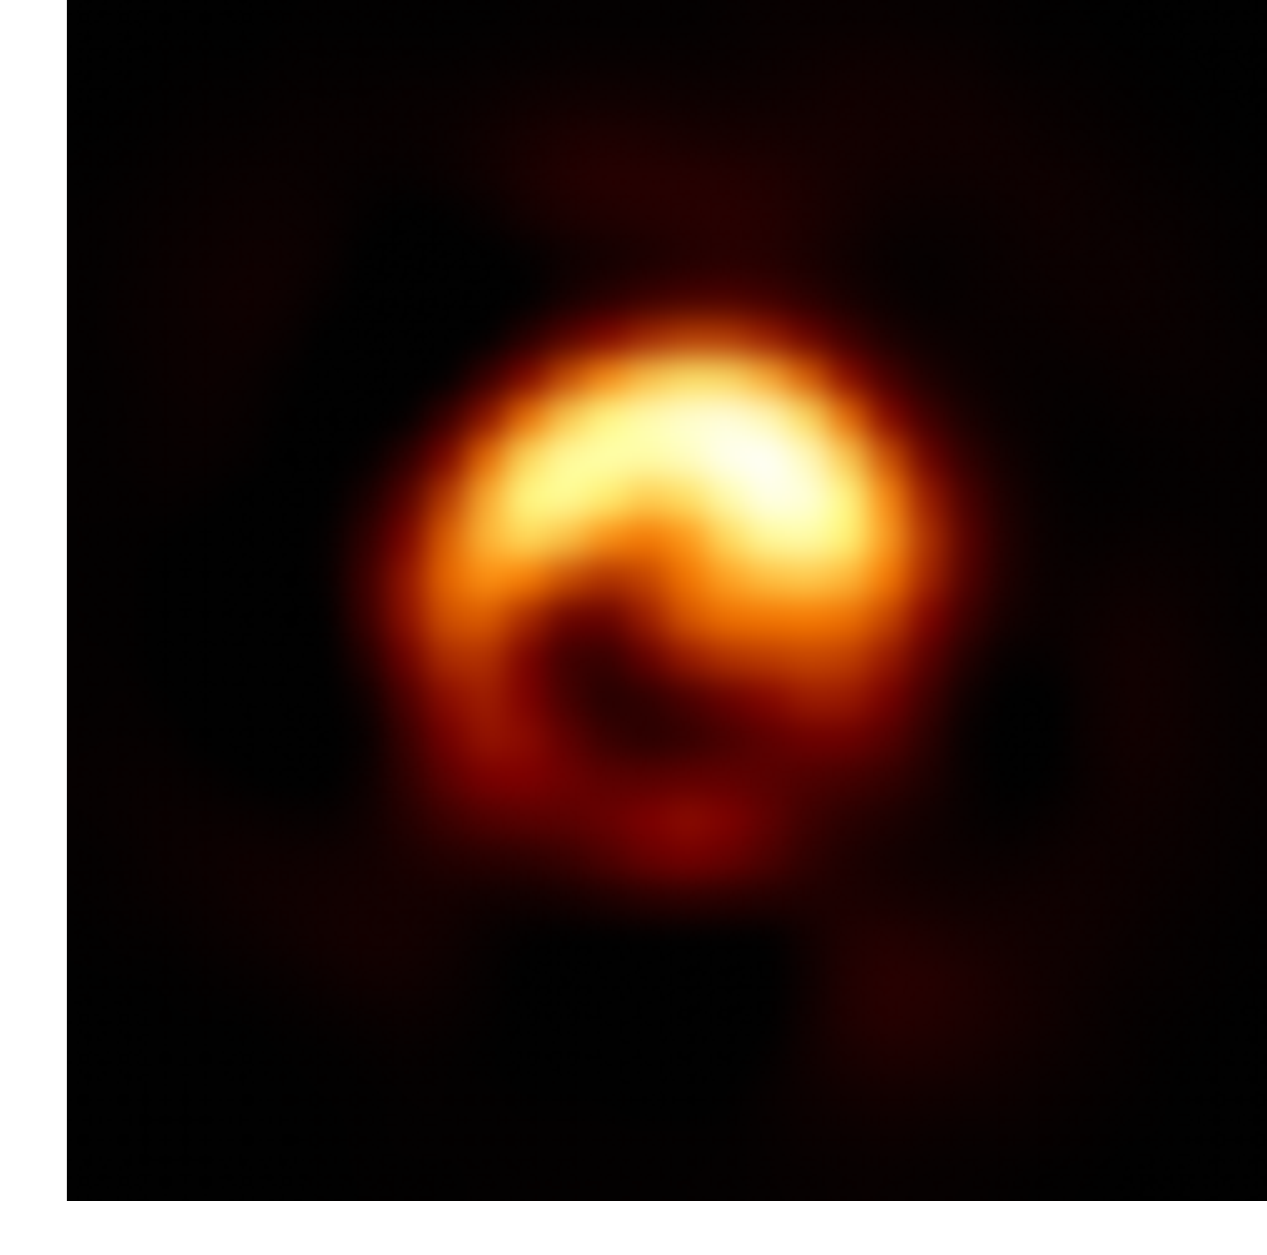} &
			\includegraphics[height=0.12\linewidth]{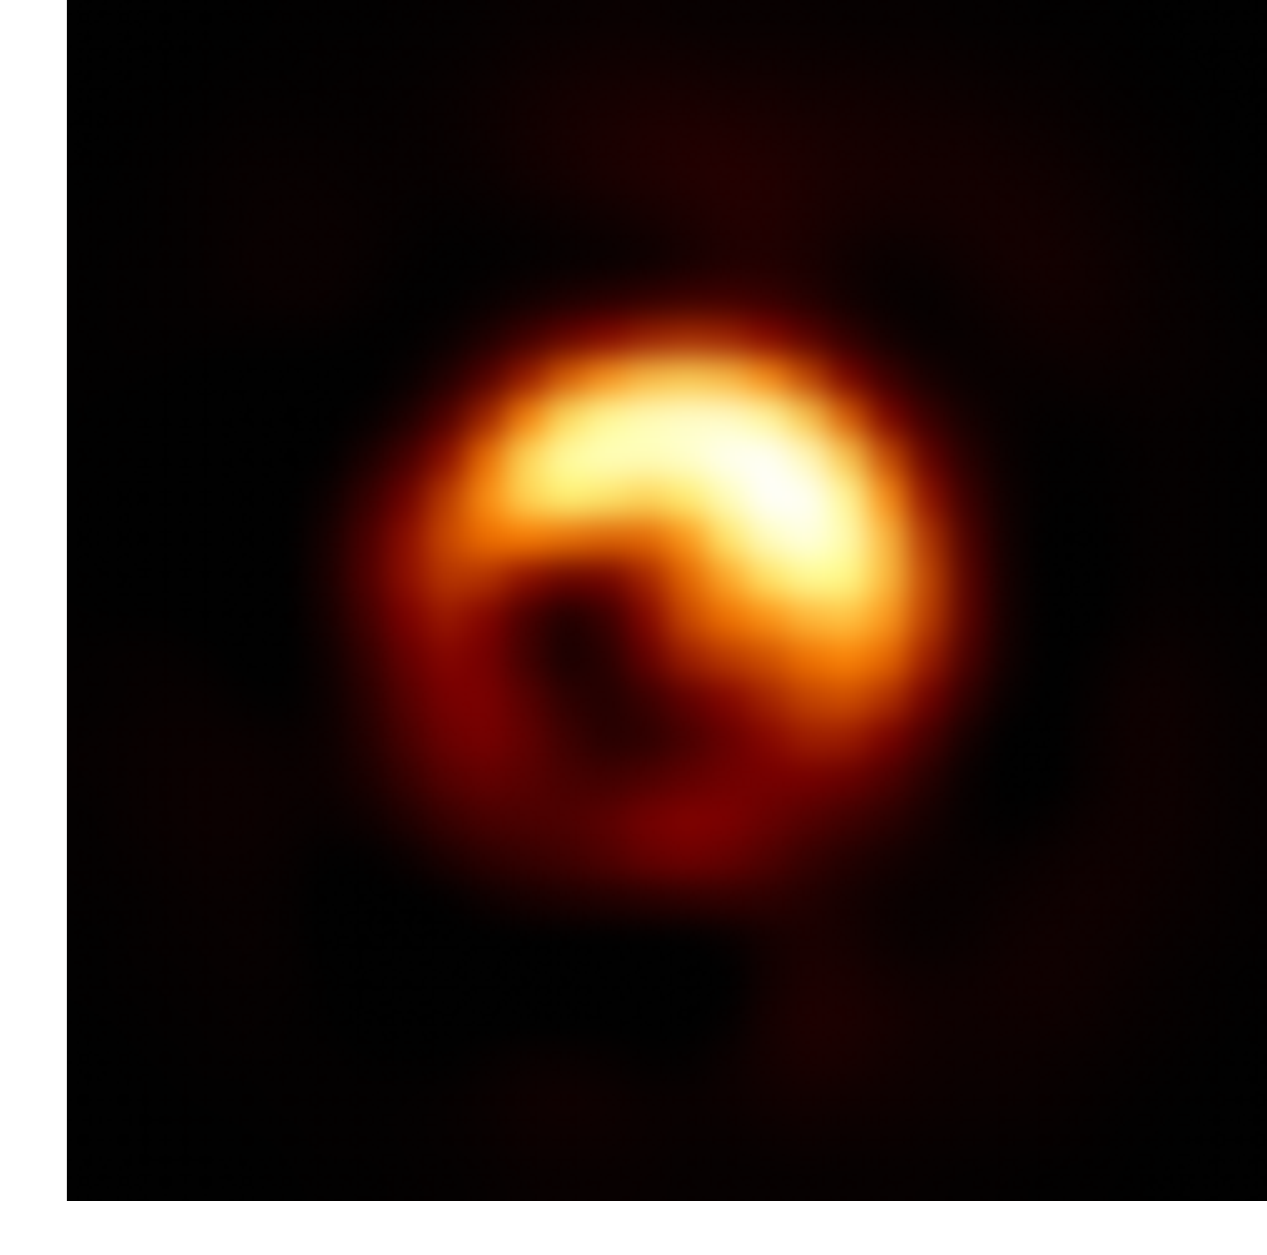} &
			\includegraphics[height=0.12\linewidth]{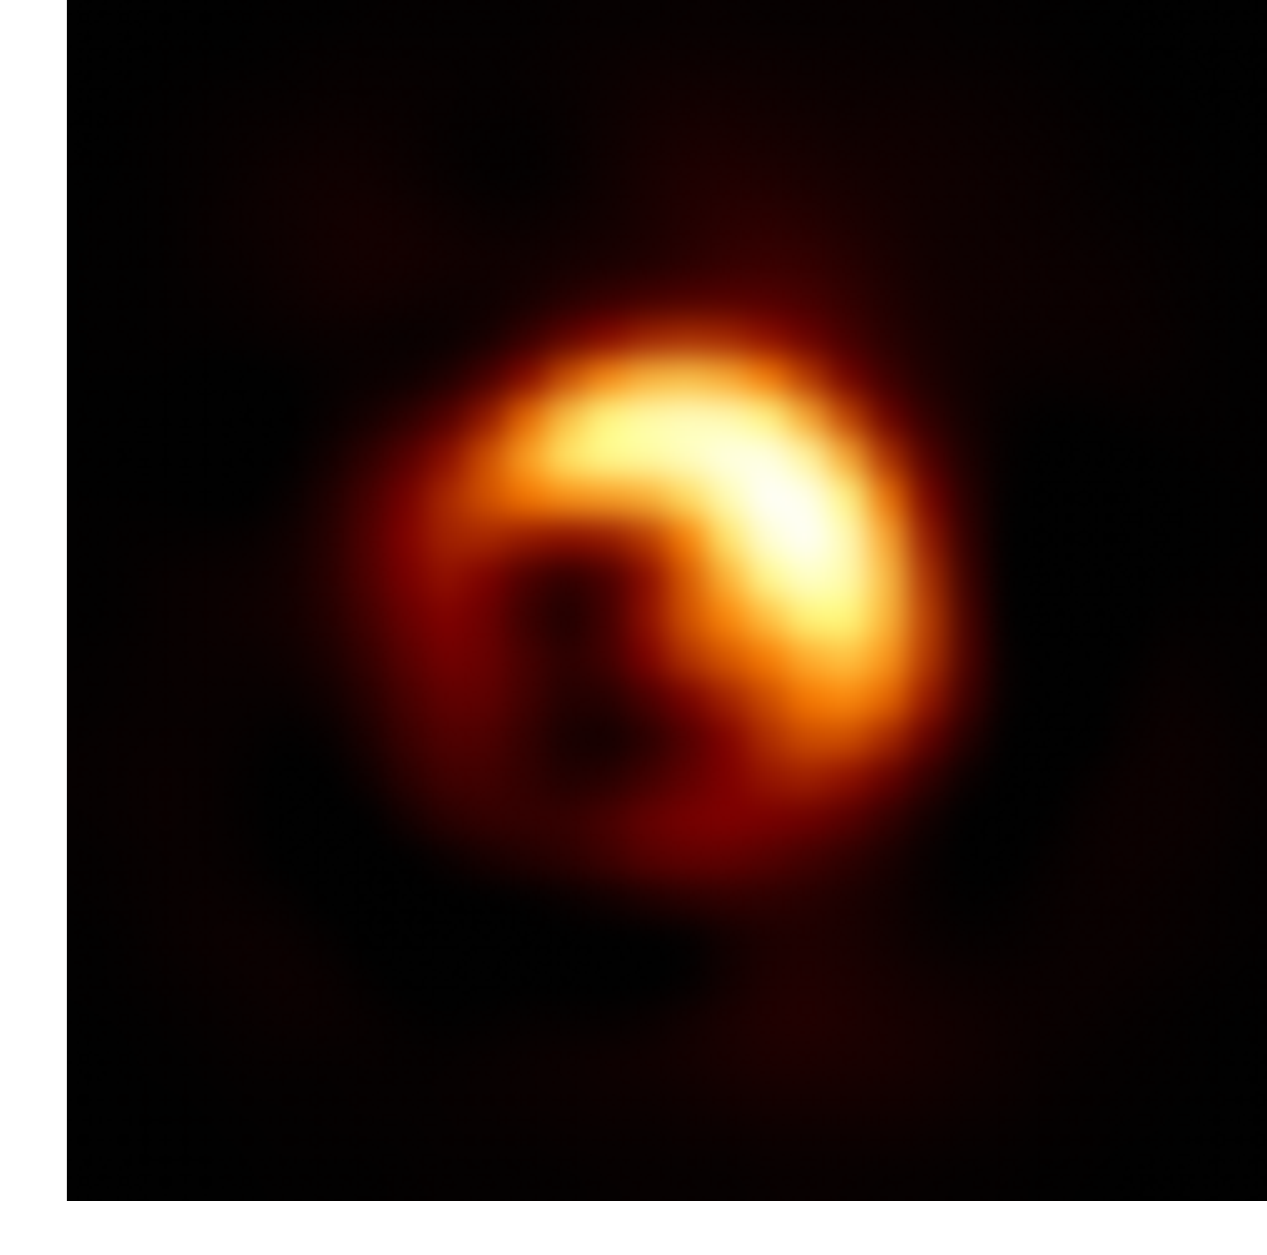} &
			\includegraphics[height=0.12\linewidth]{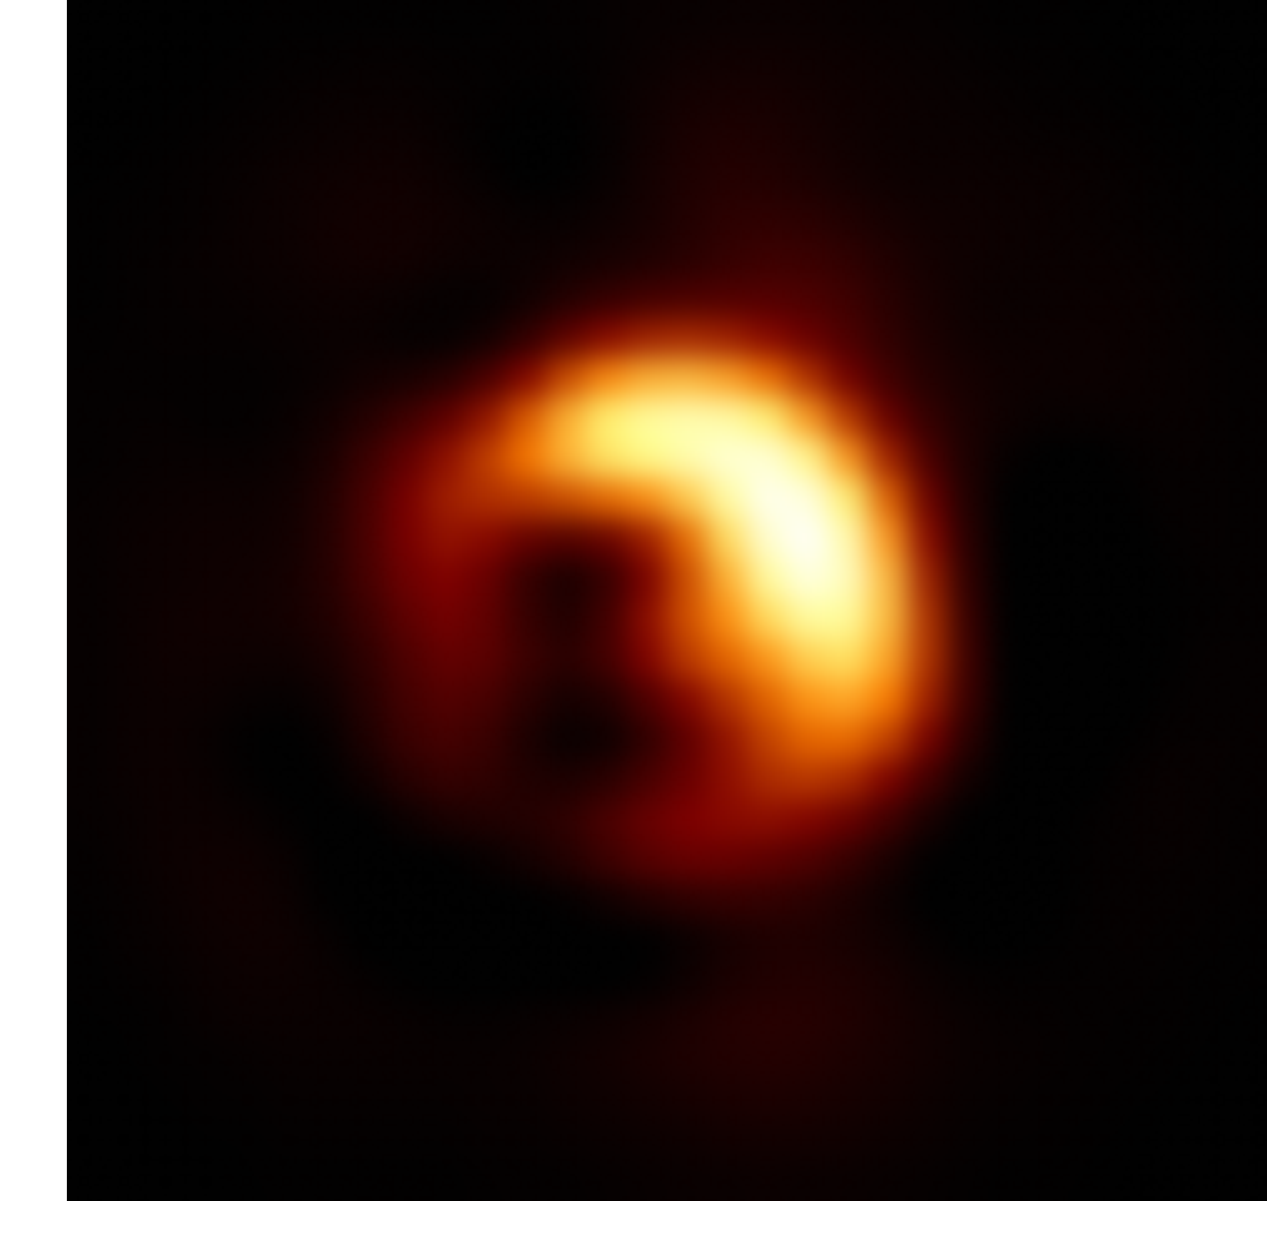}  
			%			\\ 
			%			&\vspace{-.1in} &&&&&&\\
			%			\multirow{1}{*}[.5in]{ \rotatebox[origin=t]{90}{\small{\textsf{Flow 2}} }}
			%			&
			%			{{\includegraphics[height=0.12\linewidth]{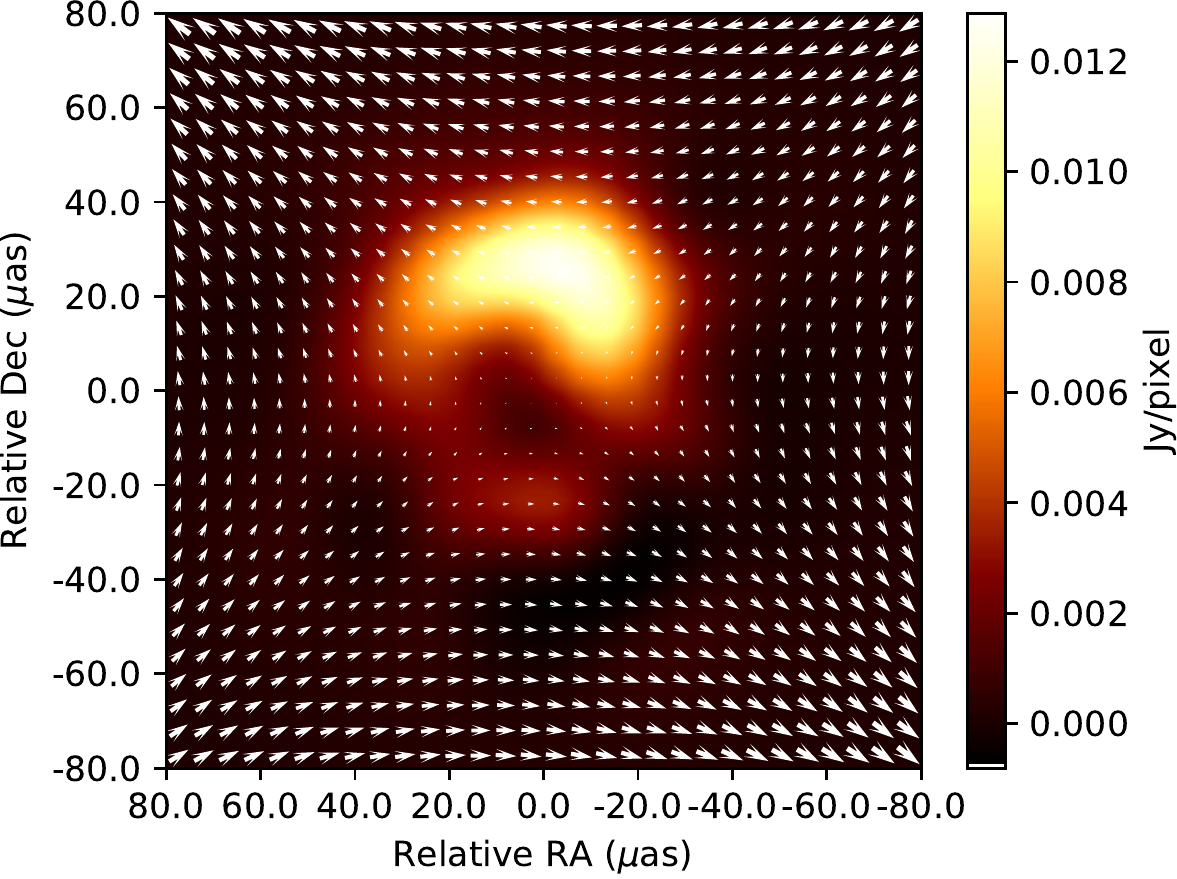}} } &
			%			\includegraphics[height=0.12\linewidth]{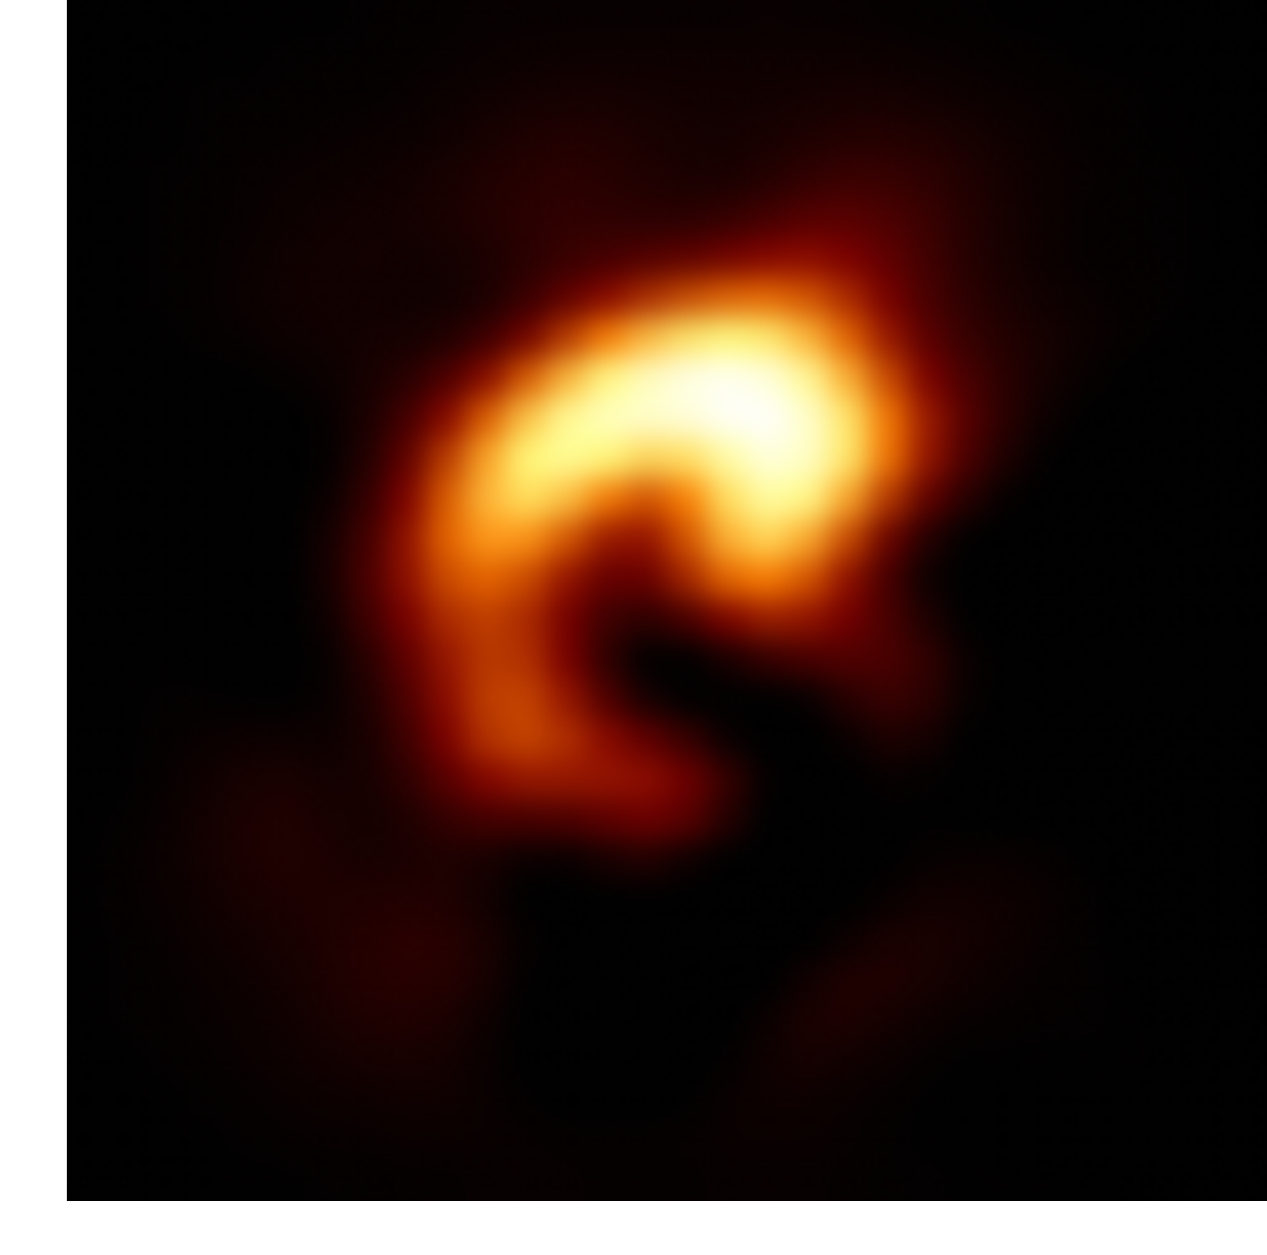} &
			%			\includegraphics[height=0.12\linewidth]{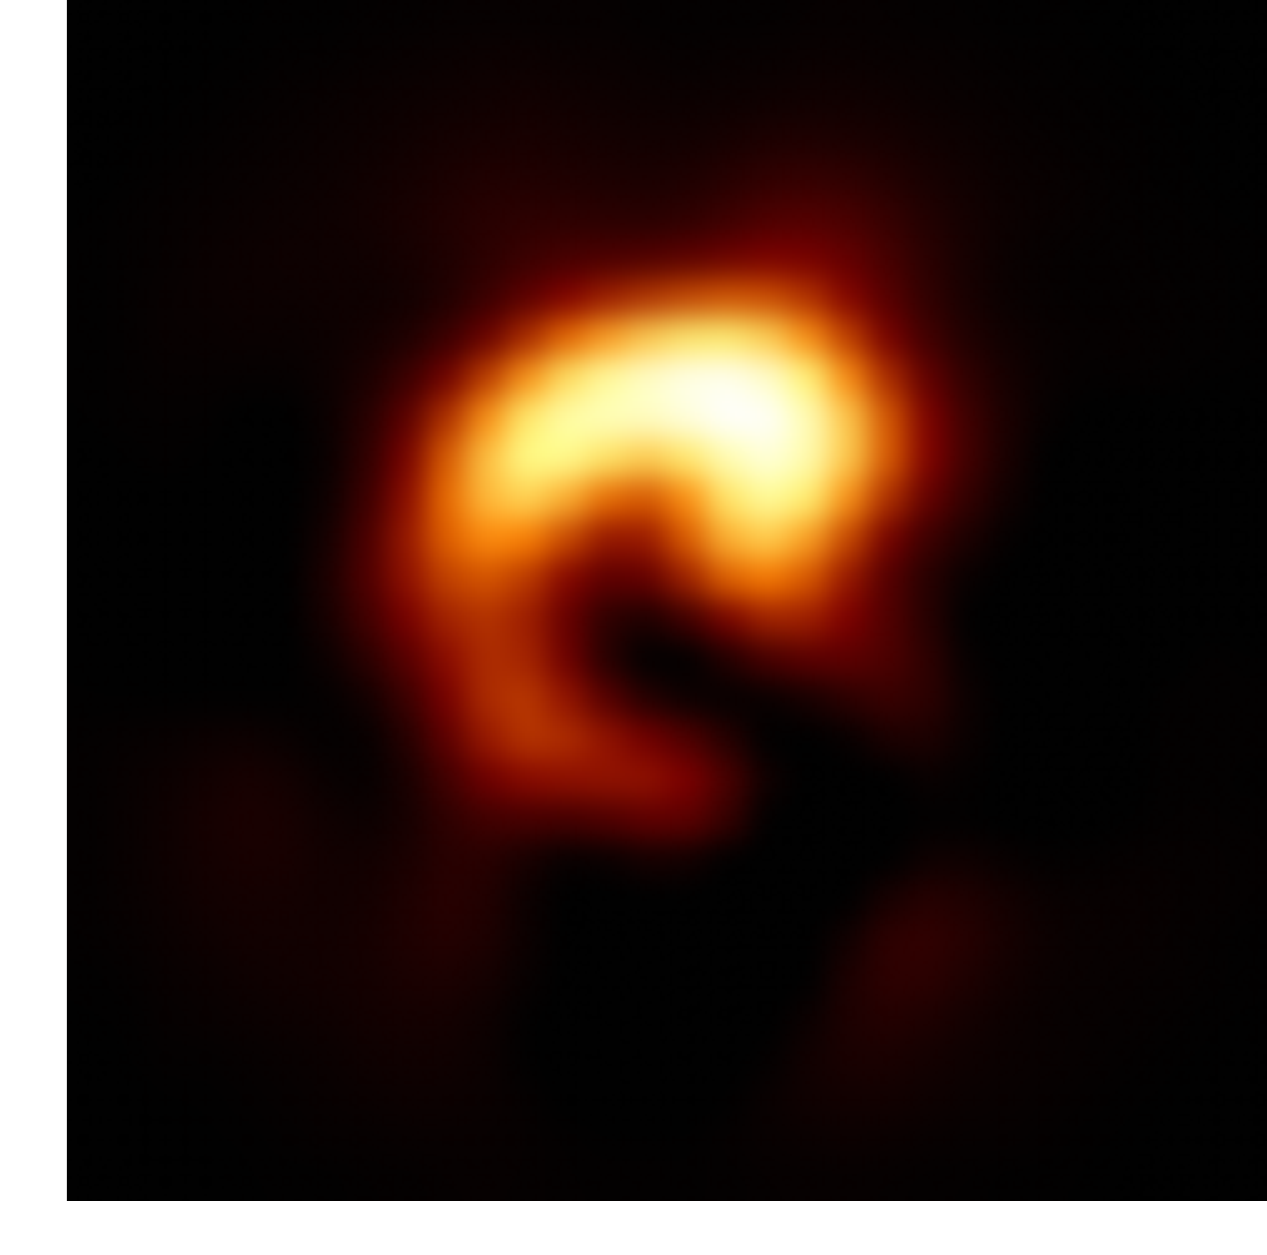} &
			%			\includegraphics[height=0.12\linewidth]{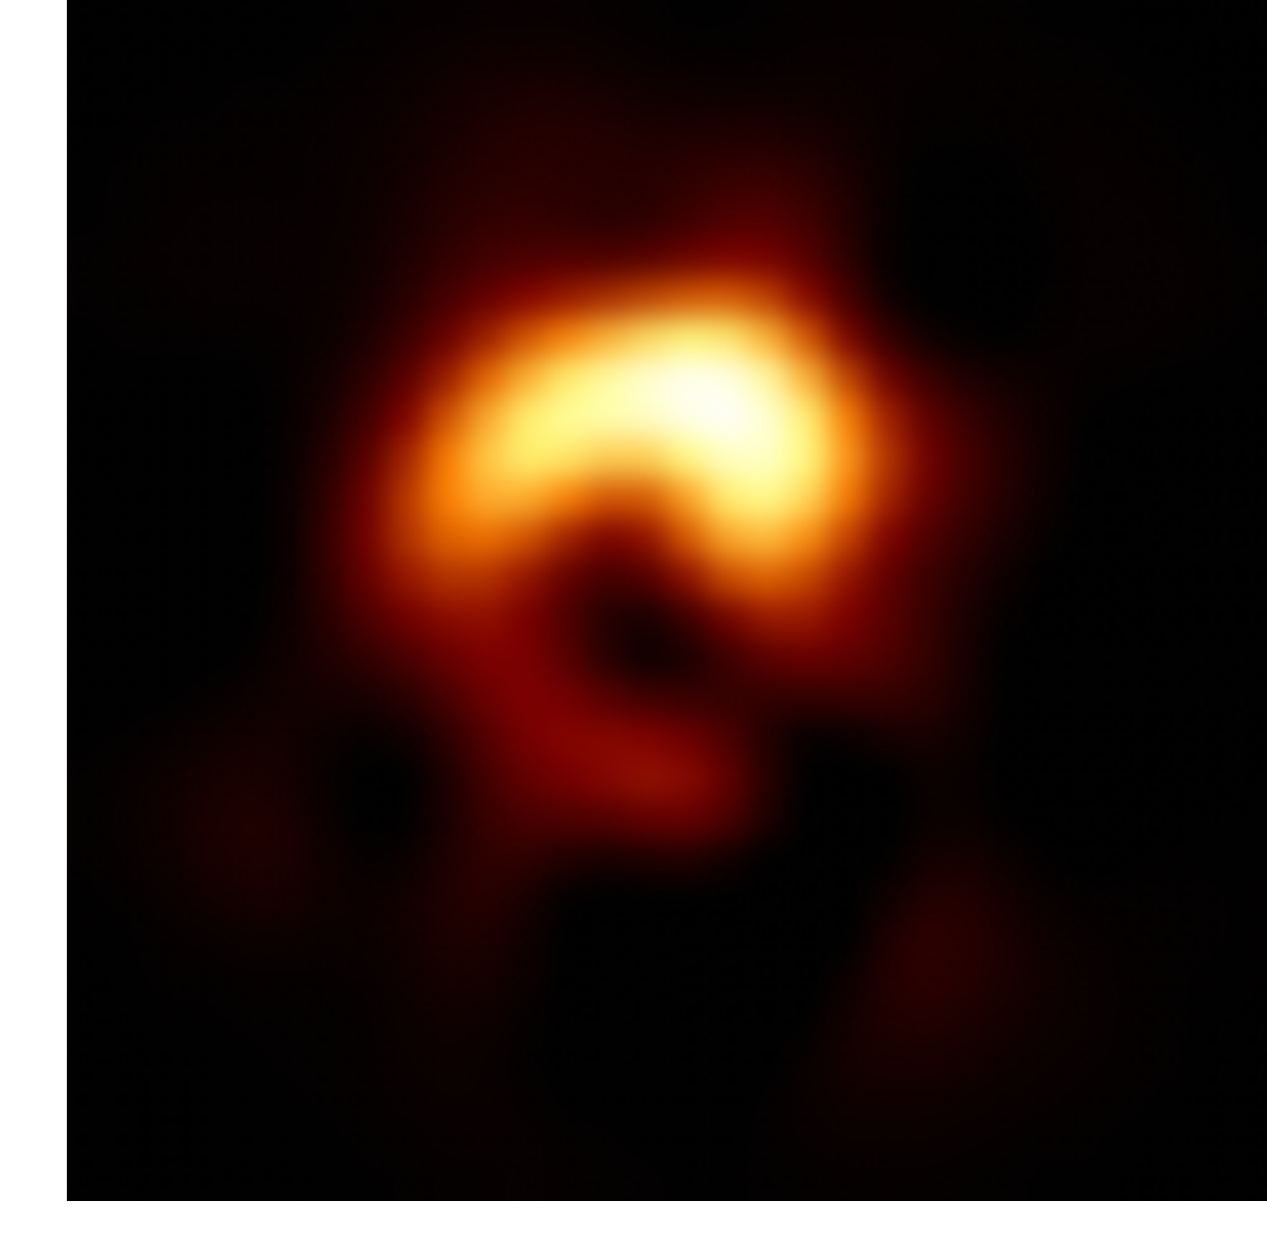} &
			%			\includegraphics[height=0.12\linewidth]{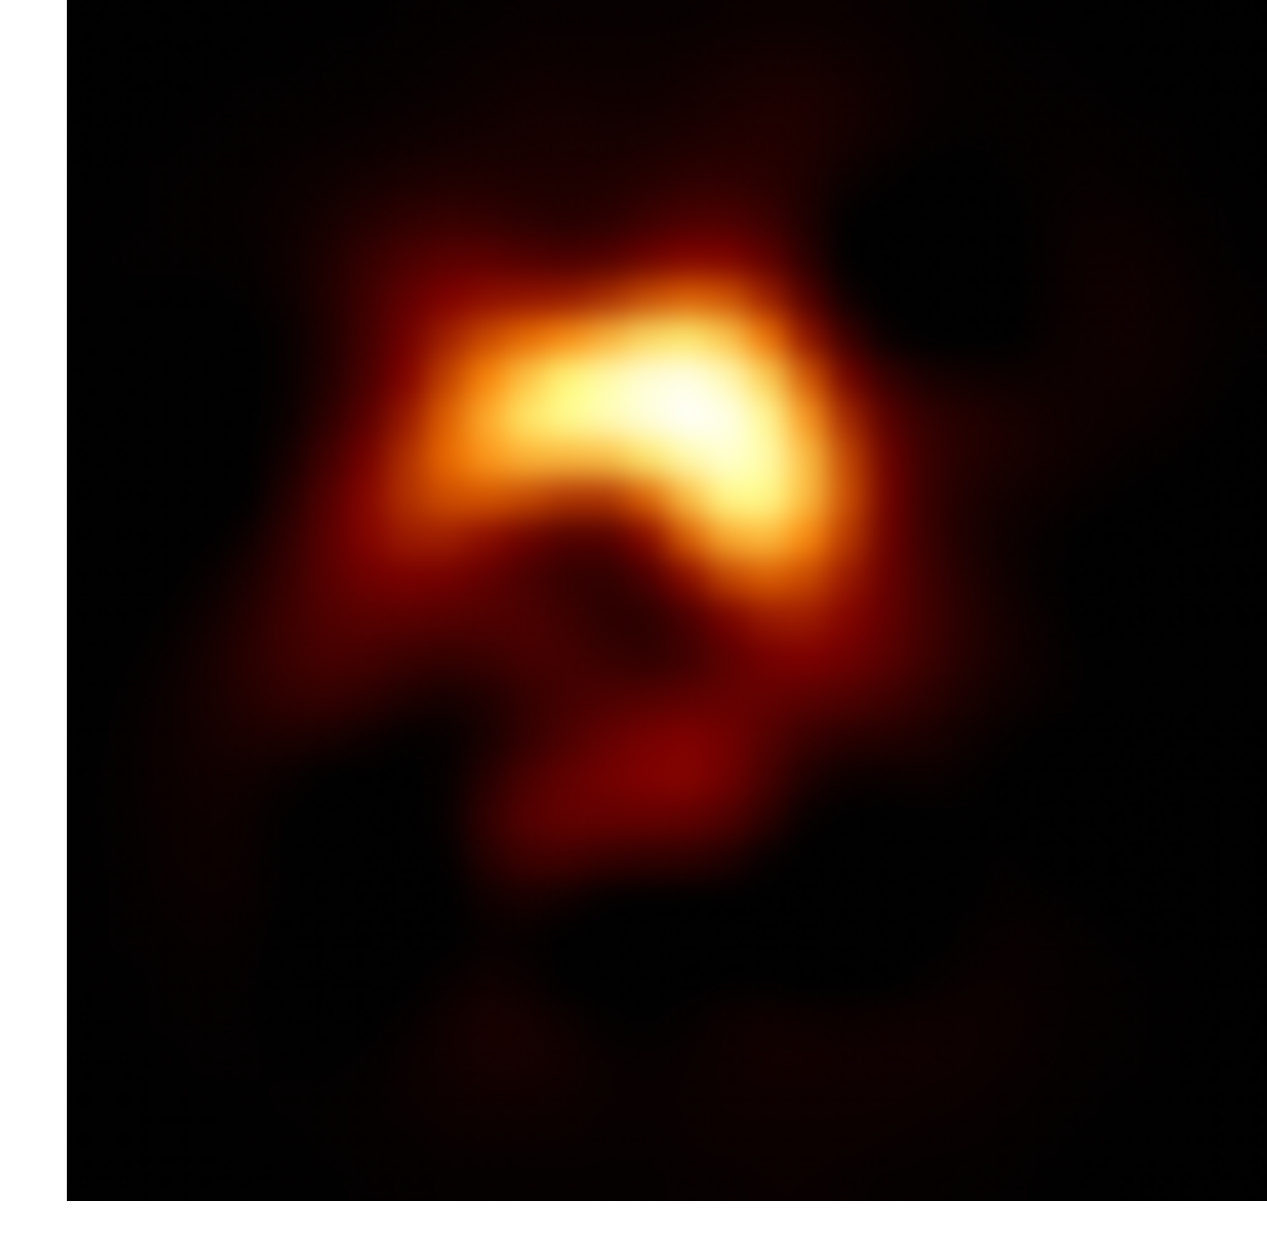} &
			%			\includegraphics[height=0.12\linewidth]{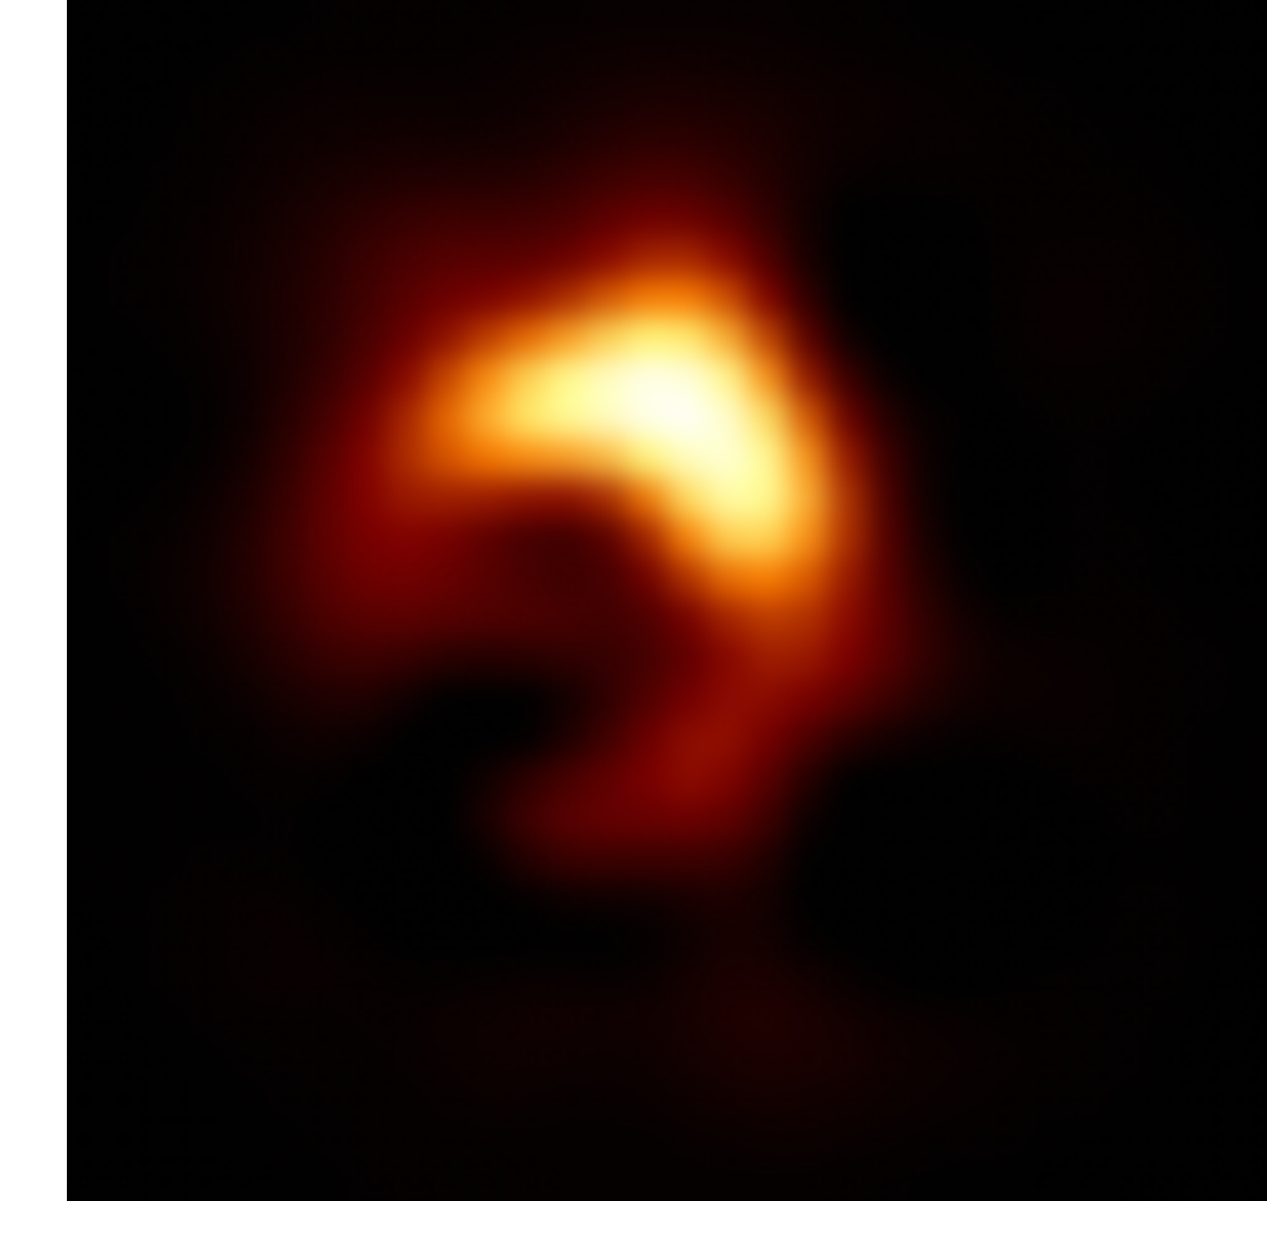} &
			%			\includegraphics[height=0.12\linewidth]{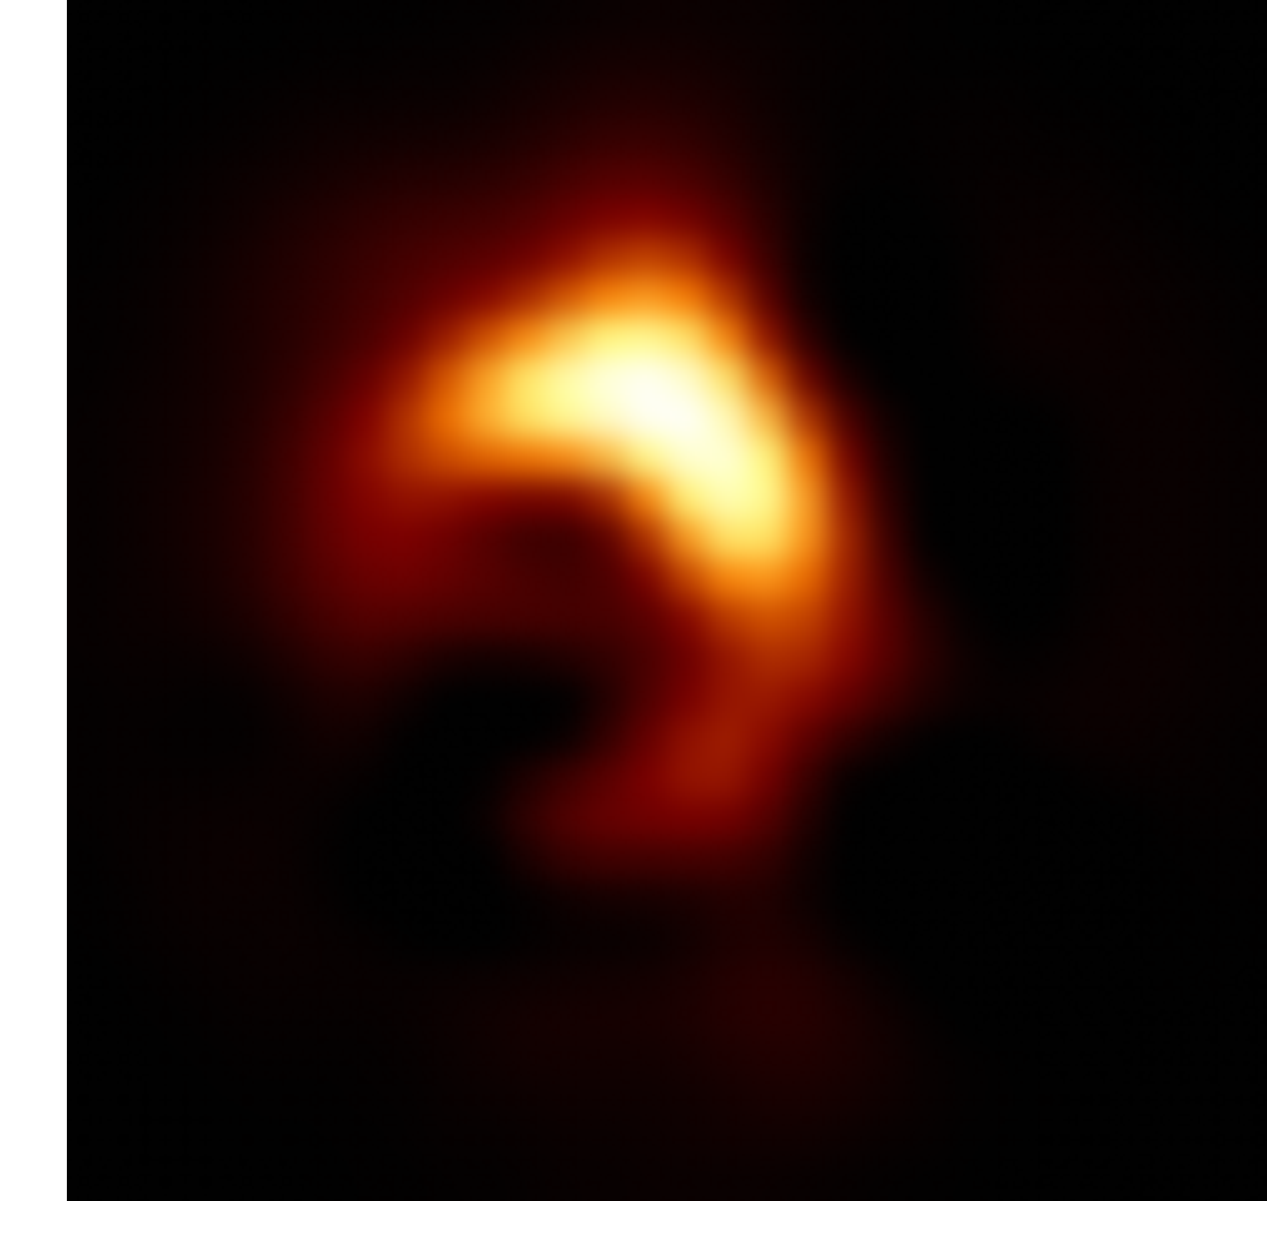}  
			\\ \hline  	
		\end{tabular}
		\caption{ {\footnotesize {\bf Time-resolved reconstruction of Video 1:} Video 1 contains an image rotating clockwise by $180^{\circ}$ over the course of the observation. At each time, the interferometric telescope array measures values related to 2D spatial frequencies of the current underlying image, shown in the row labeled `Truth'. These are indicated by the dots on the uv-coverage plots. As light emitted from the source is real-valued we obtain two values on opposite sides of the frequency plane -- each independent set of measurements displayed as either black or red. We present results obtained when using calibrated data with no atmospheric error, as well as when there is atmospheric phase error still present and we must use data products invariant to its effects.
			Below the true images, we show a subset of images from the baseline 'snapshot imaging' method and compare it to our StarWarps reconstructed video obtained when we assume a static warp field or an inferred warp field. The mean image for each sequence is shown in the leftmost column. In the case that we simultaneously estimate a warp field, we indicate the resulting field as arrows on the mean image. Our method substantially improves results over the snapshot method, especially in the case of atmospheric error when the absolute position of the source cannot be recovered. Additionally, our proposed method can estimate a warp field that gives a sense of the underlying motion of the emission region. This can help to improve results, most notably for the calibrated data with no remaining atmospheric error. } }
		\label{fig:rotation_example1}
	\end{center}
\end{figure*}

\begin{figure*}
	\begin{center}
		\setlength{\tabcolsep}{1pt}
		%\hspace*{-1.5cm}
		\vspace{-0.5cm}
		\begin{tabular}{  c | c | c  c  c  c  c c }
			%\hline
			
			\multirow{1}{*}[0.85in]{ \rotatebox[origin=t]{90}{\large{\textsf{uv-coverage}} }}
			&
			\includegraphics[height=0.12\linewidth]{figures/uvcoverage/uv_ehtfuture2_small.pdf} 
			&
			\includegraphics[height=0.12\linewidth]{figures/uvcoverage/ehtfuture2_173/uv_ehtfuture2_\HSa.pdf} &
			\includegraphics[height=0.12\linewidth]{figures/uvcoverage/ehtfuture2_173/uv_ehtfuture2_\HSb.pdf} &
			\includegraphics[height=0.12\linewidth]{figures/uvcoverage/ehtfuture2_173/uv_ehtfuture2_\HSc.pdf} &
			\includegraphics[height=0.12\linewidth]{figures/uvcoverage/ehtfuture2_173/uv_ehtfuture2_\HSd.pdf} &
			\includegraphics[height=0.12\linewidth]{figures/uvcoverage/ehtfuture2_173/uv_ehtfuture2_\HSe.pdf} &
			\includegraphics[height=0.12\linewidth]{figures/uvcoverage/ehtfuture2_173/uv_ehtfuture2_\HSf.pdf} 
			\\   \hline
			&\vspace{-.1in} &&&&&&\\
			
			&\large{\textsf{Mean Frame}}   &\large{\textsf{GST = 20:10 }} &\large{\textsf{20:20 }}    &\large{\textsf{20:30 }} &\large{\textsf{20:40 }}  &\large{\textsf{20:50 }}  &\large{\textsf{21:00 }}     \\ \hline
			
			&\vspace{-.1in} &&&&&&\\
			\multirow{1}{*}[.6in]{ \rotatebox[origin=t]{90}{\large{\textsf{Truth}} }}
			&
			{{\includegraphics[height=0.12\linewidth]{figures/starwarps_results/hotspot100sR2/gt/pavgimg_noaxis.pdf}} } &
			\includegraphics[height=0.12\linewidth]{figures/starwarps_results/hotspot100sR2/gt/frames/gt_noaxis_\HSa.pdf} &
			\includegraphics[height=0.12\linewidth]{figures/starwarps_results/hotspot100sR2/gt/frames/gt_noaxis_\HSb.pdf} &
			\includegraphics[height=0.12\linewidth]{figures/starwarps_results/hotspot100sR2/gt/frames/gt_noaxis_\HSc.pdf} &
			\includegraphics[height=0.12\linewidth]{figures/starwarps_results/hotspot100sR2/gt/frames/gt_noaxis_\HSd.pdf} &
			\includegraphics[height=0.12\linewidth]{figures/starwarps_results/hotspot100sR2/gt/frames/gt_noaxis_\HSe.pdf} &
			\includegraphics[height=0.12\linewidth]{figures/starwarps_results/hotspot100sR2/gt/frames/gt_noaxis_\HSf.pdf} 
			\\   \hline
			&\vspace{-.1in} &&&&&&\\
			\multicolumn{8}{c}{  \large{\textsf{WITH NO ATMOSPHERIC PHASE ERROR }}  }
			\\ \hline
			&\vspace{-.1in} &&&&&&\\
			\multirow{1}{*}[.6in]{ \rotatebox[origin=t]{90}{\small{\textsf{Snapshot}} }}
			&
			{{\includegraphics[height=0.12\linewidth]{figures/starwarps_results/hotspot100sR2/hotspot100sR2_ehtfuture2_100_snapshot/Reconstructed_Average_Snapshot_vis.pdf}} } &
			\includegraphics[height=0.12\linewidth]{figures/starwarps_results/hotspot100sR2/hotspot100sR2_ehtfuture2_100_snapshot/Reconstructed_Snapshot_vis_\HSa.pdf} &
			\includegraphics[height=0.12\linewidth]{figures/starwarps_results/hotspot100sR2/hotspot100sR2_ehtfuture2_100_snapshot/Reconstructed_Snapshot_vis_\HSb.pdf} &
			\includegraphics[height=0.12\linewidth]{figures/starwarps_results/hotspot100sR2/hotspot100sR2_ehtfuture2_100_snapshot/Reconstructed_Snapshot_vis_\HSc.pdf} &
			\includegraphics[height=0.12\linewidth]{figures/starwarps_results/hotspot100sR2/hotspot100sR2_ehtfuture2_100_snapshot/Reconstructed_Snapshot_vis_\HSd.pdf} &
			\includegraphics[height=0.12\linewidth]{figures/starwarps_results/hotspot100sR2/hotspot100sR2_ehtfuture2_100_snapshot/Reconstructed_Snapshot_vis_\HSe.pdf} &
			\includegraphics[height=0.12\linewidth]{figures/starwarps_results/hotspot100sR2/hotspot100sR2_ehtfuture2_100_snapshot/Reconstructed_Snapshot_vis_\HSf.pdf} 
			\\          
			&\vspace{-.1in} &&&&&&\\
			\multirow{1}{*}[0.7in]{ \rotatebox[origin=t]{90}{  \specialcell{ \small{\textsf{StarWarps:}} \\  \small{\textsf{No Warp}}}  }}
			&
			{{\includegraphics[height=0.12\linewidth]{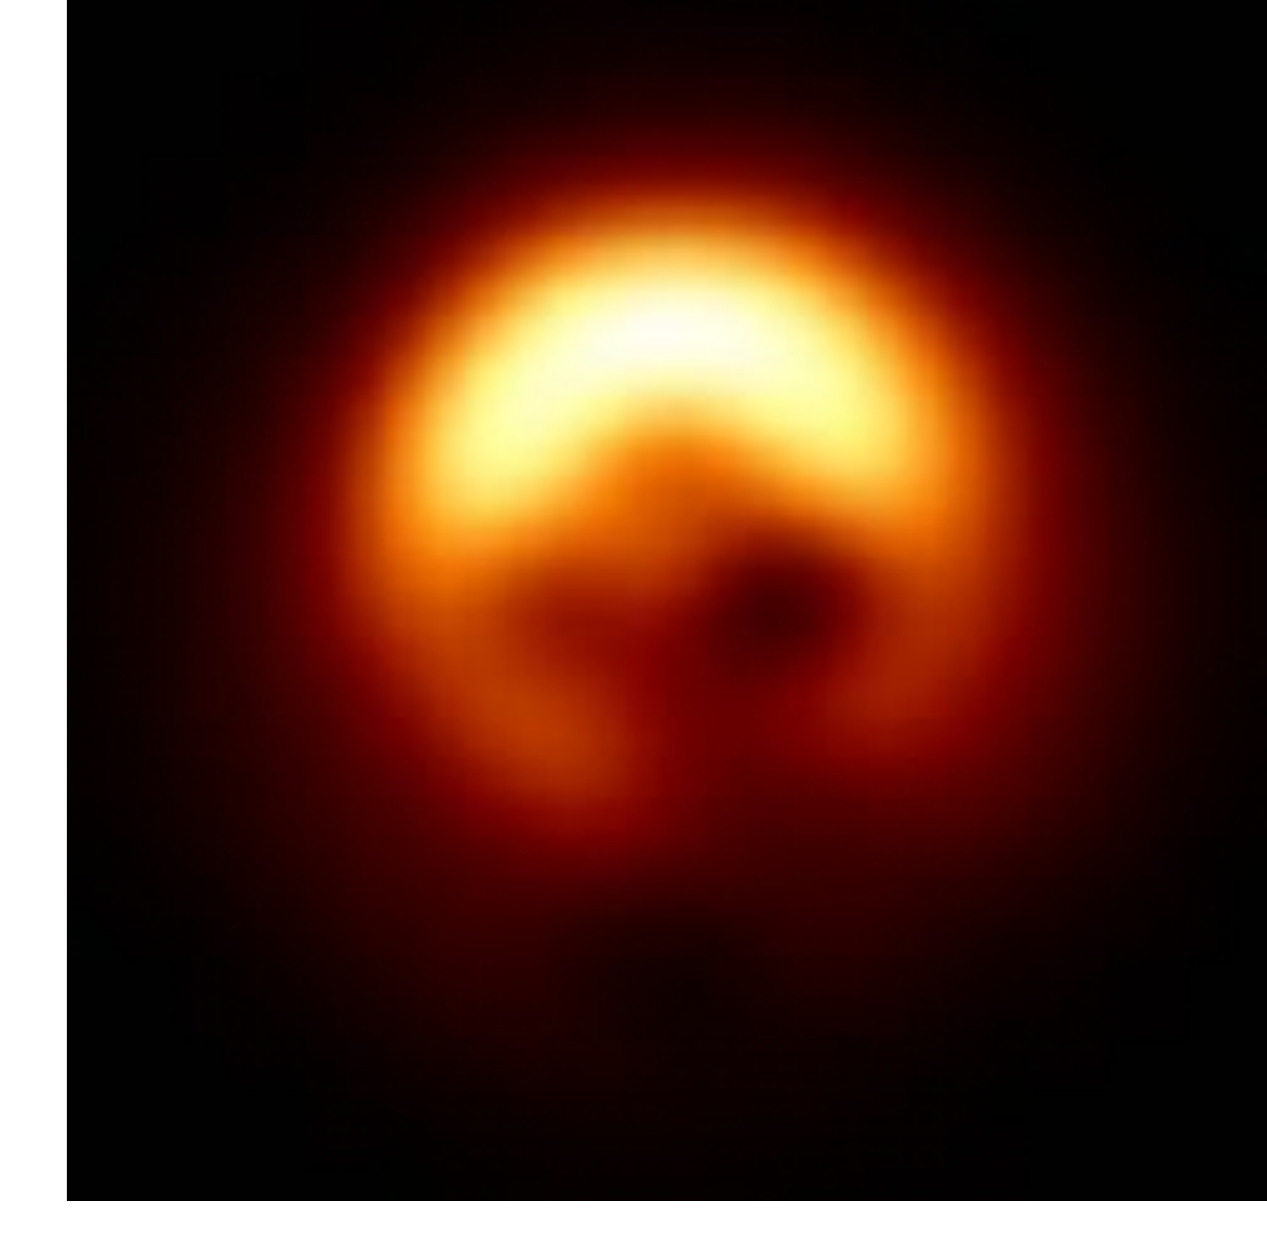}} } &
			\includegraphics[height=0.12\linewidth]{figures/starwarps_results/hotspot100sR2/ehtfuture2_100_visibility/nomotion/frames/mean_noaxis_\HSa.pdf} &
			\includegraphics[height=0.12\linewidth]{figures/starwarps_results/hotspot100sR2/ehtfuture2_100_visibility/nomotion/frames/mean_noaxis_\HSb.pdf} &
			\includegraphics[height=0.12\linewidth]{figures/starwarps_results/hotspot100sR2/ehtfuture2_100_visibility/nomotion/frames/mean_noaxis_\HSc.pdf} &
			\includegraphics[height=0.12\linewidth]{figures/starwarps_results/hotspot100sR2/ehtfuture2_100_visibility/nomotion/frames/mean_noaxis_\HSd.pdf} &
			\includegraphics[height=0.12\linewidth]{figures/starwarps_results/hotspot100sR2/ehtfuture2_100_visibility/nomotion/frames/mean_noaxis_\HSe.pdf} &
			\includegraphics[height=0.12\linewidth]{figures/starwarps_results/hotspot100sR2/ehtfuture2_100_visibility/nomotion/frames/mean_noaxis_\HSf.pdf} 
			\\          
			&\vspace{-.1in} &&&&&&\\
			\multirow{1}{*}[0.7in]{ \rotatebox[origin=t]{90}{  \specialcell{ \small{\textsf{StarWarps:}} \\  \small{\textsf{Learn Warp}}}  }}
			&
			%{{\includegraphics[height=0.12\linewidth]{figures/starwarps_results/hotspot100sR2/ehtfuture2_100_visibility/best/flow_pavg_best_noaxis.pdf}} } 
			%\hspace{0.02in} 
			{{\includegraphics[height=0.12\linewidth]{figures/recov_flowfields/hotspot100sR2_vis/flow_noaxis.pdf}} } &
			\includegraphics[height=0.12\linewidth]{figures/starwarps_results/hotspot100sR2/ehtfuture2_100_visibility/best/frames/mean_noaxis_\HSa.pdf} &
			\includegraphics[height=0.12\linewidth]{figures/starwarps_results/hotspot100sR2/ehtfuture2_100_visibility/best/frames/mean_noaxis_\HSb.pdf} &
			\includegraphics[height=0.12\linewidth]{figures/starwarps_results/hotspot100sR2/ehtfuture2_100_visibility/best/frames/mean_noaxis_\HSc.pdf} &
			\includegraphics[height=0.12\linewidth]{figures/starwarps_results/hotspot100sR2/ehtfuture2_100_visibility/best/frames/mean_noaxis_\HSd.pdf} &
			\includegraphics[height=0.12\linewidth]{figures/starwarps_results/hotspot100sR2/ehtfuture2_100_visibility/best/frames/mean_noaxis_\HSe.pdf} &
			\includegraphics[height=0.12\linewidth]{figures/starwarps_results/hotspot100sR2/ehtfuture2_100_visibility/best/frames/mean_noaxis_\HSf.pdf} 
			\\ \hline  	
			&\vspace{-.1in} &&&&&&\\
			\multicolumn{8}{c}{  \large{\textsf{WITH ATMOSPHERIC PHASE ERROR }}  }
			\\ \hline
			&\vspace{-.1in} &&&&&&\\
			\multirow{1}{*}[.6in]{ \rotatebox[origin=t]{90}{\small{\textsf{Snapshot}} }}
			&
			{{\includegraphics[height=0.12\linewidth]{figures/starwarps_results/hotspot100sR2/hotspot100sR2_ehtfuture2_100_snapshot/Reconstructed_Average_Snapshot_AmpCphase.pdf}} } &
			\includegraphics[height=0.12\linewidth]{figures/starwarps_results/hotspot100sR2/hotspot100sR2_ehtfuture2_100_snapshot/Reconstructed_Snapshot_AmpCphase_\HSa.pdf} &
			\includegraphics[height=0.12\linewidth]{figures/starwarps_results/hotspot100sR2/hotspot100sR2_ehtfuture2_100_snapshot/Reconstructed_Snapshot_AmpCphase_\HSb.pdf} &
			\includegraphics[height=0.12\linewidth]{figures/starwarps_results/hotspot100sR2/hotspot100sR2_ehtfuture2_100_snapshot/Reconstructed_Snapshot_AmpCphase_\HSc.pdf} &
			\includegraphics[height=0.12\linewidth]{figures/starwarps_results/hotspot100sR2/hotspot100sR2_ehtfuture2_100_snapshot/Reconstructed_Snapshot_AmpCphase_\HSd.pdf} &
			\includegraphics[height=0.12\linewidth]{figures/starwarps_results/hotspot100sR2/hotspot100sR2_ehtfuture2_100_snapshot/Reconstructed_Snapshot_AmpCphase_\HSe.pdf} &
			\includegraphics[height=0.12\linewidth]{figures/starwarps_results/hotspot100sR2/hotspot100sR2_ehtfuture2_100_snapshot/Reconstructed_Snapshot_AmpCphase_\HSf.pdf}  \\
			&\vspace{-.1in} &&&&&&\\
			\multirow{1}{*}[0.7in]{ \rotatebox[origin=t]{90}{  \specialcell{ \small{\textsf{StarWarps:}} \\  \small{\textsf{No Warp}}}  }}
			&
			{{\includegraphics[height=0.12\linewidth]{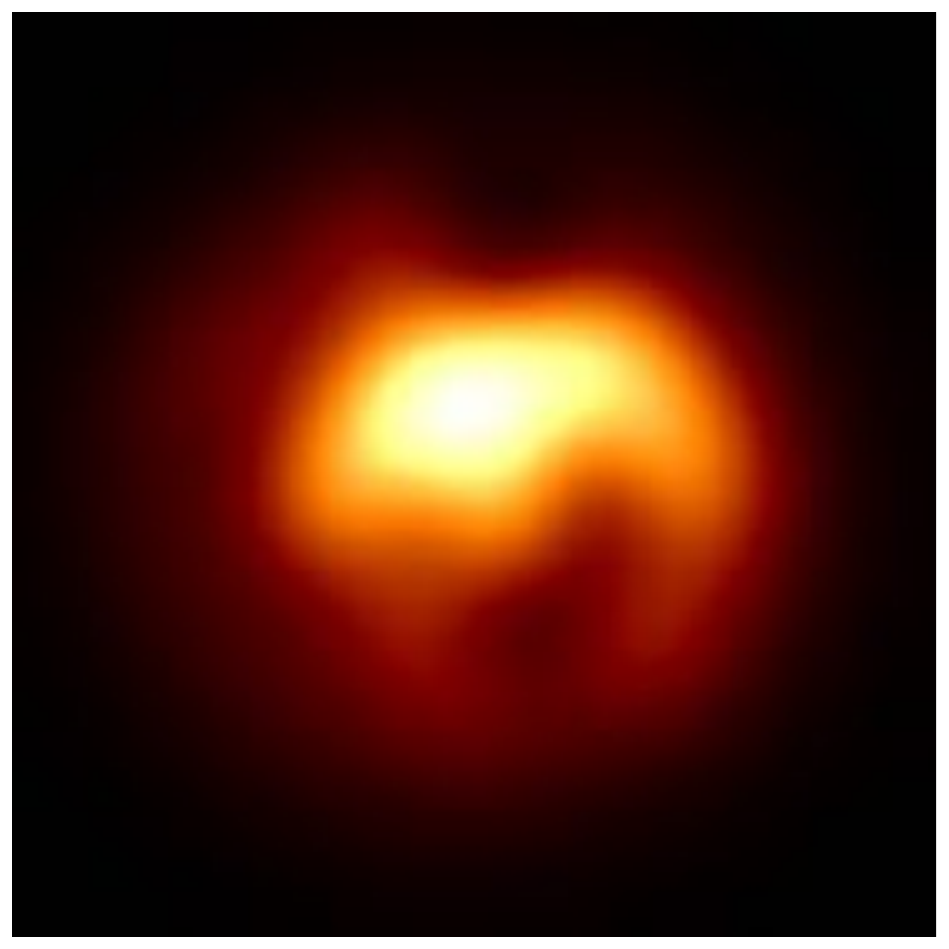}} } &
			\includegraphics[height=0.12\linewidth]{figures/starwarps_results/hotspot100sR2/ehtfuture2_100_amp-bispectrum/nomotion/frames/mean_noaxis_\HSa.pdf} &
			\includegraphics[height=0.12\linewidth]{figures/starwarps_results/hotspot100sR2/ehtfuture2_100_amp-bispectrum/nomotion/frames/mean_noaxis_\HSb.pdf} &
			\includegraphics[height=0.12\linewidth]{figures/starwarps_results/hotspot100sR2/ehtfuture2_100_amp-bispectrum/nomotion/frames/mean_noaxis_\HSc.pdf} &
			\includegraphics[height=0.12\linewidth]{figures/starwarps_results/hotspot100sR2/ehtfuture2_100_amp-bispectrum/nomotion/frames/mean_noaxis_\HSd.pdf} &
			\includegraphics[height=0.12\linewidth]{figures/starwarps_results/hotspot100sR2/ehtfuture2_100_amp-bispectrum/nomotion/frames/mean_noaxis_\HSe.pdf} &
			\includegraphics[height=0.12\linewidth]{figures/starwarps_results/hotspot100sR2/ehtfuture2_100_amp-bispectrum/nomotion/frames/mean_noaxis_\HSf.pdf} 
			\\          
			&\vspace{-.1in} &&&&&&\\
			\multirow{1}{*}[0.7in]{ \rotatebox[origin=t]{90}{  \specialcell{ \small{\textsf{StarWarps:}} \\  \small{\textsf{Learn Warp}}}  }}
			&
			%{{\includegraphics[height=0.12\linewidth]{figures/starwarps_results/hotspot100sR2/ehtfuture2_100_amp-bispectrum/best/flow_pavg_best_noaxis.pdf}} }
			%\hspace{0.02in} 
			{{\includegraphics[height=0.12\linewidth]{figures/recov_flowfields/hotspot100sR2_bis/flow_noaxis.pdf}} } &
			\includegraphics[height=0.12\linewidth]{figures/starwarps_results/hotspot100sR2/ehtfuture2_100_amp-bispectrum/best/frames/mean_noaxis_49.pdf} &
			\includegraphics[height=0.12\linewidth]{figures/starwarps_results/hotspot100sR2/ehtfuture2_100_amp-bispectrum/best/frames/mean_noaxis_59.pdf} &
			\includegraphics[height=0.12\linewidth]{figures/starwarps_results/hotspot100sR2/ehtfuture2_100_amp-bispectrum/best/frames/mean_noaxis_69.pdf} &
			\includegraphics[height=0.12\linewidth]{figures/starwarps_results/hotspot100sR2/ehtfuture2_100_amp-bispectrum/best/frames/mean_noaxis_79.pdf} &
			\includegraphics[height=0.12\linewidth]{figures/starwarps_results/hotspot100sR2/ehtfuture2_100_amp-bispectrum/best/frames/mean_noaxis_89.pdf} &
			\includegraphics[height=0.12\linewidth]{figures/starwarps_results/hotspot100sR2/ehtfuture2_100_amp-bispectrum/best/frames/mean_noaxis_90.pdf}  
			\\ \hline  	
		\end{tabular}
		\caption{ {\footnotesize {\bf Time-resolved reconstruction of Video 2:} Video 2 contains a sequence of a hotspot orbiting counter-clockwise around a black hole. We present time-resolved results obtained using data derived from this sequence. 
			Below the true images, we show a subset of images from the baseline 'snapshot imaging' method and compare it to our StarWarps reconstructed video obtained assuming a static warp field or an inferred warp field. The mean image for each sequence is shown in the leftmost column. If we simultaneously estimate a warp field, we indicate the resulting field as arrows on the mean image. 
			Our method substantially improve results over the snapshot method, especially in the case of atmospheric error when the absolute position of the source cannot be recovered. 
			Additionally, despite the fact that this hotspot video does not match our assumed motion model, using our proposed approach we were able to estimate a warp field that provides the direction of the source's true underlying motion. See the caption of Figure~\ref{fig:rotation_example1} for more detail. } }
		\label{fig:rotation_example2}
	\end{center}
\end{figure*}
