# Supplementary material for: Reconstructing Video from Interferometric Measurements of Time-Varying Sources
Source: arXiv:1711.01357 source file (2018-02-01)
Supplement: Supplementary file 2 [file appendix.tex]

\clearpage
\clearpage
\begin{center}
\begin{minipage}[c]{\textwidth}

\section{Appendix}

\subsection{Lemma} Product of Gaussians 2
\label{lemma:woodburrymatrixreduce}

\begin{align}
\mathcal{N}_{x} ({\bf A}^{-1}  y , ( {\bf A}^T  \Sigma^{-1} {\bf A} )^{-1} ) \mathcal{N}_{x} ( \mu , Q ) \propto \mathcal{N}_{x} ( m, C ) 
\end{align}

where from the Matrix Cookbook (8.1.8) and the Woodbury matrix identity we know that 

\begin{align}
 C_t & = ( {\bf A}^T  \Sigma^{-1} {\bf A} + Q^{-1} )^{-1}   \\
 & = Q - Q{\bf A}^T ( \Sigma + {\bf A} Q {\bf A}^T )^{-1} {\bf A} Q \\
 m_t & = C_t ( {\bf A}^T  \Sigma^{-1} {\bf A} {\bf A}^{-1}  y +  Q^{-1} \mu ) \\
 & = (Q - Q{\bf A}^T ( \Sigma + {\bf A} Q {\bf A}^T )^{-1} {\bf A} Q ) ( {\bf A}^T  \Sigma^{-1} y +  Q^{-1} \mu ) \\
 & = Q{\bf A}^T  \Sigma^{-1} y + Q Q^{-1} \mu  - Q{\bf A}^T ( \Sigma + {\bf A} Q {\bf A}^T )^{-1} {\bf A} Q  {\bf A}^T  \Sigma^{-1} y -   Q{\bf A}^T ( \Sigma + {\bf A} Q {\bf A}^T )^{-1} {\bf A} Q Q^{-1} \mu ) \\
 & =  \mu  + Q{\bf A}^T  \Sigma^{-1} y - Q{\bf A}^T ( \Sigma + {\bf A} Q {\bf A}^T )^{-1} {\bf A} Q  {\bf A}^T  \Sigma^{-1} y -   Q{\bf A}^T ( \Sigma + {\bf A} Q {\bf A}^T )^{-1} {\bf A} \mu ) \\
 & =  \mu  + Q{\bf A}^T ( \Sigma + {\bf A} Q {\bf A}^T )^{-1} ( ( \Sigma + {\bf A} Q {\bf A}^T ) \Sigma^{-1} y -  {\bf A} Q  {\bf A}^T  \Sigma^{-1} y -  {\bf A} \mu ) \\
& =  \mu  + Q{\bf A}^T ( \Sigma + {\bf A} Q {\bf A}^T )^{-1} (  y -  {\bf A} \mu ) 
\end{align}

\end{minipage}
\end{center}
